# Supplementary material for: Model-based Clustering of Multi-Dimensional Zero-Inflated Counts via the EM Algorithm
Source: arXiv:2406.00245 ancillary file (2025-03-27)
Supplement: Supplementary file 1 [file Supplementary_Material.pdf]

# Model-based Clustering of Zero-Inflated Single-Cell RNA Sequencing Data via the EM Algorithm

## Supplementary Material

Zahra AghahosseinaliShirazi<sup>a1\*</sup>, Pedro A. Rangel<sup>a2†</sup> and Camila P. E. de Souza<sup>a3‡</sup>

<sup>a</sup> The University of Western Ontario, ON, Canada

May 31, 2024

### Contents

|          |                                                                           |          |
|----------|---------------------------------------------------------------------------|----------|
| <b>1</b> | <b>Simulation studies</b>                                                 | <b>3</b> |
| 1.1      | Computer and software specifications . . . . .                            | 3        |
| 1.2      | V-measure . . . . .                                                       | 3        |
| 1.3      | Simulation results for the ZIP mixture model without covariates . . . . . | 4        |
| 1.3.1    | Scenario 1 . . . . .                                                      | 4        |
| 1.3.2    | Scenario 2 . . . . .                                                      | 8        |
| 1.3.3    | Scenario 3 . . . . .                                                      | 11       |
| 1.3.4    | Scenario 4 . . . . .                                                      | 15       |
| 1.3.5    | Scenario 5 . . . . .                                                      | 19       |
| 1.3.6    | Scenario 6 . . . . .                                                      | 23       |
| 1.4      | Simulation results for the ZIP mixture model with a size factor . . . . . | 28       |
| 1.4.1    | Scenario 1 . . . . .                                                      | 28       |
| 1.4.2    | Scenario 2 . . . . .                                                      | 31       |
| 1.4.3    | Scenario 3 . . . . .                                                      | 34       |
| 1.4.4    | Scenario 4 . . . . .                                                      | 38       |
| 1.4.5    | Scenario 5 . . . . .                                                      | 42       |
| 1.4.6    | Scenario 6 . . . . .                                                      | 46       |
| 1.5      | Simulation results for the ZIP mixture model with a covariate . . . . .   | 51       |
| 1.5.1    | Scenario 1 . . . . .                                                      | 51       |
| 1.5.2    | Scenario 2 . . . . .                                                      | 55       |
| 1.6      | Simulation results for the Mixture of ZINB without covariates . . . . .   | 59       |
| 1.6.1    | Scenario 1 . . . . .                                                      | 59       |
| 1.6.2    | Scenario 2 . . . . .                                                      | 61       |

---

<sup>\*1</sup> Email: zagahos@uwo.ca

<sup>†2</sup> Email: pedroar.est@gmail.com

<sup>‡3</sup> Email: camila.souza@uwo.ca

|          |                                                                         |           |
|----------|-------------------------------------------------------------------------|-----------|
| 1.7      | Simulation results for the mixture of ZINB with a size factor . . . . . | 64        |
| 1.7.1    | Scenario 1 . . . . .                                                    | 64        |
| <b>2</b> | <b>Data analyses</b>                                                    | <b>66</b> |
| 2.1      | Mouse Embryonic Stem Cell (MESC) data . . . . .                         | 66        |
| 2.2      | Liver Data . . . . .                                                    | 76        |
|          | <b>Bibliography</b>                                                     | <b>87</b> |

# 1 Simulation studies

## 1.1 Computer and software specifications

The simulations for the ZIP mixture model without covariates and the ZIP mixture model with a size factor (i.e., with only  $\beta_{0g}$  and  $\rho_{gk}$ ) were performed using Sharcnet's Graham computer cluster via the Digital Research Alliance of Canada, with a single node consisting of two Intel E5-2683 V4 (Broadwell) with 2.1 GHZ, for an overall of 32 computing cores. The number of available cores informs the decision to choose  $S = 256$  simulated datasets, a multiple of the number of cores. The computations were performed on redCent OS 7, with R version 4.1.2 (R core Team, 2021), using the packages *Parallel* to simulate and to compute the EM algorithm of independent datasets simultaneously, the *FDRSEG* (Hi et al. (2017)) package to calculate the V-measure. Simulations for the ZINB case were performed on ASUSTEK ZenBook UX535LI, Intel Core i7-10750H @2.60 GHZ with R version 4.2.2, for the case without covariates. We simulated  $S = 100$  datasets for each scenario and similar to the mixture of ZIP cases, the library *FDRSEG* was used for calculating V-measures.

## 1.2 V-measure

The V-measure (Rosenberg and Hirschberg, 2007) is a metric to assess how well a set of clusters  $K = k_1, \dots, k_m$  partition a set of  $N$  observations knowing the fact that they belong to a set of classes  $C = c_1, \dots, c_n$ . This is an entropy-based metric to evaluate the performance of the clustering using the criteria of homogeneity and completeness. The homogeneity represents how similar the elements of the clusters are to the other elements of the same cluster, as measured by:

$$h = \begin{cases} 1 & \text{if } H(C, K) = 0 \\ 1 - \frac{H(C|K)}{H(C)} & \text{otherwise,} \end{cases}$$

where

$$H(C|K) = - \sum_{k=1}^{|K|} \sum_{c=1}^{|C|} \frac{a_{ck}}{N} \log \left( \frac{a_{ck}}{\sum_{c=1}^{|C|} a_{ck}} \right), \text{ and}$$

$$H(C) = - \sum_{c=1}^{|C|} \frac{\sum_{k=1}^{|K|} a_{ck}}{n} \log \left( \frac{\sum_{k=1}^{|K|} a_{ck}}{n} \right),$$

with  $a_{ck}$  as the number of observations from class  $c$  assigned to cluster  $k$ . The completeness represents how close the elements of the same class are clustered together, and is measured by:

$$c = \begin{cases} 1 & \text{if } H(K, C) = 0 \\ 1 - \frac{H(K|C)}{H(K)} & \text{otherwise,} \end{cases}$$

where

$$H(K|C) = - \sum_{c=1}^{|C|} \sum_{k=1}^{|K|} \frac{a_{ck}}{N} \log \left( \frac{a_{ck}}{\sum_{k=1}^{|K|} a_{ck}} \right), \text{ and}$$

$$H(K) = - \sum_{k=1}^{|K|} \frac{\sum_{c=1}^{|C|} a_{ck}}{n} \log \left( \frac{\sum_{c=1}^{|C|} a_{ck}}{n} \right).$$

With these two measures,  $h$  and  $c$ , the overall V-measure is obtained as follows:

$$V_\beta = \frac{(1 + \beta) \times h \times c}{(\beta \times h) + c},$$

where we use the default  $\beta = 1$  in our calculations.

### 1.3 Simulation results for the ZIP mixture model without covariates

#### 1.3.1 Scenario 1

**Table 1: Scenario 1:** Mean and standard deviation (SD) for the estimates of  $\phi_k$  obtained for each  $k$  and each  $N$  using the EM algorithm across the simulated datasets.

| $k$ | $N$  | Mean    | SD      |
|-----|------|---------|---------|
| 1   | 12   | 0.09052 | 0.02572 |
|     | 60   | 0.10002 | 0.00581 |
|     | 120  | 0.09998 | 0.00414 |
|     | 600  | 0.09990 | 0.00190 |
|     | 1200 | 0.09994 | 0.00136 |
| 2   | 12   | 0.08971 | 0.02448 |
|     | 60   | 0.09949 | 0.00608 |
|     | 120  | 0.09966 | 0.00432 |
|     | 600  | 0.10004 | 0.00188 |
|     | 1200 | 0.10003 | 0.00132 |
| 3   | 12   | 0.09242 | 0.02372 |
|     | 60   | 0.10024 | 0.00616 |
|     | 120  | 0.09989 | 0.00464 |
|     | 600  | 0.10015 | 0.00194 |
|     | 1200 | 0.10012 | 0.00155 |

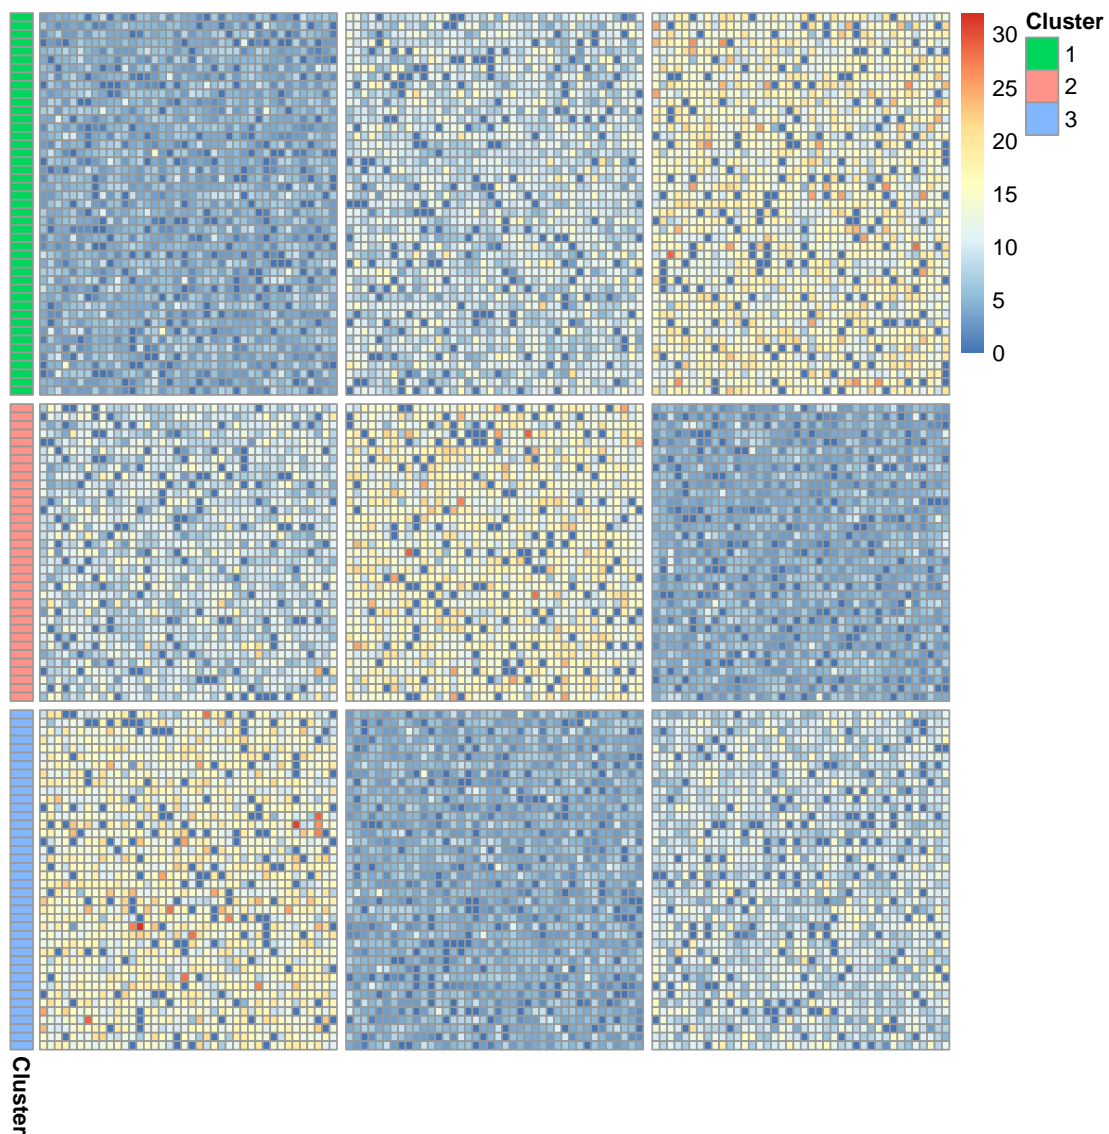

**Figure 1: Scenario 1:** Heatmap of a simulated data set generated according to the settings in Case 3 of Table 1 of paper Darker colors represent higher counts. The assigned true clusters at the simulation stage are represented by the colored column on the left side of the plot.

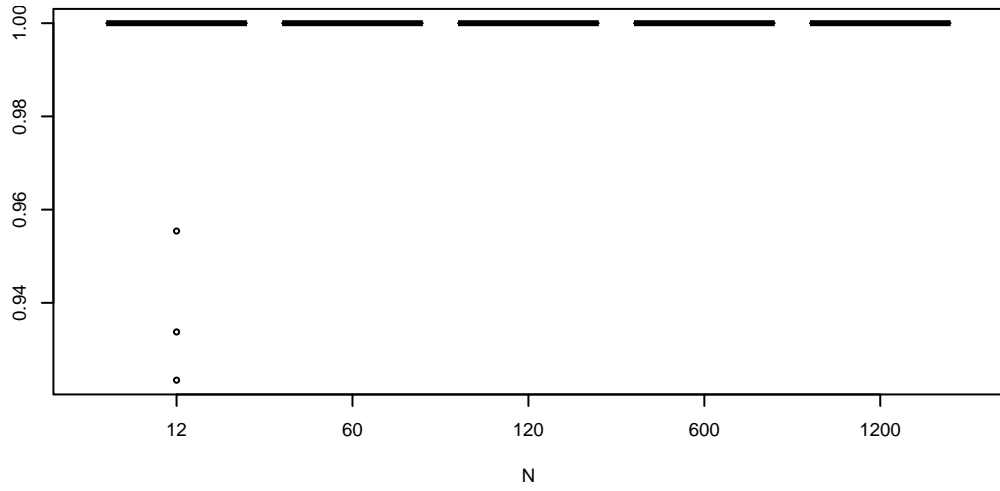

**Figure 2: Scenario 1:** Boxplots of the V-measures comparing the EM clustering assignments with true cluster labels, across the simulated datasets.

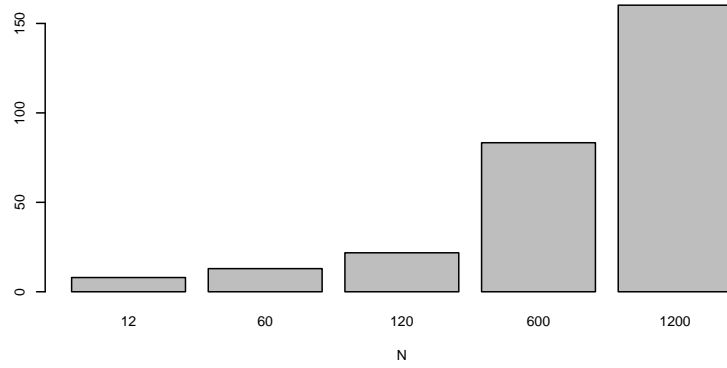

**Figure 3: Scenario 1:** Bar plot for the total computing times, in seconds, taken for the EM algorithm to converge across the simulated datasets. See also Table 3.

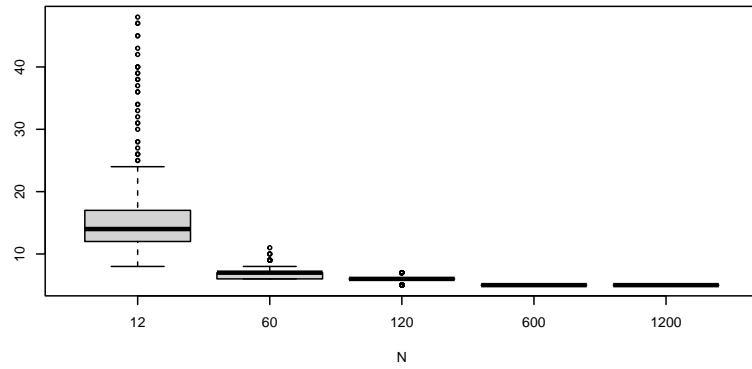

**Figure 4: Scenario 1:** Boxplots for the number of iterations until the EM algorithm converged across the simulated datasets. See also Table 4.

**Table 2: Scenario 1:** Mean and standard deviation (SD) for the estimates of  $\pi_k$  obtained for each  $k$  and each  $N$  using the EM algorithm across the simulated datasets.

| $k$ | $N$  | Mean    | SD      |
|-----|------|---------|---------|
| 1   | 12   | 0.33431 | 0.13777 |
|     | 60   | 0.32689 | 0.05793 |
|     | 120  | 0.33385 | 0.04303 |
|     | 600  | 0.33447 | 0.01805 |
|     | 1200 | 0.33274 | 0.01361 |
| 2   | 12   | 0.34017 | 0.13359 |
|     | 60   | 0.33906 | 0.06123 |
|     | 120  | 0.33815 | 0.04353 |
|     | 600  | 0.33371 | 0.01862 |
|     | 1200 | 0.33420 | 0.01334 |
| 3   | 12   | 0.32552 | 0.13445 |
|     | 60   | 0.33405 | 0.06115 |
|     | 120  | 0.32799 | 0.04730 |
|     | 600  | 0.33182 | 0.01967 |
|     | 1200 | 0.33306 | 0.01287 |

**Table 3: Scenario 1:** Mean and standard deviation (SD) for the EM algorithm computing times, in seconds, by  $N$ , across the simulated datasets.

| $N$  | Mean    | SD      |
|------|---------|---------|
| 12   | 0.03111 | 0.01597 |
| 60   | 0.05055 | 0.01114 |
| 120  | 0.08514 | 0.01712 |
| 600  | 0.32546 | 0.03525 |
| 1200 | 0.62588 | 0.03852 |

**Table 4: Scenario 1:** Mean and standard deviation (SD) for the number of iterations until the EM algorithm converged, by  $N$ , across the simulated datasets.

| $N$  | Mean     | SD      |
|------|----------|---------|
| 12   | 16.78125 | 8.02588 |
| 60   | 6.84766  | 0.91407 |
| 120  | 5.96094  | 0.41354 |
| 600  | 5.00000  | 0.00000 |
| 1200 | 5.00000  | 0.00000 |

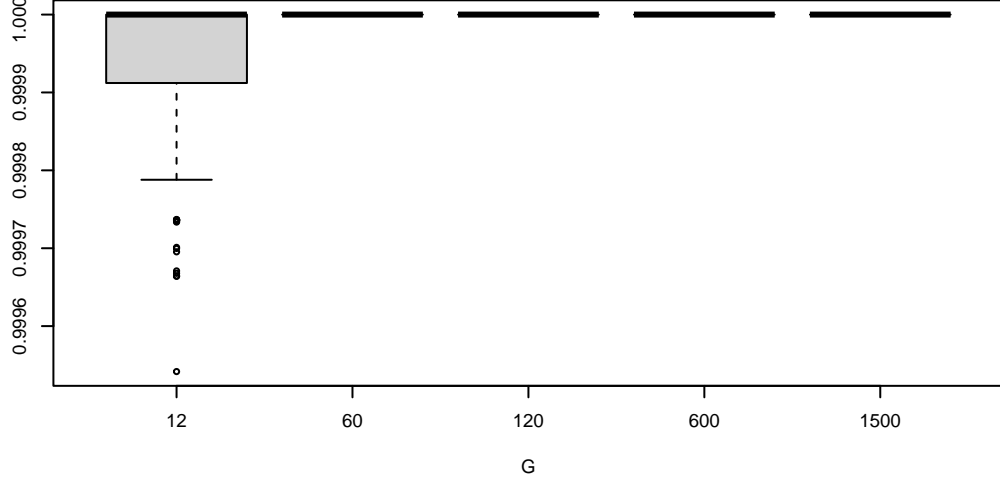

**Figure 5: Scenario 2:** Boxplots for the  $V$ -measures comparing the EM clustering assignments with true cluster labels, across the simulated datasets.

### 1.3.2 Scenario 2

**Table 5: Scenario 2:** Mean and standard deviation (SD) for the estimates of  $\phi_k$  obtained for each  $k$  and each  $G$  using the EM algorithm across the simulated datasets.

| $k$ | $G$  | Mean    | SD      |
|-----|------|---------|---------|
| 1   | 12   | 0.09992 | 0.00450 |
|     | 60   | 0.09966 | 0.00195 |
|     | 120  | 0.09998 | 0.00133 |
|     | 600  | 0.10007 | 0.00063 |
|     | 1500 | 0.09993 | 0.00036 |
| 2   | 12   | 0.09997 | 0.00437 |
|     | 60   | 0.10018 | 0.00206 |
|     | 120  | 0.09985 | 0.00142 |
|     | 600  | 0.10000 | 0.00056 |
|     | 1500 | 0.09999 | 0.00038 |
| 3   | 12   | 0.10050 | 0.00459 |
|     | 60   | 0.09977 | 0.00198 |
|     | 120  | 0.09995 | 0.00133 |
|     | 600  | 0.09998 | 0.00066 |
|     | 1500 | 0.09998 | 0.00042 |

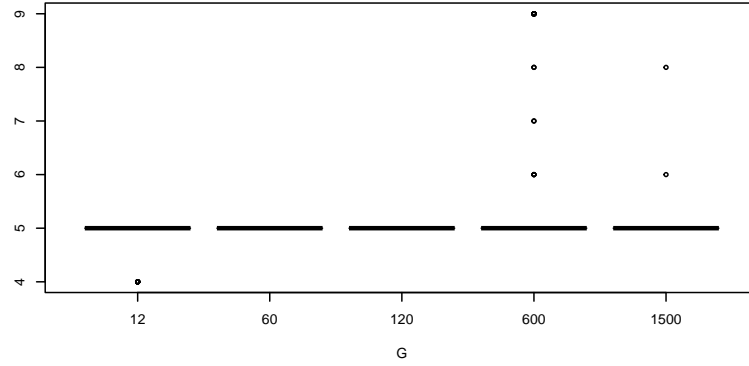

**Figure 6: Scenario 2:** Boxplots for the number of iterations until the EM algorithm converged across the simulated datasets. See also Table 7.

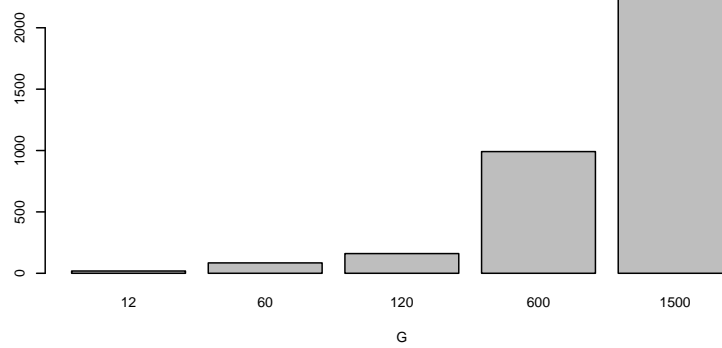

**Figure 7: Scenario 2:** Bar plot for the total computing times, in seconds, taken for the EM algorithm to converge across the simulated datasets. See also Table 8.

**Table 6: Scenario 2:** Mean and standard deviation (SD) for the estimates of  $\pi_k$  obtained for each  $k$  and each  $G$  using the EM algorithm across the simulated datasets.

| $k$ | $G$  | Mean    | SD      |
|-----|------|---------|---------|
| 1   | 12   | 0.33396 | 0.01266 |
|     | 60   | 0.33258 | 0.01346 |
|     | 120  | 0.33403 | 0.01329 |
|     | 600  | 0.33247 | 0.01318 |
|     | 1500 | 0.33383 | 0.01323 |
| 2   | 12   | 0.33200 | 0.01446 |
|     | 60   | 0.33375 | 0.01365 |
|     | 120  | 0.33238 | 0.01350 |
|     | 600  | 0.33339 | 0.01319 |
|     | 1500 | 0.33291 | 0.01353 |
| 3   | 12   | 0.33404 | 0.01374 |
|     | 60   | 0.33367 | 0.01395 |
|     | 120  | 0.33359 | 0.01362 |
|     | 600  | 0.33414 | 0.01320 |
|     | 1500 | 0.33325 | 0.01389 |

**Table 7: Scenario 2:** Mean and standard deviation (SD) for the number of iterations until the EM algorithm converged, by  $G$ , across the simulated datasets.

| $G$  | Mean    | SD      |
|------|---------|---------|
| 12   | 4.95703 | 0.20318 |
| 60   | 5.00000 | 0.00000 |
| 120  | 5.00000 | 0.00000 |
| 600  | 5.28906 | 0.98739 |
| 1500 | 5.01562 | 0.19741 |

**Table 8: Scenario 2:** Mean and standard deviation (SD) for the EM algorithm computing times, in seconds, by  $G$ , across the simulated datasets.

| $G$  | Mean    | SD      |
|------|---------|---------|
| 12   | 0.07286 | 0.01496 |
| 60   | 0.33071 | 0.03244 |
| 120  | 0.62677 | 0.03691 |
| 600  | 3.87268 | 0.55939 |
| 1500 | 9.12037 | 0.58807 |

### 1.3.3 Scenario 3

For this scenario, the number of clusters  $K$  changes, and, therefore, the corresponding probabilities of cluster assignments also change to maintain the balanced format of the clusters. We keep the values of the other parameters fixed, and their choice is shown in Table 9. Note that when the number of clusters varies, the number of  $\phi_k$  parameters changes, but their values are the same. For example, we have  $\phi_1$  and  $\phi_2$  for the case of  $K = 2$  and  $\phi_1, \phi_2, \phi_3, \phi_4, \phi_5$  for  $K = 5$ , but their values are all equal to 0.1. For Scenario 3, the true values of the  $\lambda_{gk}$ 's used to simulate the data are as follows:

$$K = 1 \rightarrow \lambda_{gk}'s = 10$$

$$K = 2 \rightarrow \lambda_{gk}'s = (10, 15)$$

$$K = 3 \rightarrow \lambda_{gk}'s = (5, 10, 15)$$

$$K = 5 \rightarrow \lambda_{gk}'s = (5, 10, 15, 20, 25)$$

So that, for example, for  $K = 5$  in the above setting, the first  $\frac{120}{5} = 24$  genes in cluster  $k = 1$  are assigned  $\lambda_{gk}$  values equal to 5, then the following 24 genes are assigned values of 10, etc. We repeat this process for the remaining clusters so that each gene's rate parameters are distinct across clusters.

**Table 9: ZIP mixture model without covariates. Scenario 3:** Values chosen for the number of clusters  $K$  in each of four different cases along with the fixed parameters used to simulate the datasets.

| Case | $N$  | $G$ | $K$ | $\phi_k$ | $\pi_k$ |
|------|------|-----|-----|----------|---------|
| 1    |      |     | 1   |          |         |
| 2    | 1200 | 120 | 2   | 0.1      | $1/K$   |
| 3    |      |     | 3   |          |         |
| 4    |      |     | 5   |          |         |

We can observe from Table (10) and Figure (8) that as the number of clusters increases, the standard deviation of the estimates of  $\phi_k$  increases due to the reduction in the number of observations per cluster since  $N$  is fixed. In addition, the estimates of  $\phi_k$ 's are centered around the true values used to simulate the data. Figure 8 and Table 11 show that the estimates of  $\pi_k$  are also centered around the true values. Note that in Figure 8, we merge the vectors of  $\pi_k$  estimates for different  $K$  into one vector in order to show their behaviour better. The standard deviations of the estimates of  $\pi_k$  remain somewhat the same across the different  $K$  choices (Table 11). From Table 12, we can see that for the  $\lambda_{gk}$ 's, the MSE increases as the number of clusters increases. In this simulation scenario, all V-measure values remain constant and equal to one, demonstrating no misclassification. The number of iterations until convergence remains the same in all cases (Table 13 and Figure 9); however, we observe an increase in computing time when the number of clusters increases (Table 14 and Figure 10).

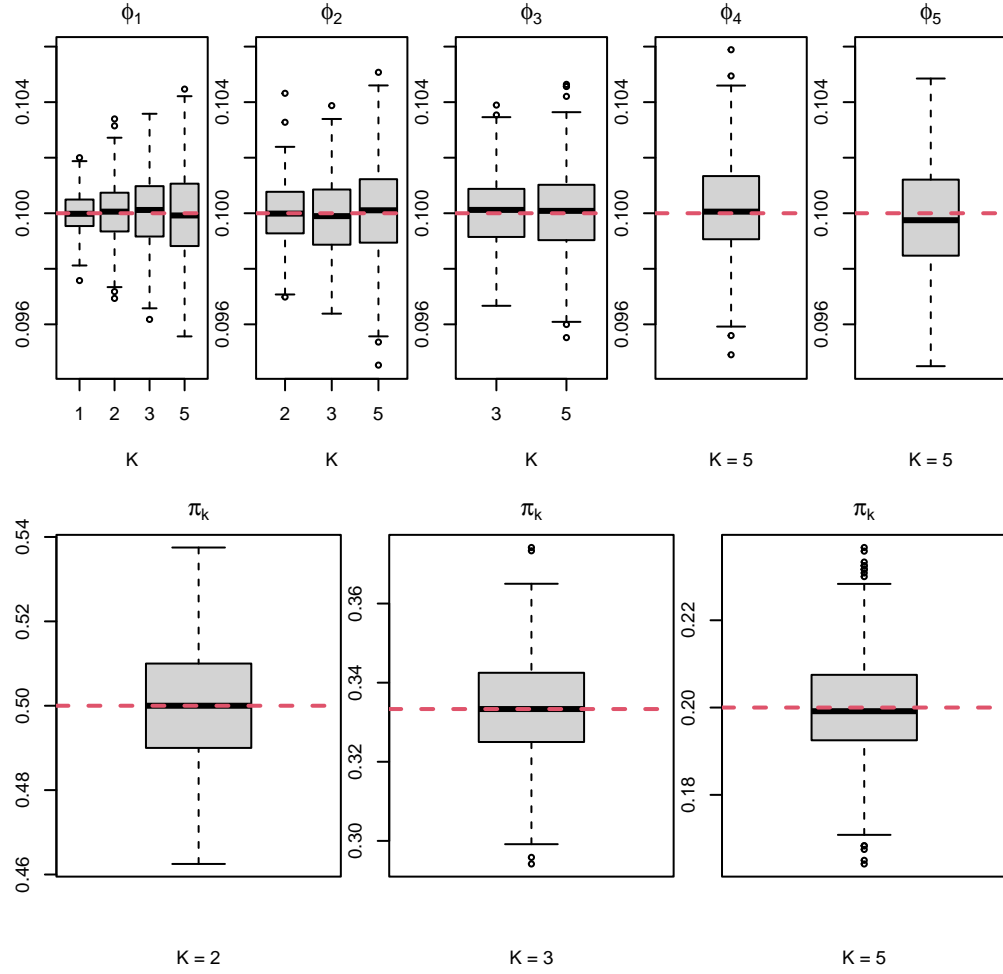

**Figure 8: ZIP mixture model without covariates. Scenario 3:** Boxplots for the estimates of  $\phi_k$  (top row) and  $\pi_k$  (bottom row), for  $k = 1, \dots, 5$  obtained using the proposed EM algorithm across the datasets simulated from the settings described in Table 9. Red lines correspond to true values. See also Tables 10 and 11.

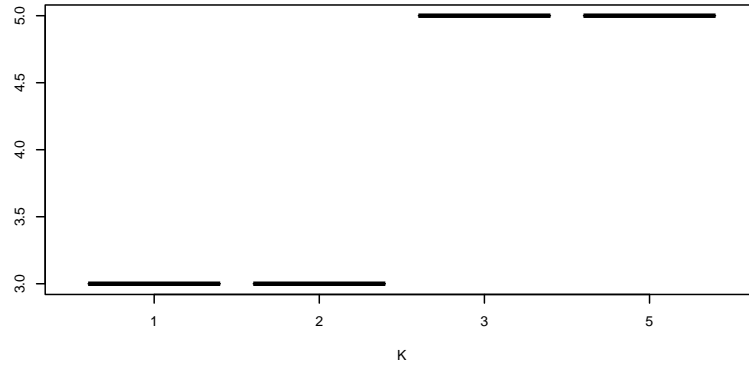

**Figure 9: Scenario 3:** Boxplots for the number of iterations until the EM algorithm converged across the datasets simulated from the settings described in Table 9. See also Table 13.

**Table 10: Scenario 3:** Mean and standard deviation (SD) for the estimates of  $\phi_k$  obtained for each  $k$  in each choice of  $K$  using the EM algorithm across the datasets simulated from the settings described in Table 9. Regarding the table structure, note that  $\phi_1$  exists for  $K = 1, 2, 3$ , and 5 clusters (all cases), while  $\phi_2$  only exists for  $K = 2, 3, 5$ ,  $\phi_3$  exists for only  $K = 3, 5$ , and finally,  $\phi_4$  and  $\phi_5$  exist only for  $K = 5$ .

| $k$ | $K$ | Mean    | SD      |
|-----|-----|---------|---------|
| 1   | 1   | 0.10001 | 0.00077 |
|     | 2   | 0.10008 | 0.00111 |
|     | 3   | 0.10004 | 0.00133 |
|     | 5   | 0.10001 | 0.00174 |
| 2   | 2   | 0.10000 | 0.00109 |
|     | 3   | 0.09991 | 0.00140 |
|     | 5   | 0.10012 | 0.00174 |
| 3   | 3   | 0.10008 | 0.00135 |
|     | 5   | 0.10007 | 0.00169 |
| 4   | 5   | 0.10011 | 0.00178 |
| 5   | 5   | 0.09977 | 0.00186 |

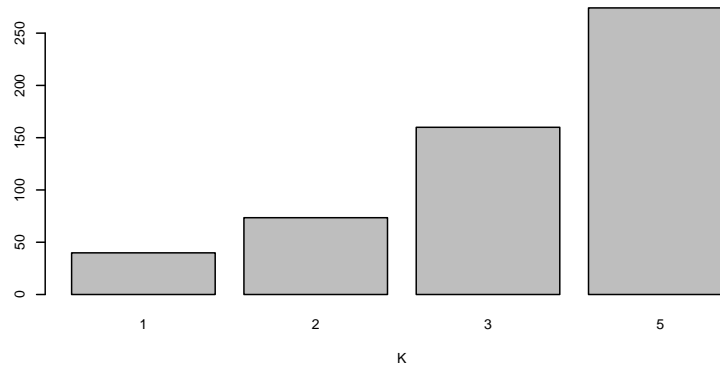

**Figure 10: Scenario 3:** Bar plot for the total computing times, in seconds, taken for the EM algorithm to converge across the datasets simulated from the settings described in Table 9. See also Table 14.

**Table 11: Scenario 3:** Mean and standard deviation (SD) for the estimates of  $\pi_k$  obtained for each  $k$  in each choice of  $K$  using the EM algorithm across the datasets simulated from the settings described in Table 9. Regarding the table structure, note that  $\pi_1$  exists for  $K = 1, 2, 3$ , and 5 clusters (all cases), while  $\pi_2$  only exists for  $K = 2, 3, 5$ ,  $\pi_3$  exists for only  $K = 3, 5$ , and finally,  $\pi_4$  and  $\pi_5$  exist only for  $K = 5$ . In addition,  $\pi_1$  is always equal to 1 when  $K = 1$ .

| $k$ | $K$ | Mean    | SD      |
|-----|-----|---------|---------|
| 1   | 1   | -       | -       |
|     | 2   | 0.49974 | 0.01406 |
|     | 3   | 0.33266 | 0.01289 |
|     | 5   | 0.20015 | 0.01160 |
| 2   | 2   | 0.50026 | 0.01406 |
|     | 3   | 0.33458 | 0.01281 |
|     | 5   | 0.19951 | 0.01182 |
| 3   | 3   | 0.33276 | 0.01288 |
|     | 5   | 0.20049 | 0.01176 |
| 4   | 5   | 0.19993 | 0.01149 |
| 5   | 5   | 0.19992 | 0.01179 |

**Table 12: Scenario 3:** Mean squared error for the EM estimates of the  $\lambda_{gk}$ 's for each  $k$  and each  $K$  across genes and simulated datasets according to the settings described in Table 9.

| $k$ | $K$     |         |         |         |
|-----|---------|---------|---------|---------|
|     | 1       | 2       | 3       | 5       |
| 1   | 0.00921 | 0.02316 | 0.02767 | 0.06997 |
| 2   |         | 0.02309 | 0.02766 | 0.06998 |
| 3   |         |         | 0.02817 | 0.06918 |
| 4   |         |         |         | 0.07115 |
| 5   |         |         |         | 0.06950 |

**Table 13: Scenario 3:** Mean and standard deviation (SD) for the number of iterations until the EM algorithm converged, by  $K$ , across the datasets simulated from the settings described in Table 9.

| $K$ | Mean | SD |
|-----|------|----|
| 1   | 3    | 0  |
| 2   | 3    | 0  |
| 3   | 5    | 0  |
| 5   | 5    | 0  |

**Table 14: Scenario 3:** Mean and standard deviation (SD) for the EM algorithm computing times, in seconds, by  $K$ , across the datasets simulated from the settings described in Table 9.

| $K$ | Mean    | SD      |
|-----|---------|---------|
| 1   | 0.15568 | 0.01381 |
| 2   | 0.28696 | 0.02467 |
| 3   | 0.62479 | 0.03260 |
| 5   | 1.07090 | 0.06759 |

### 1.3.4 Scenario 4

In this scenario, we consider two clusters and study the effect of changing the probabilities of the clusters from a balanced case to a very unbalanced case. Changes in cluster probabilities can be seen in the columns  $\pi_1$  and  $\pi_2$  of Table 15. All other parameters and hyperparameters are kept fixed according to the settings shown in Table 15.

**Table 15: ZIP mixture model without covariates. Scenario 4:** Values chosen for the proportion  $\pi_k$  assigned to each cluster  $k$  in each of four different cases along with the fixed parameters used to simulate the datasets. Note that  $\pi_2 = 1 - \pi_1$ .

| Case | $N$  | $G$ | $K$ | $\phi_k$ | $\pi_1$ | $\pi_2$ |
|------|------|-----|-----|----------|---------|---------|
| 1    | 1200 | 120 | 2   | 0.1      | 0.50    | 0.50    |
| 2    |      |     |     |          | 0.25    | 0.75    |
| 3    |      |     |     |          | 0.10    | 0.90    |
| 4    |      |     |     |          | 0.05    | 0.95    |

We can see in Figure 11 and Table 16 that as the cluster proportions change from balanced to unbalanced, the standard deviations of estimated values of  $\phi_1$  increase. At the same time, no significant changes are observed in the standard deviations of the estimates of  $\phi_2$  as  $\pi_2 \geq \pi_1$  across all cases. Moreover, the estimates of  $\phi_1$  and  $\phi_2$  are centered around their true values. Figure 11 and Table 17 show that the estimated values of  $\pi_k$  are centered around their true values, and the standard deviations are small for all cases. For the  $\lambda_{gk}$ 's, from Table 18, we can observe that the MSEs increase for the first cluster while slightly decreasing for the second cluster as  $\pi_1$  and  $\pi_2$  change from balanced to unbalanced. The V-measures for this scenario are equal to one for all cases. For the number of iterations and computing times, no considerable differences are observed in the balanced and unbalanced scenarios (Tables 19, 20 and Figures 12, 13 ).

**Table 16: Scenario 4:** Mean and standard deviation (SD) for the estimates of  $\phi_k$  obtained for each  $k$  and each case using the EM algorithm across the datasets simulated from the settings described in Table 15.

| $k$ | Case | Mean    | SD      |
|-----|------|---------|---------|
| 1   | 1    | 0.09993 | 0.00113 |
|     | 2    | 0.10008 | 0.00167 |
|     | 3    | 0.09995 | 0.00251 |
|     | 4    | 0.09984 | 0.00362 |
| 2   | 1    | 0.09989 | 0.00106 |
|     | 2    | 0.10005 | 0.00090 |
|     | 3    | 0.10003 | 0.00084 |
|     | 4    | 0.09998 | 0.00076 |

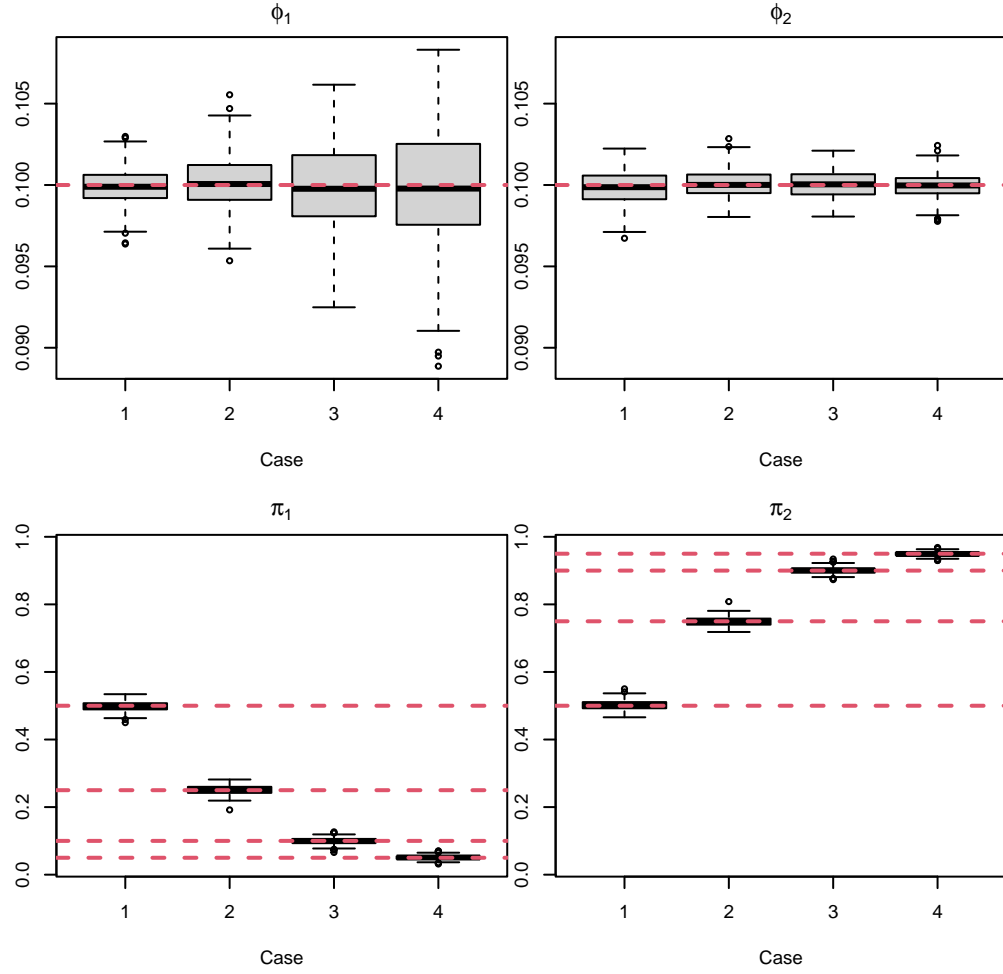

**Figure 11: ZIP mixture model without covariates. Scenario 3:** Boxplots for the estimates of  $\phi_k$  (*top row*) and  $\pi_k$  (*bottom row*), for  $k = 1, 2$  obtained using the proposed EM algorithm across the datasets simulated from the settings described in Table 15. Red lines correspond to true values. See also Tables 16 and 17.

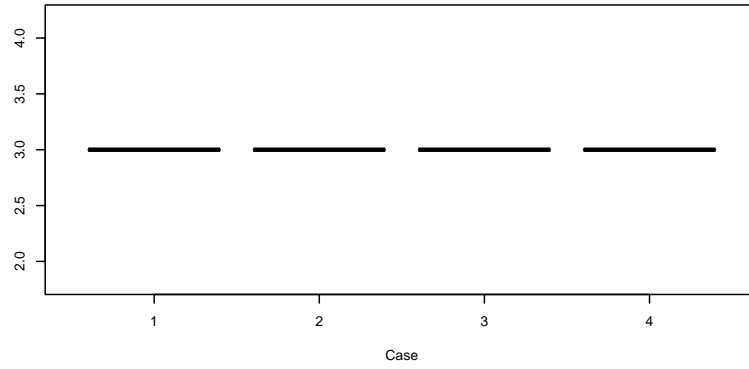

**Figure 12: Scenario 4:** Boxplots for the number of iterations until the EM algorithm converged across the datasets simulated from the settings described in Table 15. See also Table 19.

**Table 17: Scenario 4:** Mean and standard Deviation for the estimates of  $\pi_k$  obtained for each  $k$  and each case using the EM algorithm across the datasets simulated from the settings described in Table 15.

| $k$ | Case | Mean    | SD      |
|-----|------|---------|---------|
| 1   | 1    | 0.49846 | 0.01470 |
|     | 2    | 0.25039 | 0.01319 |
|     | 3    | 0.09937 | 0.00912 |
|     | 4    | 0.05069 | 0.00653 |
| 2   | 1    | 0.50154 | 0.01470 |
|     | 2    | 0.74961 | 0.01319 |
|     | 3    | 0.90063 | 0.00912 |
|     | 4    | 0.94931 | 0.00653 |

**Table 18: Scenario 4:** Mean squared error for the EM estimates of the  $\lambda_{gk}$ 's for each  $k$  and each case across genes and simulated datasets according to the settings described in Table 15.

| $k$ | Case    |         |         |         |
|-----|---------|---------|---------|---------|
|     | 1       | 2       | 3       | 4       |
| 1   | 0.02306 | 0.04653 | 0.11769 | 0.23423 |
| 2   | 0.02327 | 0.01544 | 0.01303 | 0.01208 |

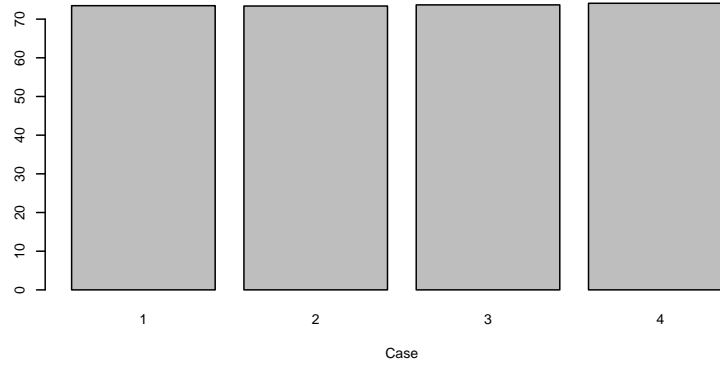

**Figure 13: Scenario 4:** Bar plot for the total computing times, in seconds, taken for the EM algorithm to converge across the datasets simulated from the settings described in Table 15. See also Table 20.

**Table 19: Scenario 4:** Mean and standard deviation (SD) for the number of iterations until the EM algorithm converged, by case, across the datasets simulated from the settings described in Table 15.

| Case | Mean | SD |
|------|------|----|
| 1    | 3    | 0  |
| 2    | 3    | 0  |
| 3    | 3    | 0  |
| 4    | 3    | 0  |

**Table 20: Scenario 4:** Mean and standard deviation (SD) for the EM algorithm computing times, in seconds, by case, across the datasets simulated from the settings described in Table 15.

| Case | Mean    | SD      |
|------|---------|---------|
| 1    | 0.28701 | 0.02457 |
| 2    | 0.28668 | 0.02583 |
| 3    | 0.28782 | 0.02587 |
| 4    | 0.28946 | 0.02601 |

### 1.3.5 Scenario 5

In this scenario, we vary the choice of the rate parameters, the  $\lambda_{gk}$ 's. In all other previous scenarios, their values are selected to avoid any overlap between the clusters. Now, in Scenario 5, considering  $p_\lambda$  as the proportion of overlap of the  $\lambda_{gk}$  values across clusters, we start from no overlap (Case 1) and go until the case of having two-thirds of the genes with the same  $\lambda_{gk}$  values across clusters (Case 5). We consider the true values of 4 and 5 for the  $\lambda_{gk}$ 's. All other parameters are kept fixed in this scenario. The settings used to simulate data under this scenario are shown in Table 21.

**Table 21: ZIP mixture model without covariates. Scenario 5:** Values chosen for the proportion of  $\lambda_{gk}$  parameters in common between the two clusters,  $p_\lambda$ , in each of six possible cases along with the fixed parameters used to simulate the datasets.

| Case | $N$  | $G$ | $K$ | $\phi_k$ | $\pi_k$ | $p_\lambda$ |
|------|------|-----|-----|----------|---------|-------------|
| 1    | 1200 | 120 | 2   | 0.1      | $1/K$   | 0           |
| 2    |      |     |     |          |         | $1/6$       |
| 3    |      |     |     |          |         | $1/3$       |
| 4    |      |     |     |          |         | $1/2$       |
| 5    |      |     |     |          |         | $2/3$       |

Figure 14 and Table 22 show that the EM estimates of  $\phi_1$  and  $\phi_2$  remain somewhat unbiased and with small standard deviations across all cases in Scenario 5. For the estimates of  $\pi_1$  and  $\pi_2$ , we can see from Figure 14 and Table 23 that they are all unbiased, while their standard deviations slightly increase in cases 4 and 5. The MSEs of the estimated values of  $\lambda_{gk}$  are slightly similar across the cases according to Table 24. Moreover, as expected, according to the V-measures, clustering performance decreases as the overlap between the clusters increases (see Figure 15). Also, computing time increases for the most complicated case with more cluster overlap (Table 25 and Figure 16). Finally, the number of iterations also increases for the more complicated cases, as expected (see Table 26 and Figure 17).

**Table 22: Scenario 5:** Mean and standard deviation (SD) for the estimates of  $\phi_k$  obtained for each  $k$  and each case using the EM algorithm across the datasets simulated from the settings described in Table 21.

| $k$ | Case | Mean    | SD      |
|-----|------|---------|---------|
| 1   | 1    | 0.09989 | 0.00123 |
|     | 2    | 0.09978 | 0.00122 |
|     | 3    | 0.09991 | 0.00132 |
|     | 4    | 0.09985 | 0.00130 |
|     | 5    | 0.09975 | 0.00134 |
| 2   | 1    | 0.09998 | 0.00116 |
|     | 2    | 0.09991 | 0.00115 |
|     | 3    | 0.09994 | 0.00111 |
|     | 4    | 0.10000 | 0.00113 |
|     | 5    | 0.09989 | 0.00145 |

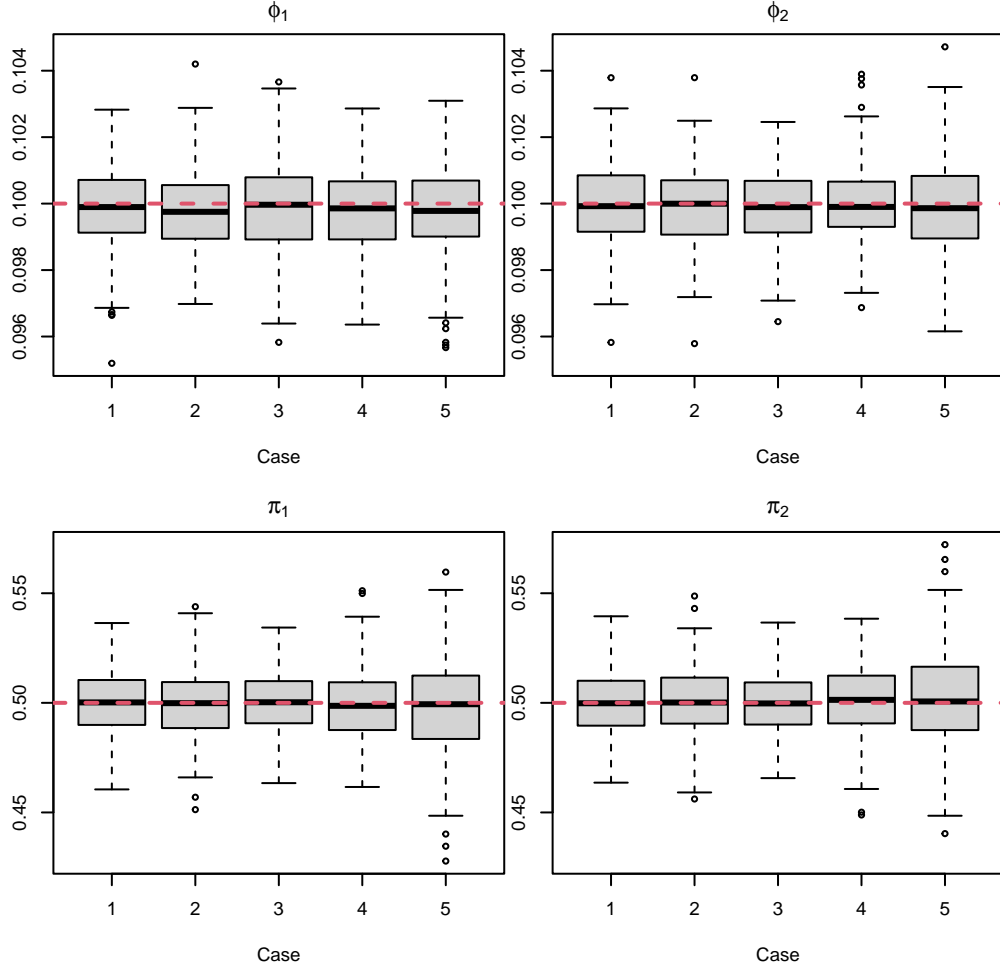

**Figure 14: ZIP mixture model without covariates. Scenario 3:** Boxplots for the estimates of  $\phi_k$  (top row) and  $\pi_k$  (bottom row), for  $k = 1, 2$  obtained using the proposed EM algorithm across the datasets simulated from the settings described in Table 21. Red lines correspond to true values. See also Tables 22 and 23.

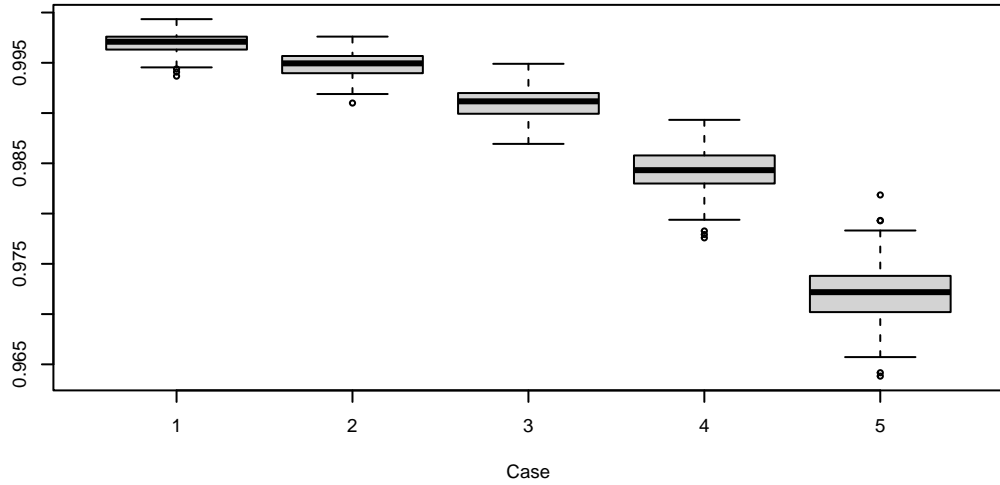

**Figure 15: Scenario 5:** Boxplots of the V-measures of the clustering obtained by the EM algorithm across the datasets simulated from the settings described in Table 21.

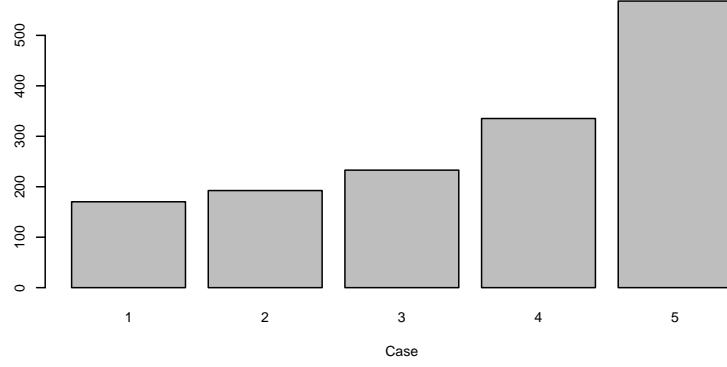

**Figure 16: Scenario 5:** Bar plot for the total computing times, in seconds, taken for the EM algorithm to converge across the datasets simulated from the settings described in Table 21. See also Table 25.

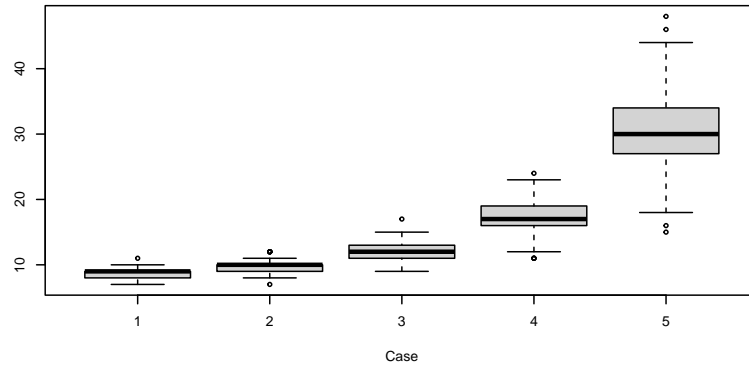

**Figure 17: Scenario 5:** Boxplots for the number of iterations until the EM algorithm converged across the datasets simulated from the settings described in Table 21. See also Table 26.

**Table 23: Scenario 5:** Mean and standard deviation (SD) for the estimates of  $\pi_k$  obtained for each  $k$  and each case using the EM algorithm across the datasets simulated from the settings described in Table 21.

| $k$ | Case | Mean    | SD      |
|-----|------|---------|---------|
| 1   | 1    | 0.50024 | 0.01459 |
|     | 2    | 0.49967 | 0.01485 |
|     | 3    | 0.50013 | 0.01443 |
|     | 4    | 0.49850 | 0.01666 |
|     | 5    | 0.49791 | 0.02190 |
| 2   | 1    | 0.49976 | 0.01459 |
|     | 2    | 0.50033 | 0.01485 |
|     | 3    | 0.49987 | 0.01443 |
|     | 4    | 0.50150 | 0.01666 |
|     | 5    | 0.50209 | 0.02190 |

**Table 24: Scenario 5:** Mean squared error for the EM estimates of the  $\lambda_{gk}$ 's for each  $k$  and each case across genes and simulated datasets according to the settings described in Table 21.

| $k$ | Case    |         |         |         |         |
|-----|---------|---------|---------|---------|---------|
|     | 1       | 2       | 3       | 4       | 5       |
| 1   | 0.00804 | 0.00813 | 0.00827 | 0.00874 | 0.00945 |
| 2   | 0.00965 | 0.00967 | 0.00947 | 0.00952 | 0.00996 |

**Table 25: Scenario 5:** Mean and standard deviation (SD) for the EM algorithm computing times, in seconds, by case, across the datasets simulated from the settings described in Table 21.

| Case | Mean    | SD      |
|------|---------|---------|
| 1    | 0.66502 | 0.06492 |
| 2    | 0.75189 | 0.07942 |
| 3    | 0.90994 | 0.11186 |
| 4    | 1.30957 | 0.18450 |
| 5    | 2.21893 | 0.38235 |

**Table 26: Scenario 5:** Mean and standard deviation (SD) for the number of iterations until the EM algorithm converged, by case, across the datasets simulated from the settings described in Table 21.

| Case | Mean     | SD      |
|------|----------|---------|
| 1    | 8.55078  | 0.71219 |
| 2    | 9.72266  | 1.00060 |
| 3    | 11.87500 | 1.42526 |
| 4    | 16.98828 | 2.30172 |
| 5    | 30.19922 | 5.38074 |

### 1.3.6 Scenario 6

The effect of changes in the probability of always zero ( $\phi_k$ ) is studied in this scenario. Considering three clusters, we first consider the same probability of always zero across all clusters, while these probabilities change from small to large (cases 1 to 5). For the last case, case 6, we consider different probabilities across clusters (see Table 27).

**Table 27: ZIP mixture model without covariates. Scenario 6:** Values chosen for the probability of always zero  $\phi_k$  in each of six different cases along with the fixed parameters used to simulate the datasets.

| Case | $N$  | $G$ | $K$ | $\phi_k$           | $\pi_k$ |
|------|------|-----|-----|--------------------|---------|
| 1    | 1200 | 120 | 3   | 0.05               | $1/K$   |
| 2    |      |     |     | 0.10               |         |
| 3    |      |     |     | 0.25               |         |
| 4    |      |     |     | 0.50               |         |
| 5    |      |     |     | 0.90               |         |
| 6    |      |     |     | (0.05, 0.25, 0.50) |         |

Both Figure 18 and Table 28 demonstrate small values of the standard deviation of the estimates of  $\phi_k$ 's and no remarkable changes across the different cases. Also, the estimates are all centered around their true values. It should be mentioned that in Figure 18, for cases 1 to 5, we merge the estimates of  $\phi_1$ ,  $\phi_2$ , and  $\phi_3$  into one vector to show their behaviour better. No significant differences are also observed in the means and standard deviations of the estimate of  $\pi_k$ 's (Table 29 and Figure 18). Table 30 shows that, for any cluster  $k$ , the MSE of the estimates of the  $\lambda_{gk}$ 's increases as the probability of always zero increases. We can also observe in Table 30 that for each cluster  $k$ , the MSEs are similar, except for the last case (case 6), where there are different probabilities of always zero in each cluster. The V-measures show a slightly worse clustering performance in case 5, where there are more zeros ( $\phi_1 = \phi_2 = \phi_3 = 0.9$ ) than in the other cases (Figure 19). Moreover, for case 5, standard deviations of the number of iterations are slightly larger than for the other cases (Table 31 and Figure 20). Also, computing times increase for cases 4 and 5, where the probabilities of always zero are large, and for case 6, where they vary across the clusters (Table 32 and Figure 21 ).

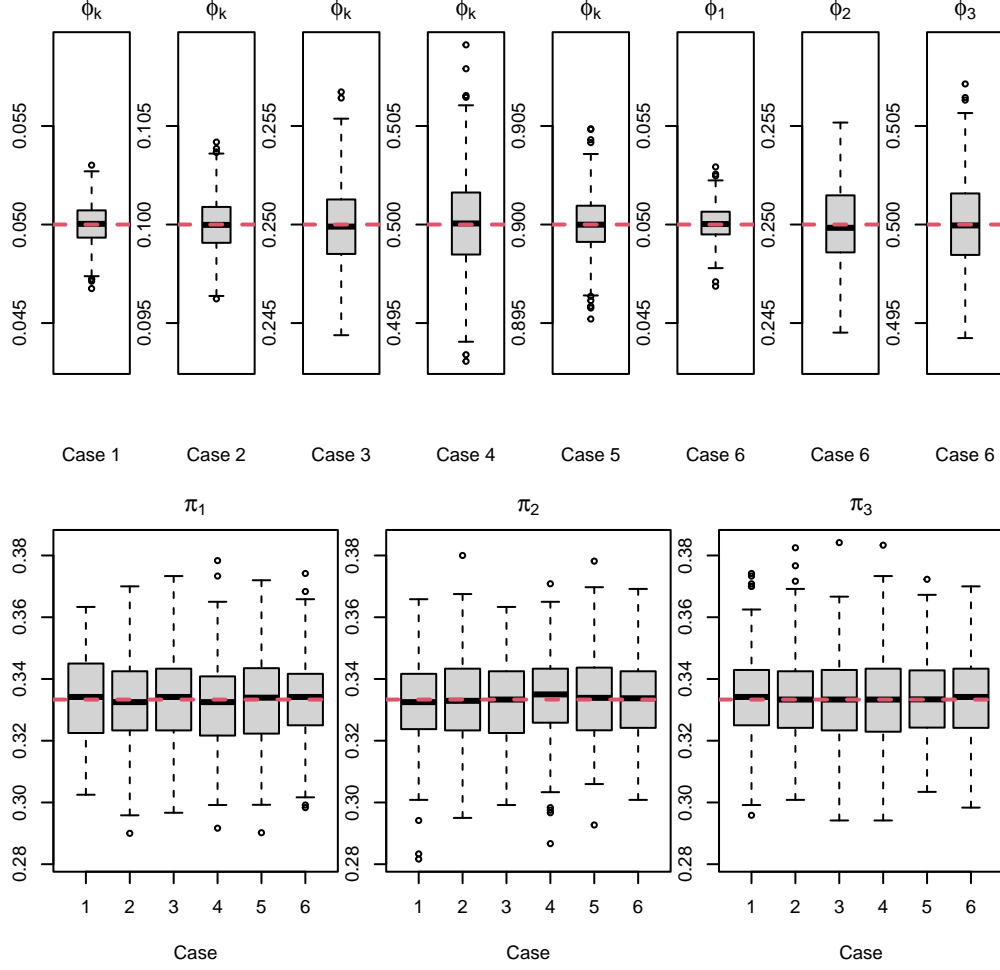

**Figure 18: ZIP mixture model without covariates. Scenario 3:** Boxplots for the estimates of  $\phi_k$  (top row) and  $\pi_k$  (bottom row), for  $k = 1, \dots, 3$  obtained using the proposed EM algorithm across the datasets simulated from the settings described in Table 27. Red lines correspond to true values. See also Tables 28 and 29.

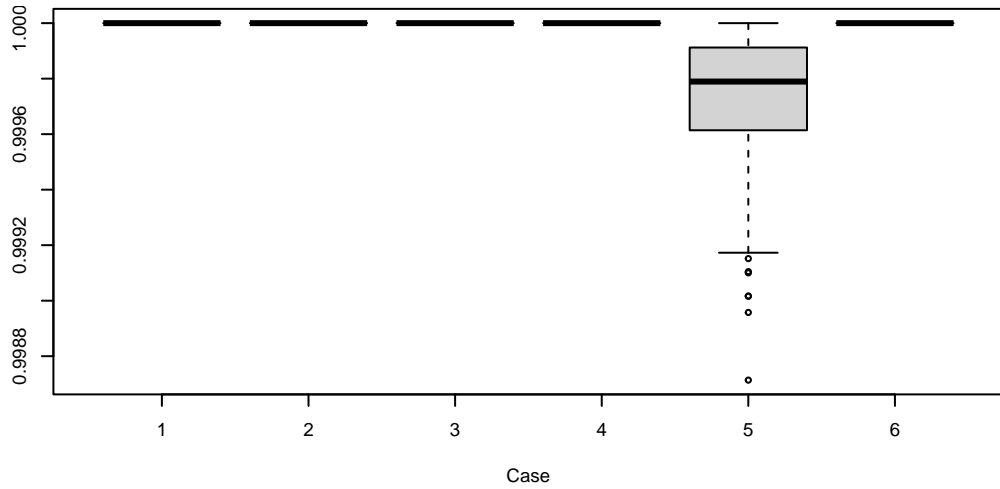

**Figure 19: Scenario 6:** Boxplots for the V-measures of the clustering obtained by the EM algorithm across the datasets simulated from the settings described in Table 27.

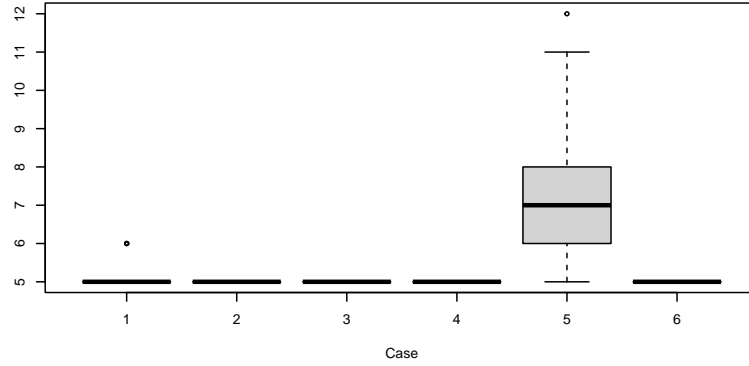

**Figure 20: Scenario 6:** Boxplots for the number of iterations until the EM algorithm converged across the datasets simulated from the settings described in Table 27. See also Table 31.

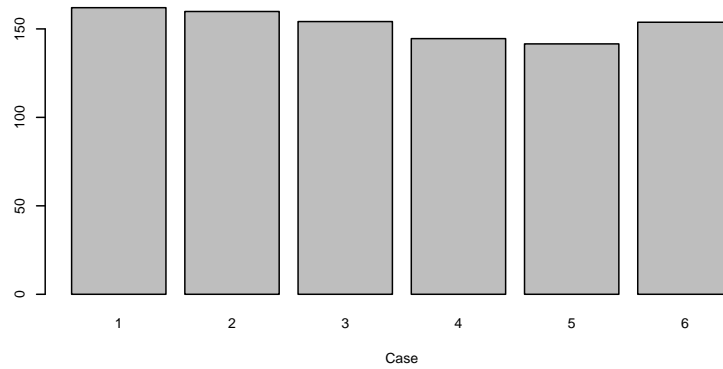

**Figure 21: Scenario 6:** Bar plot for the total computing times, in seconds, taken for the EM algorithm to converge across the datasets simulated from the settings described in Table 27. See also Table 32.

**Table 28: Scenario 6:** Mean and standard deviation for the estimates of  $\phi_k$  obtained for each  $k$  and each case using the EM algorithm across the datasets simulated from the settings described in Table 27.

| $\phi_k$ | Case | Mean    | SD      |
|----------|------|---------|---------|
| $\phi_1$ | 1    | 0.05006 | 0.00093 |
|          | 2    | 0.10003 | 0.00140 |
|          | 3    | 0.24992 | 0.00188 |
|          | 4    | 0.50034 | 0.00234 |
|          | 5    | 0.90006 | 0.00144 |
|          | 6    | 0.05007 | 0.00099 |
| $\phi_2$ | 1    | 0.04989 | 0.00106 |
|          | 2    | 0.09994 | 0.00134 |
|          | 3    | 0.25001 | 0.00195 |
|          | 4    | 0.49992 | 0.00214 |
|          | 5    | 0.89987 | 0.00139 |
|          | 6    | 0.24996 | 0.00201 |
| $\phi_3$ | 1    | 0.05006 | 0.00104 |
|          | 2    | 0.10010 | 0.00145 |
|          | 3    | 0.24981 | 0.00195 |
|          | 4    | 0.49990 | 0.00239 |
|          | 5    | 0.90006 | 0.00137 |
|          | 6    | 0.50007 | 0.00240 |

**Table 29: Scenario 6:** Mean and standard deviation for the estimates of  $\pi_k$  obtained for each  $k$  and each case using the EM algorithm across the datasets simulated from the settings described in Table 27.

| $\pi_k$ | Case | Mean    | SD      |
|---------|------|---------|---------|
| $\pi_1$ | 1    | 0.33378 | 0.01395 |
|         | 2    | 0.33344 | 0.01388 |
|         | 3    | 0.33390 | 0.01424 |
|         | 4    | 0.33157 | 0.01438 |
|         | 5    | 0.33285 | 0.01484 |
|         | 6    | 0.33345 | 0.01359 |
| $\pi_2$ | 1    | 0.33214 | 0.01418 |
|         | 2    | 0.33278 | 0.01467 |
|         | 3    | 0.33251 | 0.01354 |
|         | 4    | 0.33445 | 0.01347 |
|         | 5    | 0.33357 | 0.01382 |
|         | 6    | 0.33315 | 0.01287 |
| $\pi_3$ | 1    | 0.33408 | 0.01424 |
|         | 2    | 0.33379 | 0.01367 |
|         | 3    | 0.33359 | 0.01403 |
|         | 4    | 0.33398 | 0.01428 |
|         | 5    | 0.33358 | 0.01323 |
|         | 6    | 0.33340 | 0.01387 |

**Table 30: Scenario 6:** Mean squared error for the EM estimates of the  $\lambda_{gk}$ 's for each  $k$  and each  $N$  across genes and simulated datasets according to the settings described in Table 27.

| $k$ | Case    |         |         |         |         |         |
|-----|---------|---------|---------|---------|---------|---------|
|     | 1       | 2       | 3       | 4       | 5       | 6       |
| 1   | 0.02645 | 0.02775 | 0.03323 | 0.05075 | 0.25699 | 0.02649 |
| 2   | 0.02629 | 0.02795 | 0.03420 | 0.05042 | 0.25946 | 0.03409 |
| 3   | 0.02626 | 0.02808 | 0.03321 | 0.05096 | 0.25699 | 0.05017 |

**Table 31: Scenario 6:** Mean and standard deviation (SD) for the number of iterations until the EM algorithm converged, by case, across the datasets simulated from the settings described in Table 27.

| Case | Mean    | SD      |
|------|---------|---------|
| 1    | 5.01172 | 0.10783 |
| 2    | 5.00000 | 0.00000 |
| 3    | 5.00000 | 0.00000 |
| 4    | 5.00000 | 0.00000 |
| 5    | 6.86719 | 1.24850 |
| 6    | 5.00000 | 0.00000 |

**Table 32: Scenario 6:** Mean and standard deviation (SD) for the EM algorithm computing times, in seconds, by case, across the datasets simulated from the settings described in Table 27.

| Case | Mean    | SD      |
|------|---------|---------|
| 1    | 0.63283 | 0.04231 |
| 2    | 0.62440 | 0.03581 |
| 3    | 0.60219 | 0.03868 |
| 4    | 0.56450 | 0.04575 |
| 5    | 0.55288 | 0.10138 |
| 6    | 0.60067 | 0.03832 |

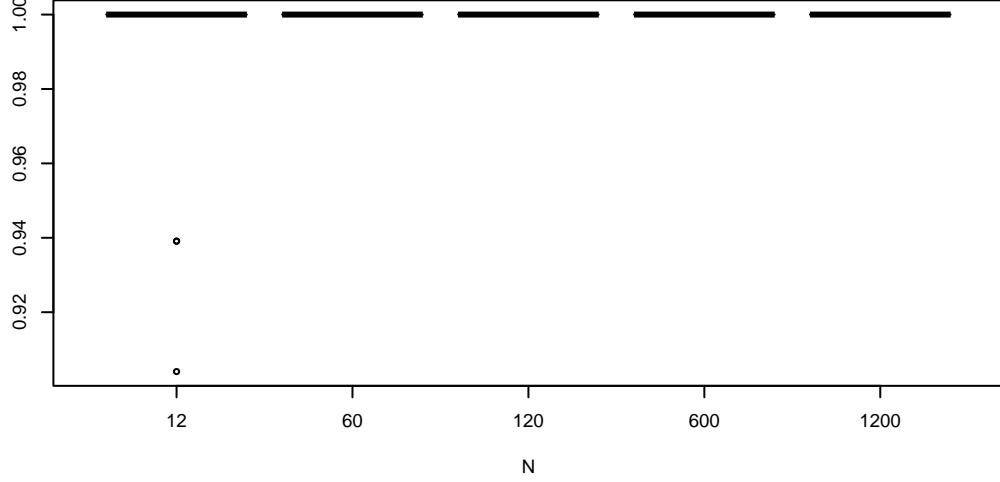

**Figure 22: Scenario 1:** Boxplots for the  $V$ -measures of the clustering obtained by the EM algorithm across the simulated datasets.

## 1.4 Simulation results for the ZIP mixture model with a size factor

### 1.4.1 Scenario 1

**Table 33: Scenario 1:** Mean and standard deviation (SD) for the estimates of  $\phi_k$  for each  $k$  and each  $N$ , obtained using the EM algorithm across the simulated datasets.

| $\phi_k$ | $N$  | Mean    | SD      |
|----------|------|---------|---------|
| $\phi_1$ | 12   | 0.09738 | 0.01496 |
|          | 60   | 0.10003 | 0.00655 |
|          | 120  | 0.09983 | 0.00416 |
|          | 600  | 0.09999 | 0.00195 |
|          | 1200 | 0.10027 | 0.00125 |
| $\phi_2$ | 12   | 0.09748 | 0.01473 |
|          | 60   | 0.10020 | 0.00628 |
|          | 120  | 0.09978 | 0.00448 |
|          | 600  | 0.10001 | 0.00199 |
|          | 1200 | 0.10020 | 0.00139 |
| $\phi_3$ | 12   | 0.09714 | 0.01625 |
|          | 60   | 0.09961 | 0.00642 |
|          | 120  | 0.09987 | 0.00427 |
|          | 600  | 0.10003 | 0.00205 |
|          | 1200 | 0.09994 | 0.00139 |

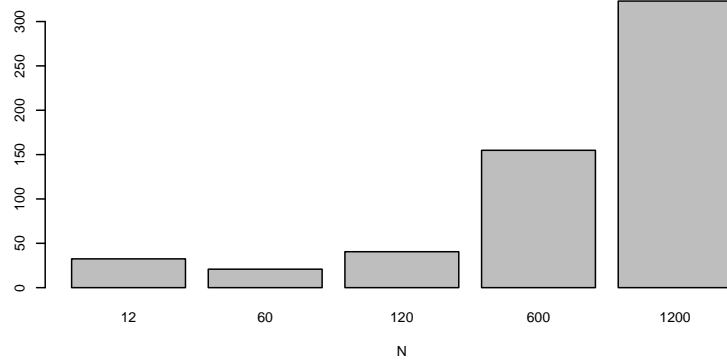

**Figure 23: Scenario 1:** Bar plot for the total computing times, in seconds, taken for the EM algorithm to converge across the simulated datasets. See also Table 35.

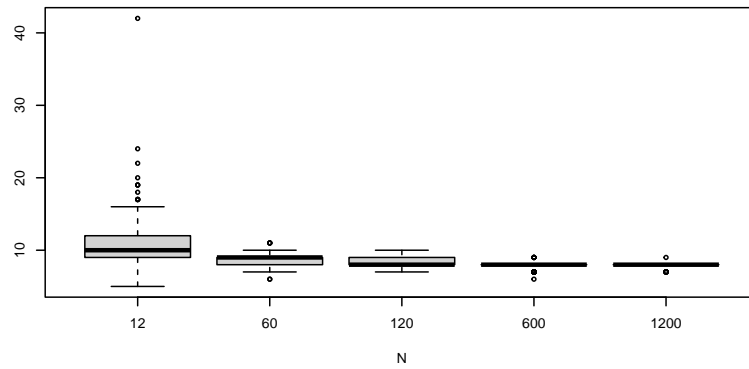

**Figure 24: Scenario 1:** Boxplots for the number of iterations until the EM algorithm converged across the simulated datasets. See also Table 36.

**Table 34: Scenario 1:** Mean and standard deviation for the estimates of  $\pi_k$  for each  $k$  and each  $N$ , obtained using the EM algorithm across the simulated datasets.

| $\pi_k$ | $N$  | Mean    | SD      |
|---------|------|---------|---------|
| $\pi_1$ | 12   | 0.35156 | 0.12500 |
|         | 60   | 0.33841 | 0.06177 |
|         | 120  | 0.33490 | 0.04423 |
|         | 600  | 0.33444 | 0.01958 |
|         | 1200 | 0.33292 | 0.01328 |
| $\pi_2$ | 12   | 0.33952 | 0.13218 |
|         | 60   | 0.33333 | 0.06444 |
|         | 120  | 0.33402 | 0.04170 |
|         | 600  | 0.33236 | 0.01870 |
|         | 1200 | 0.33380 | 0.01333 |
| $\pi_3$ | 12   | 0.30892 | 0.12448 |
|         | 60   | 0.32826 | 0.05925 |
|         | 120  | 0.33109 | 0.04288 |
|         | 600  | 0.33320 | 0.01748 |
|         | 1200 | 0.33328 | 0.01330 |

**Table 35: Scenario 1:** Mean and standard deviation (SD) for the EM algorithm computing times, in seconds, by  $N$ , across the simulated datasets.

| $N$  | Mean    | SD      |
|------|---------|---------|
| 12   | 0.12676 | 0.11630 |
| 60   | 0.08136 | 0.01778 |
| 120  | 0.15825 | 0.02253 |
| 600  | 0.60486 | 0.05189 |
| 1200 | 1.26211 | 0.11048 |

**Table 36: Scenario 1:** Mean and standard deviation (SD) for the number of iterations until the EM algorithm converged, by  $N$ , across the simulated datasets.

| $N$  | Mean     | SD      |
|------|----------|---------|
| 12   | 11.19531 | 3.35964 |
| 60   | 8.64844  | 0.78305 |
| 120  | 8.27734  | 0.63031 |
| 600  | 7.88281  | 0.39845 |
| 1200 | 7.96094  | 0.21337 |

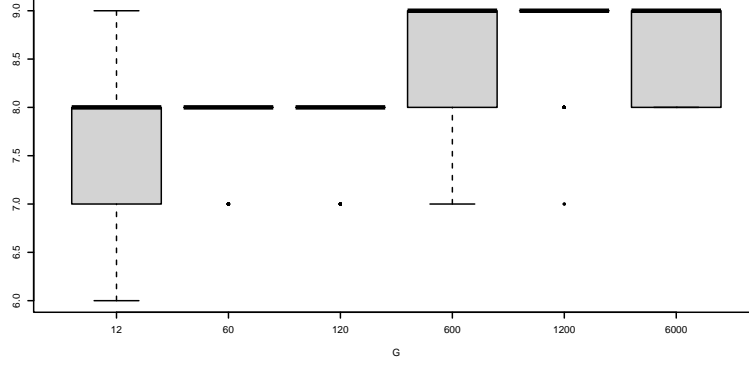

**Figure 25: Scenario 2:** Boxplots for the number of iterations until the EM algorithm converged across the simulated datasets. See also Table 39.

### 1.4.2 Scenario 2

**Table 37: Scenario 2:** Mean and standard deviation (SD) for the estimates of  $\phi_k$  for each  $k$  and each  $G$ , obtained using the EM algorithm across the simulated datasets.

| $\phi_k$ | $G$  | Mean    | SD      |
|----------|------|---------|---------|
| $\phi_1$ | 12   | 0.10021 | 0.00457 |
|          | 60   | 0.10027 | 0.00214 |
|          | 120  | 0.10021 | 0.00141 |
|          | 600  | 0.10015 | 0.00060 |
|          | 1200 | 0.10013 | 0.00047 |
|          | 6000 | 0.10016 | 0.00023 |
| $\phi_2$ | 12   | 0.10021 | 0.00422 |
|          | 60   | 0.10015 | 0.00199 |
|          | 120  | 0.10005 | 0.00133 |
|          | 600  | 0.10017 | 0.00061 |
|          | 1200 | 0.10022 | 0.00049 |
|          | 6000 | 0.10017 | 0.00024 |
| $\phi_3$ | 12   | 0.09993 | 0.00419 |
|          | 60   | 0.10008 | 0.00187 |
|          | 120  | 0.10016 | 0.00126 |
|          | 600  | 0.10014 | 0.00061 |
|          | 1200 | 0.10019 | 0.00047 |
|          | 6000 | 0.10017 | 0.00024 |

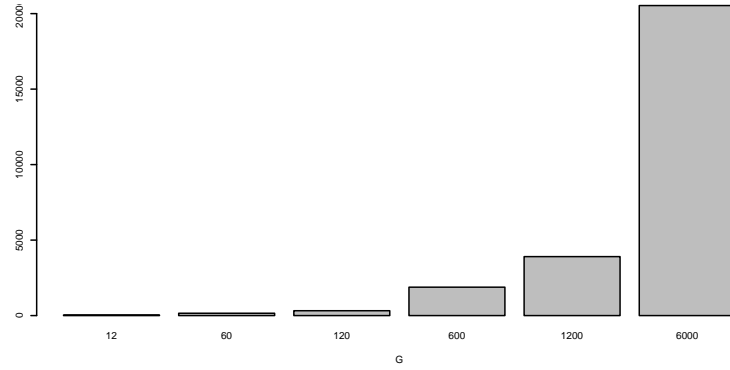

**Figure 26: Scenario 2:** Bar plot for the total computing times, in seconds, taken for the EM algorithm to converge across the simulated datasets. See also Table 40.

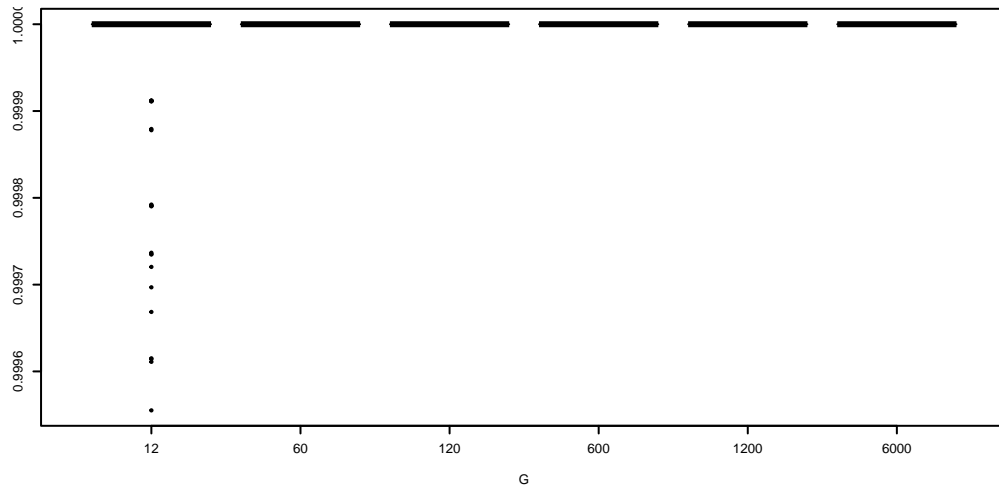

**Figure 27: Scenario 2:** Boxplots for the V-measures of the clustering obtained by the EM algorithm across the simulated datasets.

**Table 38: Scenario 2:** Mean and standard deviation (SD) for the estimates of  $\pi_k$  for each  $k$  and each  $G$ , obtained using the EM algorithm across the simulated datasets.

| $\pi_k$ | $G$  | Mean    | SD      |
|---------|------|---------|---------|
| $\pi_1$ | 12   | 0.33115 | 0.01282 |
|         | 60   | 0.33486 | 0.01351 |
|         | 120  | 0.33135 | 0.01334 |
|         | 600  | 0.33437 | 0.01373 |
|         | 1200 | 0.33301 | 0.01280 |
|         | 6000 | 0.33365 | 0.01426 |
| $\pi_2$ | 12   | 0.33442 | 0.01320 |
|         | 60   | 0.33349 | 0.01266 |
|         | 120  | 0.33472 | 0.01439 |
|         | 600  | 0.33385 | 0.01349 |
|         | 1200 | 0.33363 | 0.01346 |
|         | 6000 | 0.33223 | 0.01306 |
| $\pi_3$ | 12   | 0.33443 | 0.01311 |
|         | 60   | 0.33165 | 0.01382 |
|         | 120  | 0.33393 | 0.01312 |
|         | 600  | 0.33178 | 0.01462 |
|         | 1200 | 0.33336 | 0.01371 |
|         | 6000 | 0.33412 | 0.01397 |

**Table 39: Scenario 2:** Mean and standard deviation (SD) for the number of iterations until the EM algorithm converged, by  $G$ , across the simulated datasets.

| $G$  | Mean    | SD      |
|------|---------|---------|
| 12   | 7.63672 | 0.53583 |
| 60   | 7.89844 | 0.30266 |
| 120  | 7.94141 | 0.23532 |
| 600  | 8.69141 | 0.47946 |
| 1200 | 8.76953 | 0.44015 |
| 6000 | 8.52734 | 0.50023 |

**Table 40: Scenario 2:** Mean and standard deviation (SD) for the EM algorithm computing times, in seconds, by  $G$ , across the simulated datasets.

| $G$  | Mean     | SD      |
|------|----------|---------|
| 12   | 0.14569  | 0.01856 |
| 60   | 0.60723  | 0.04875 |
| 120  | 1.25957  | 0.11428 |
| 600  | 7.35106  | 0.71482 |
| 1200 | 15.25344 | 1.32889 |
| 6000 | 80.20718 | 5.61694 |

### 1.4.3 Scenario 3

For this scenario, after fixing  $N$  and  $G$ , we vary  $K$  as the number of clusters to evaluate how that affect the EM parameter estimation. For this scenario, the true values of the  $\rho_{gk}$ 's used to simulate the data are as follows:

$$K = 1 \rightarrow \rho_{gk}'s = 0$$

$$K = 2 \rightarrow \rho_{gk}'s = (-0.6, 0.6)$$

$$K = 3 \rightarrow \rho_{gk}'s = (-0.6, 0, 0.6)$$

$$K = 5 \rightarrow \rho_{gk}'s = (-0.8, -0.6, 0, 0.6, 0.8)$$

So that, for example, for  $K = 5$  in the above setting, the first  $\frac{120}{5} = 24$  genes in cluster  $k = 1$  are assigned  $\rho_{gk}$  values equal to  $-0.8$ , then the following 24 genes are assigned values of  $-0.6$ , etc. We repeat this process for the remaining clusters so that each gene's rate parameters are distinct across clusters. Table 41 shows the parameter setting for this scenario.

As can be seen in both Tables 42, 43 and Figure 28, the estimates of  $\phi_k$  and  $\pi_k$  are very close to their true values. For the estimates of  $\phi_k$ , the standard deviations are lower for small  $K$  and become larger when  $K$  increases. The standard deviations of the estimates of  $\pi_k$  are almost the same and small as we change  $K$ . Note that, in Figure 28, the resulted estimates of  $\pi_k$  for different  $K$  are all merged into one vector to show their behavior more exactly, which shows the closeness of the estimates to their true values and their stable standard deviations in all cases. Tables 44 and 45 show that for most cases, the MSEs for the estimates of  $\rho_{gk}$  and  $\beta_{0g}$  are small, showing their closeness to their true corresponding values. The average number of iterations for most cases is around 9, with fewer iterations needed when there is no cluster (i.e.,  $K = 1$ , see Table 46 and Figure 29). Furthermore, computation time increases as the number of clusters increases (Table 47 and Figure 30), which is expected. And finally, all V-measures demonstrate true clustering assignments and are equal to one.

**Table 41: ZIP mixture model with a size factor. Scenario 3:** Values chosen for the number of clusters  $K$  in each case along with the fixed parameters used to simulate the datasets.

| Case | $N$  | $G$ | $K$ | $\phi_k$ | $\pi_k$ |
|------|------|-----|-----|----------|---------|
| 1    | 1200 | 120 | 1   | 0.1      | $1/K$   |
| 2    |      |     | 2   |          |         |
| 3    |      |     | 3   |          |         |
| 4    |      |     | 5   |          |         |

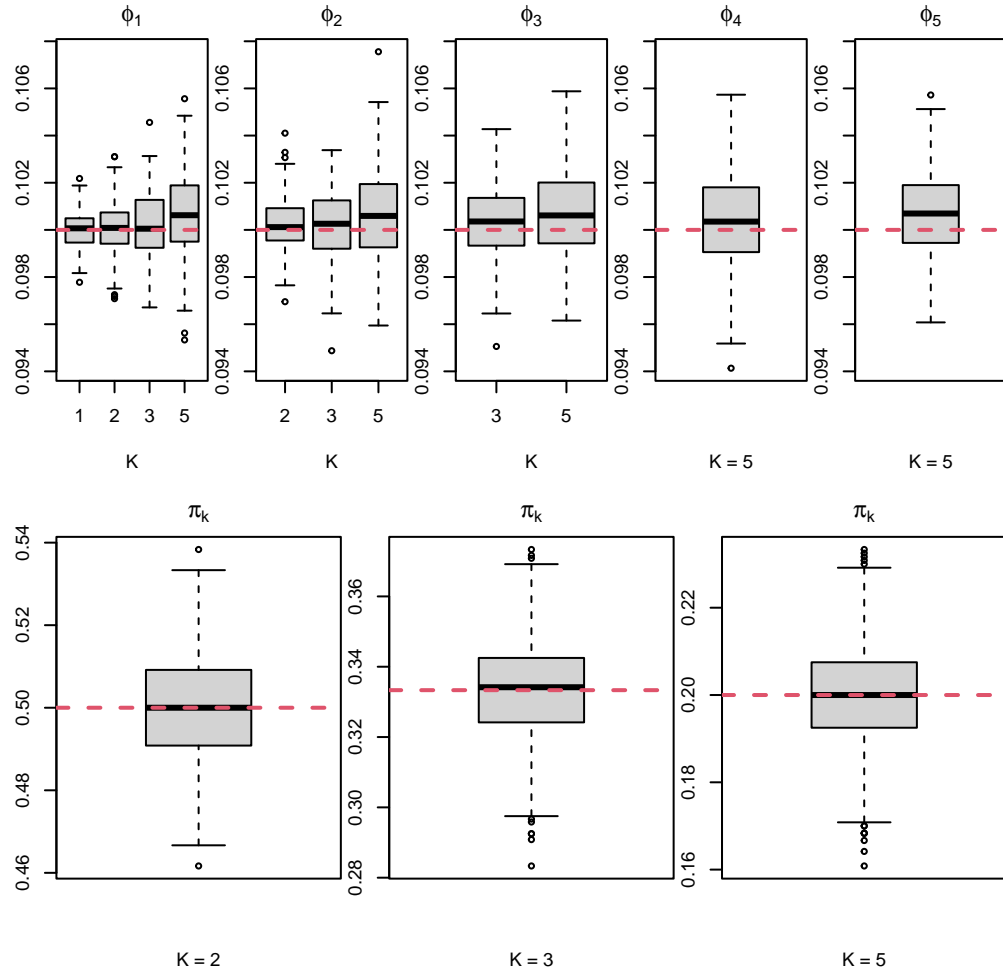

**Figure 28: ZIP mixture model without covariates. Scenario 3:** Boxplots for the estimates of  $\phi_k$  (top row) and  $\pi_k$  (bottom row), for  $k = 1, \dots, 5$  obtained using the proposed EM algorithm across the datasets simulated from the settings described in Table 41. Red lines correspond to true values. See also Tables 42 and 43.

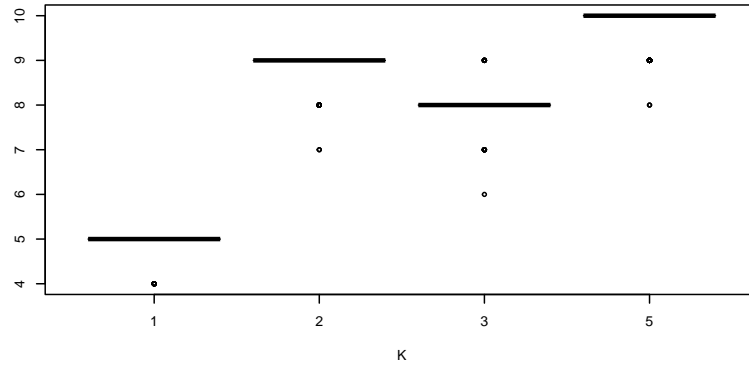

**Figure 29: Scenario 3:** Boxplots for the number of iterations until the EM algorithm converged across the datasets simulated from the settings described in Table 41. See also Table 46.

**Table 42: Scenario 3:** Mean and standard deviations for the estimates of  $\phi_k$  for each  $k$  and each  $K$ , obtained using the EM algorithm across the datasets simulated from the settings described in Table 41.

| $\phi_k$ | $K$ | Mean    | SD      |
|----------|-----|---------|---------|
| $\phi_1$ | 1   | 0.09998 | 0.00074 |
|          | 2   | 0.10008 | 0.00114 |
|          | 3   | 0.10016 | 0.00139 |
|          | 5   | 0.10065 | 0.00178 |
| $\phi_2$ | 2   | 0.10017 | 0.00109 |
|          | 3   | 0.10024 | 0.00142 |
|          | 5   | 0.10068 | 0.00191 |
| $\phi_3$ | 3   | 0.10030 | 0.00148 |
|          | 5   | 0.10072 | 0.00182 |
| $\phi_4$ | 5   | 0.10040 | 0.00192 |
| $\phi_5$ | 5   | 0.10073 | 0.00177 |

**Table 43: Scenario 3:** Mean and standard deviation for the estimates of  $\pi_k$  for each  $k$  and each  $K$ , obtained using the EM algorithm across the datasets simulated from the settings described in Table 41.

| $\pi_k$ | $K$ | Mean    | SD      |
|---------|-----|---------|---------|
| $\pi_1$ | 1   | 1.00000 | 0.00000 |
|         | 2   | 0.50001 | 0.01348 |
|         | 3   | 0.33347 | 0.01482 |
|         | 5   | 0.20009 | 0.01170 |
| $\pi_2$ | 2   | 0.49999 | 0.01348 |
|         | 3   | 0.33316 | 0.01414 |
|         | 5   | 0.19911 | 0.01142 |
| $\pi_3$ | 3   | 0.33337 | 0.01443 |
|         | 5   | 0.19873 | 0.01164 |
| $\pi_4$ | 5   | 0.20121 | 0.01079 |
| $\pi_5$ | 5   | 0.20086 | 0.01070 |

**Table 44: Scenario 3:** Mean squared error for the estimates of  $\rho_{gk}$  for each  $k$  and each  $K$ , using the EM algorithm across the datasets simulated from the settings described in Table 41.

| $k$ | $K$ |             |             |             |
|-----|-----|-------------|-------------|-------------|
|     | 1   | 2           | 3           | 5           |
| 1   | 0   | 0.000129537 | 0.000235247 | 0.000525599 |
| 2   |     | 0.000129537 | 0.000238153 | 0.000529169 |
| 3   |     |             | 0.000236647 | 0.000515542 |
| 4   |     |             |             | 0.000515218 |
| 5   |     |             |             | 0.000519752 |

**Table 45: Scenario 3:** Mean squared error for the estimates of  $\beta_{0g}$  for each  $K$ , using the EM algorithm across the datasets simulated from the settings described in Table 41.

| $K$         |             |             |             |
|-------------|-------------|-------------|-------------|
| 1           | 2           | 3           | 5           |
| 0.000101369 | 0.000117110 | 0.000112684 | 0.000121417 |

**Table 46: Scenario 3:** Mean and standard deviation (SD) for the number of iterations until the EM algorithm converged, by  $K$ , across the datasets simulated from the settings described in Table 41.

| $K$ | Mean    | SD      |
|-----|---------|---------|
| 1   | 4.95312 | 0.21179 |
| 2   | 8.87500 | 0.35425 |
| 3   | 7.99609 | 0.30030 |
| 5   | 9.79297 | 0.42485 |

**Table 47: Scenario 3:** Mean and standard deviation (SD) for the EM algorithm computing times, in seconds, by  $K$ , across the datasets simulated from the settings described in Table 41.

| $K$ | Mean    | SD      |
|-----|---------|---------|
| 1   | 0.25657 | 0.02467 |
| 2   | 0.90463 | 0.06559 |
| 3   | 1.27514 | 0.09175 |
| 5   | 2.68266 | 0.19326 |

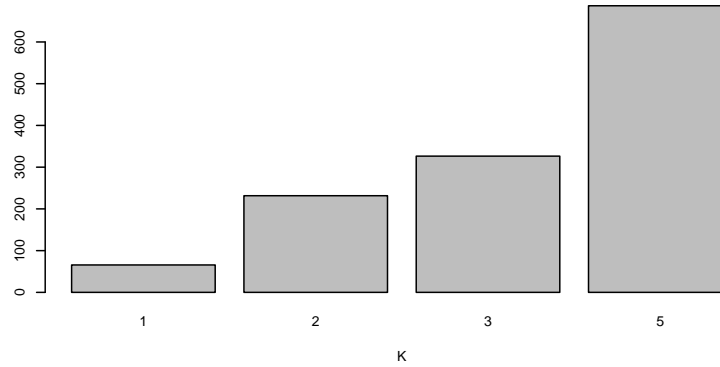

**Figure 30: Scenario 3:** Bar plot for the total computing times, in seconds, taken for the EM algorithm to converge across the datasets simulated from the settings described in Table 41. See also Table 47.

#### 1.4.4 Scenario 4

In this scenario, we investigate the sensitivity of our proposed EM algorithm to the choice of initial parameter values. We consider two cases and for both of them, we simulate data from the setting in Table 48, and the method described in detail in Section 1.4 for the cluster effect parameters. For case 1, we consider the true values as the initial parameter values as in all other simulation scenarios. In case 2, we use the  $K$ -means initialization approach to obtain initial clusters. Then, we find the initial parameter values for the obtained clusters as described in the following paragraph.

We find the initial values of the cluster assignment probabilities ( $\pi_k^{(0)}$ ) by calculating the number of cells in each obtained cluster divided by the total number of cells ( $N = 1200$ ). Then, we calculate the proportions of zero in each cluster as initial values for  $\phi_k^{(0)}$ . Finally, we compute the means over the genes for each inferred cluster as the initial values of the rate parameters ( $\lambda_{gk}^{(0)}$ ).

As can be seen in Tables 49 and 50 and Figure 31 the estimates of  $\phi_k$ 's and  $\pi_k$ 's are centered at their true values in both cases. However, there are some outliers in case 2 with larger standard deviations. According to Tables 51 and 52, the estimates for the parameters  $\beta_{0g}$  and  $\rho_{gk}$  all have reasonably small MADs in both cases, although higher values for case 2. Furthermore, most of the time the V-measures are approximately one (all greater than 0.95), except for some misclassification that occurred in case 2 (Figure 32). In most simulations, the number of iterations is almost the same, and not too many iterations are needed for convergence, but there were some cases with more iterations for case 2 (Table 53 and Figure 33). Finally, the computation time was considerably longer for case 2 (Table 54 and Figure 34)

**Table 48: ZIP mixture model with a size factor. Scenario 4:** Values chosen for the fixed parameters used to simulate the datasets.

| $N$  | $G$ | $K$ | $\phi_k$ | $\pi_k$ |
|------|-----|-----|----------|---------|
| 1200 | 120 | 3   | 0.1      | $1/K$   |

**Table 49: Scenario 4:** Mean and standard deviation (SD) for the estimates of  $\phi_k$  for each  $k$  and each case, obtained using the EM algorithm across the datasets simulated from the settings described in Table 48.

| $\phi_k$ | Case | Mean    | SD      |
|----------|------|---------|---------|
| $\phi_1$ | 1    | 0.10023 | 0.00142 |
|          | 2    | 0.09962 | 0.00956 |
| $\phi_2$ | 1    | 0.10003 | 0.00140 |
|          | 2    | 0.09946 | 0.00825 |
| $\phi_3$ | 1    | 0.10017 | 0.00140 |
|          | 2    | 0.09899 | 0.01376 |

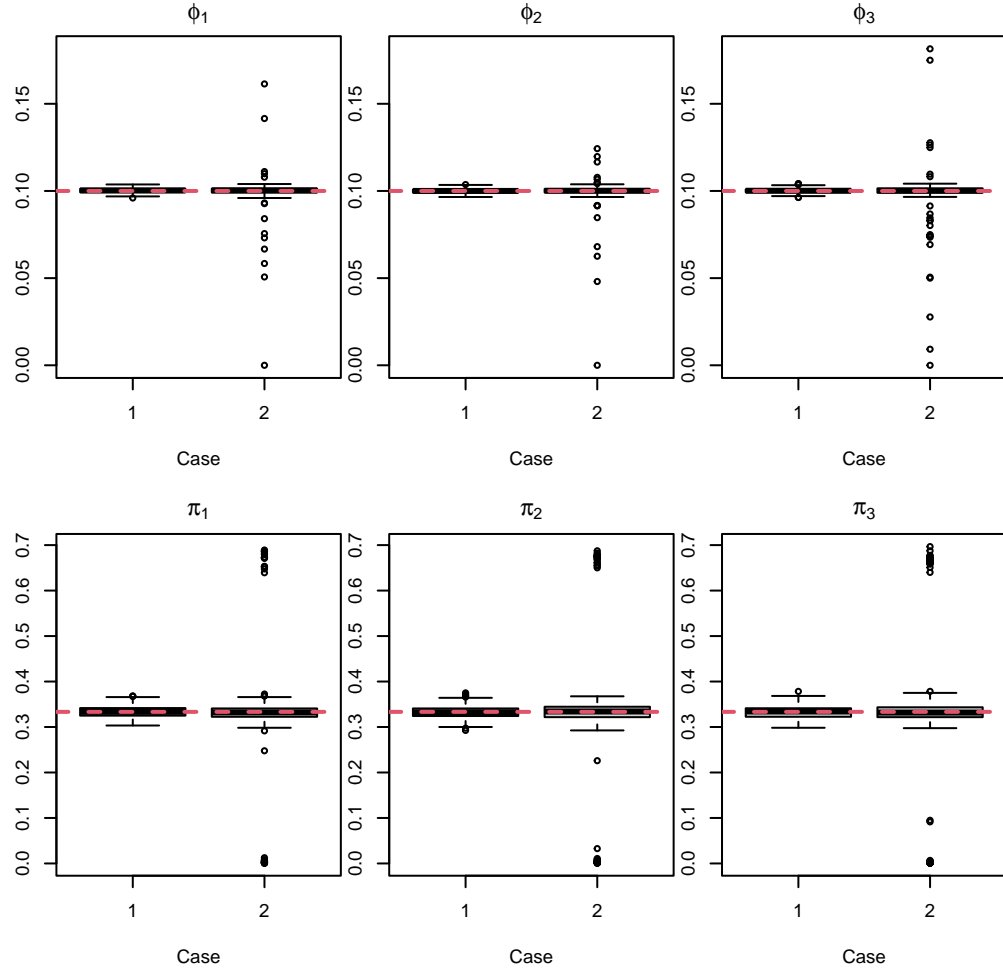

**Figure 31: ZIP mixture model without covariates. Scenario 3:** Boxplots for the estimates of  $\phi_k$  (*top row*) and  $\pi_k$  (*bottom row*), for  $k = 1, \dots, 3$  obtained using the proposed EM algorithm across the datasets simulated from the settings described in Table 48. Red lines correspond to true values. See also Tables 49 and 50.

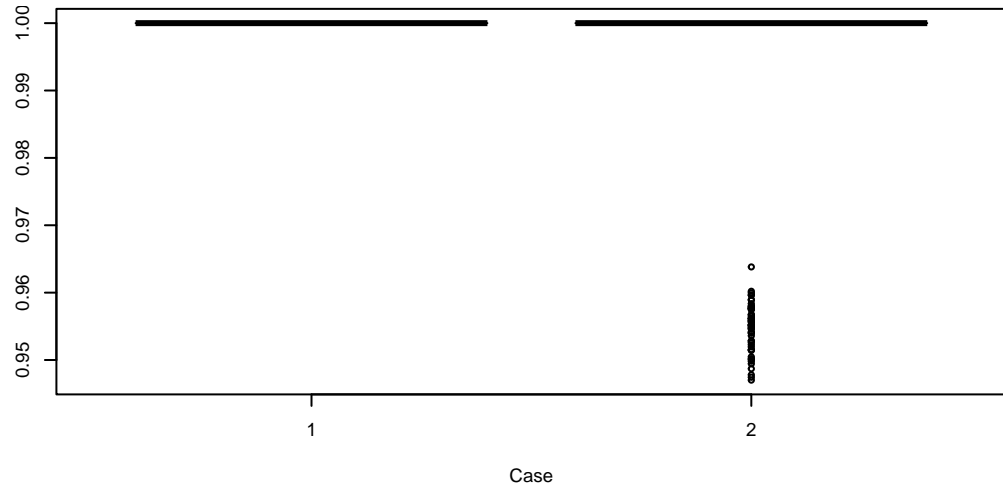

**Figure 32: Scenario 4:** Boxplots for the V-measures of the clustering obtained by the EM algorithm across the datasets simulated from the settings described in Table 48.

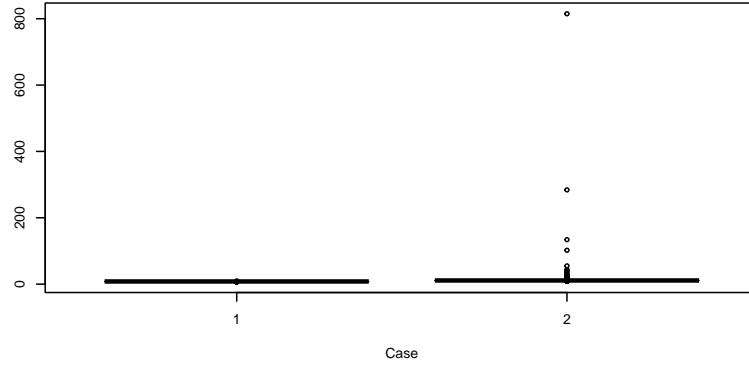

**Figure 33: Scenario 4:** Boxplots for the number of iterations until the EM algorithm converged across the datasets simulated from the settings described in Table 48. See also Table 53.

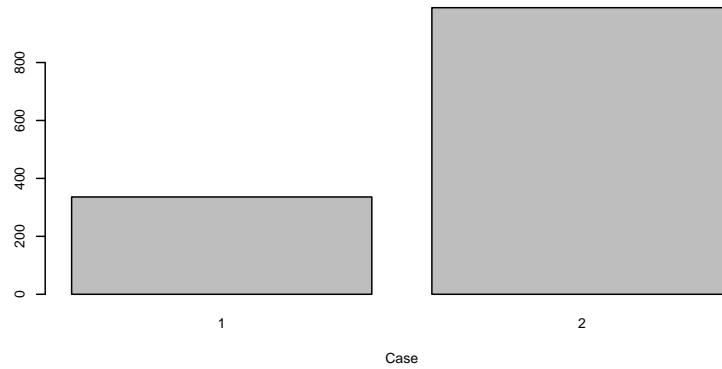

**Figure 34: Scenario 4:** Bar plot for the total computing times, in seconds, taken for the EM algorithm to converge across the datasets simulated from the settings described in Table 48. See also Table 54.

**Table 50: Scenario 4:** Mean and standard deviation (SD) for the estimates of  $\pi_k$  for each  $k$  and each case, obtained using the EM algorithm across the datasets simulated from the settings described in Table 48.

| $\pi_k$ | Case | Mean    | SD      |
|---------|------|---------|---------|
| $\pi_1$ | 1    | 0.33444 | 0.01317 |
|         | 2    | 0.33124 | 0.11683 |
| $\pi_2$ | 1    | 0.33255 | 0.01399 |
|         | 2    | 0.33474 | 0.12418 |
| $\pi_3$ | 1    | 0.33301 | 0.01327 |
|         | 2    | 0.33403 | 0.14037 |

**Table 51: Scenario 4:** Median absolute deviation for the estimates of  $\rho_{gk}$  for each  $k$  and each case, using the EM algorithm across the datasets simulated from the settings described in Table 48.

| $k$ | Case    |         |
|-----|---------|---------|
|     | 1       | 2       |
| 1   | 0.01026 | 0.59934 |
| 2   | 0.01005 | 0.59589 |
| 3   | 0.01009 | 0.60201 |

**Table 52: Scenario 4:** Median absolute deviation for the estimates of  $\beta_{0_g}$  for each case, using the EM algorithm across the datasets simulated from the settings described in Table 48.

| Case    |         |
|---------|---------|
| 1       | 2       |
| 0.00707 | 0.00949 |

**Table 53: Scenario 4:** Mean and standard deviation (SD) for the number of iterations until the EM algorithm converged, by case, across the datasets simulated from the settings described in Table 48.

| Case | Mean     | SD       |
|------|----------|----------|
| 1    | 7.96875  | 0.21466  |
| 2    | 17.14844 | 53.90989 |

**Table 54: Scenario 4:** Mean and standard deviation (SD) for the EM algorithm computing times, in seconds, by case, across the datasets simulated from the settings described in Table 48.

| Case | Mean    | SD      |
|------|---------|---------|
| 1    | 1.31225 | 0.07914 |
| 2    | 3.86476 | 8.52394 |

### 1.4.5 Scenario 5

For this scenario, we use  $K = 2$  clusters, and rather than using the equal cluster assignment probabilities, we use different values for these probabilities. The setting for this scenario is shown in Table 55.

As demonstrated in Tables 56 and 57 and Figure 35 the estimated probabilities of  $\phi_k$  and  $\pi_k$  are close to their true values. From Table 56 and Figure 35, for the probabilities of always zero estimates ( $\phi_k$ ), we can see that the standard deviations for the first cluster increase in each case, but remain almost the same for the second cluster. For the estimates of  $\pi_k$ , the standard deviations are almost the same and small enough in all cases (Table 57 and Figure 35). According to the MSE results (see Tables 58 and 59), the estimates of  $\rho_{gk}$  and  $\beta_{0g}$  are close to their true values, and when the clusters are more unbalanced, the MSEs become a bit larger for both estimates. Also, the V-measures in all the cases are one or very close to one. The number of iterations is equal to 9 for all cases (Table 60 and Figure 36), and the computation time is the same for all cases (Table 61 and Figure 37)

**Table 55: ZIP mixture model with a size factor. Scenario 5:** Values chosen for the proportion assigned to each cluster  $\pi_k$  in each case along with the fixed parameters used to simulate the datasets. Note that  $\pi_2 = 1 - \pi_1$ .

| Case | $N$  | $G$ | $K$ | $\phi_k$ | $\pi_1$ | $\pi_2$ |
|------|------|-----|-----|----------|---------|---------|
| 1    | 1200 | 120 | 2   | 0.1      | 0.50    | 0.50    |
| 2    |      |     |     |          | 0.25    | 0.75    |
| 3    |      |     |     |          | 0.10    | 0.90    |
| 4    |      |     |     |          | 0.05    | 0.95    |

**Table 56: Scenario 5:** Mean and standard deviation (SD) for the estimates of  $\phi_k$  for each  $k$  and each case, obtained using the EM algorithm across the datasets simulated from the settings described in Table 55.

| $\phi_k$ | Case | Mean    | SD      |
|----------|------|---------|---------|
| $\phi_1$ | 1    | 0.10027 | 0.00116 |
|          | 2    | 0.10024 | 0.00158 |
|          | 3    | 0.10029 | 0.00271 |
|          | 4    | 0.10041 | 0.00342 |
| $\phi_2$ | 1    | 0.10015 | 0.00110 |
|          | 2    | 0.10019 | 0.00094 |
|          | 3    | 0.10023 | 0.00085 |
|          | 4    | 0.10031 | 0.00082 |

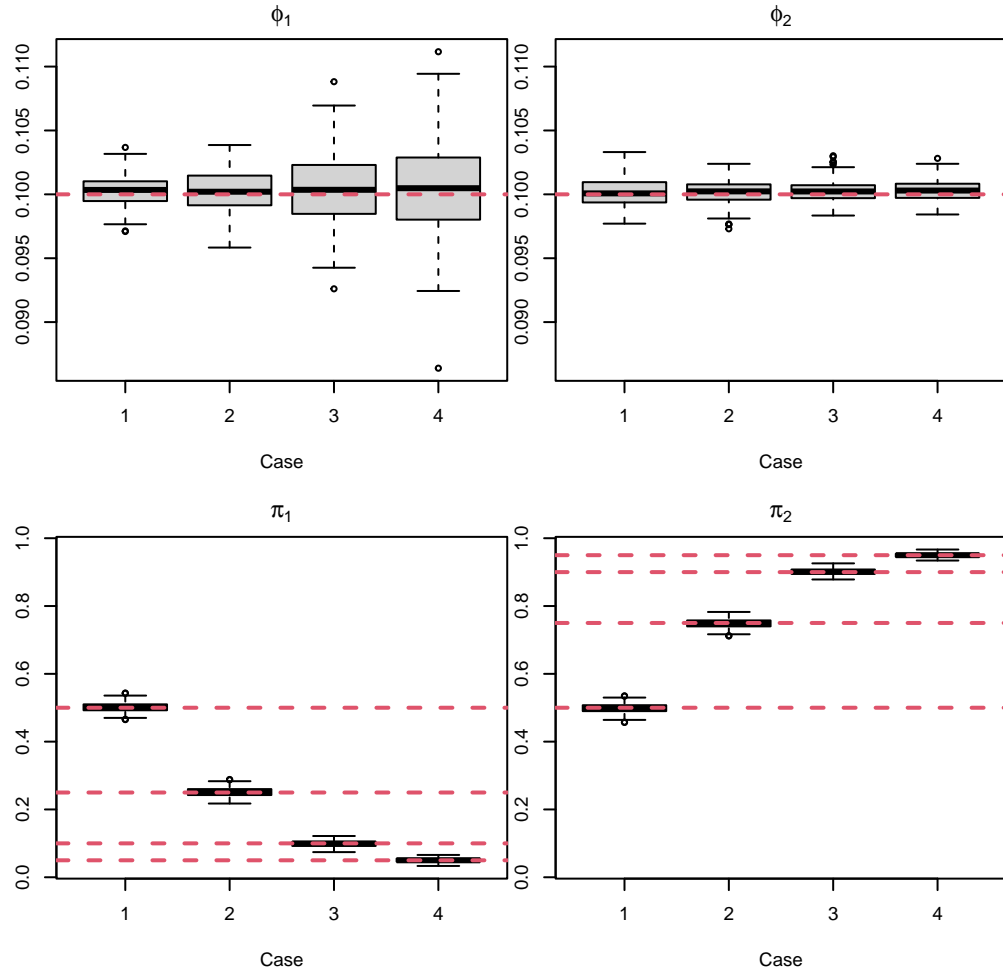

**Figure 35: ZIP mixture model without covariates. Scenario 3:** Boxplots for the estimates of  $\phi_k$  (*top row*) and  $\pi_k$  (*bottom row*), for  $k = 1, 2$  obtained using the proposed EM algorithm across the datasets simulated from the settings described in Table 55. Red lines correspond to true values. See also Tables 56 and 57.

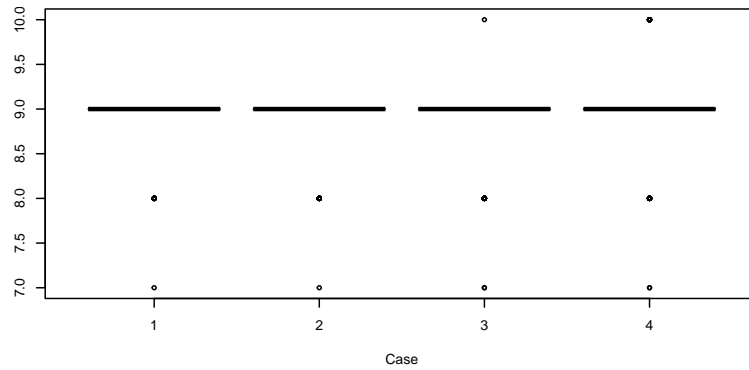

**Figure 36: Scenario 5:** Boxplots for the number of iterations until the EM algorithm converged across the datasets simulated from the settings described in Table 55. See also Table 60.

**Table 57: Scenario 5:** Mean and standard deviation (SD) for the estimates of  $\pi_k$  for each  $k$  and each case, obtained using the EM algorithm across the datasets simulated from the settings described in Table 55.

| $\pi_k$ | Case | Mean    | SD      |
|---------|------|---------|---------|
| $\pi_1$ | 1    | 0.50042 | 0.01393 |
|         | 2    | 0.25139 | 0.01278 |
|         | 3    | 0.09914 | 0.00900 |
|         | 4    | 0.05029 | 0.00618 |
| $\pi_2$ | 1    | 0.49958 | 0.01393 |
|         | 2    | 0.74861 | 0.01278 |
|         | 3    | 0.90086 | 0.00900 |
|         | 4    | 0.94971 | 0.00618 |

**Table 58: Scenario 5:** Mean squared error for the estimates of  $\rho_{gk}$  for each  $k$  and each case, using the EM algorithm across the datasets simulated from the settings described in Table 55.

| $k$ | Case        |             |             |             |
|-----|-------------|-------------|-------------|-------------|
|     | 1           | 2           | 3           | 4           |
| 1   | 0.000128601 | 0.000168903 | 0.000335283 | 0.000650272 |
| 2   | 0.000128601 | 0.000168903 | 0.000335283 | 0.000650272 |

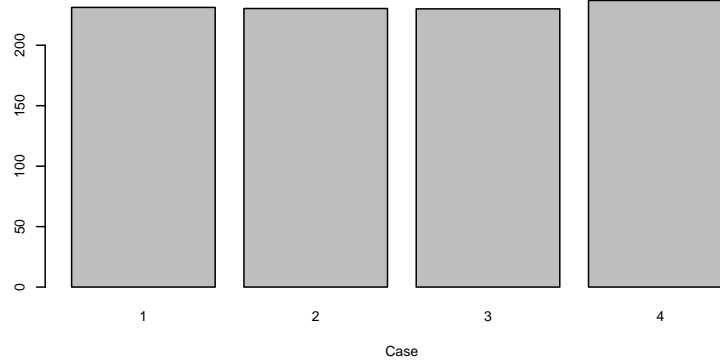

**Figure 37: Scenario 5:** Bar plot for the total computing times, in seconds, taken for the EM algorithm to converge across the datasets simulated from the settings described in Table 55. See also Table 61.

**Table 59: Scenario 5:** Mean squared error for the estimates of  $\beta_{0g}$  for each case, using the EM algorithm across the datasets simulated from the settings described in Table 55.

| Case    |         |         |         |
|---------|---------|---------|---------|
| 1       | 2       | 3       | 4       |
| 0.00012 | 0.00016 | 0.00032 | 0.00063 |

**Table 60: Scenario 5:** Mean and standard deviation (SD) for the number of iterations until the EM algorithm converged, by case, across the datasets simulated from the settings described in Table 55.

| Case | Mean    | SD      |
|------|---------|---------|
| 1    | 8.89062 | 0.32502 |
| 2    | 8.89844 | 0.31535 |
| 3    | 8.86328 | 0.37685 |
| 4    | 8.95703 | 0.38870 |

**Table 61: Scenario 5:** Mean and standard deviation (SD) for the EM algorithm computing times, in seconds, by case, across the datasets simulated from the settings described in Table 55.

| Case | Mean    | SD      |
|------|---------|---------|
| 1    | 0.90346 | 0.06764 |
| 2    | 0.89992 | 0.06433 |
| 3    | 0.89883 | 0.06407 |
| 4    | 0.92589 | 0.06959 |

#### 1.4.6 Scenario 6

For this scenario, the probability of always zero varies between different cases to see their effects on parameter estimation. We start from a very small probability of always zero (5%) to a large one (90%) across  $K = 3$  clusters. All other parameters and hyperparameters are kept fixed and the setting for this scenario can be seen in Table 62.

According to Tables 63 and 64 and Figure 38, the estimates of  $\pi_k$  and  $\phi_k$  are all close to their true values and have almost the same standard deviations for all cases. The only thing is that the standard deviations have a little increase in some cases when there is a larger probability of always zero. We should note that in Figure 38 for cases 1 to 5, the estimates of  $\phi_1$ ,  $\phi_2$ , and  $\phi_3$  are all merged into one vector to demonstrate their behaviour better. Again, the V-measures are mostly close to one except for some misclassifications in case 5 (Figure 39). Also, the estimates of the parameters  $\beta_{0g}$  and  $\rho_{gk}$  have small MSEs that show their proximity to the true values (Tables 65 and 66). The number of iterations is almost the same, except for case 5, which has always zero proportions of 90% (Table 67 and Figure 40). The computational time is almost the same across the cases except for case 4, which is faster compared to the other cases (Table 68 and Figure 41).

**Table 62: ZIP mixture model with a size factor. Scenario 6:** Values chosen for the probability of always-zero in the ZIP distribution  $\phi_k$  in each case along with the fixed parameters used to simulate the datasets.

| Case | $N$  | $G$ | $K$ | $\phi_k$           | $\pi_k$ |
|------|------|-----|-----|--------------------|---------|
| 1    | 1200 | 120 | 3   | 0.05               | $1/K$   |
| 2    |      |     |     | 0.10               |         |
| 3    |      |     |     | 0.25               |         |
| 4    |      |     |     | 0.50               |         |
| 5    |      |     |     | 0.90               |         |
| 6    |      |     |     | (0.05, 0.25, 0.50) |         |

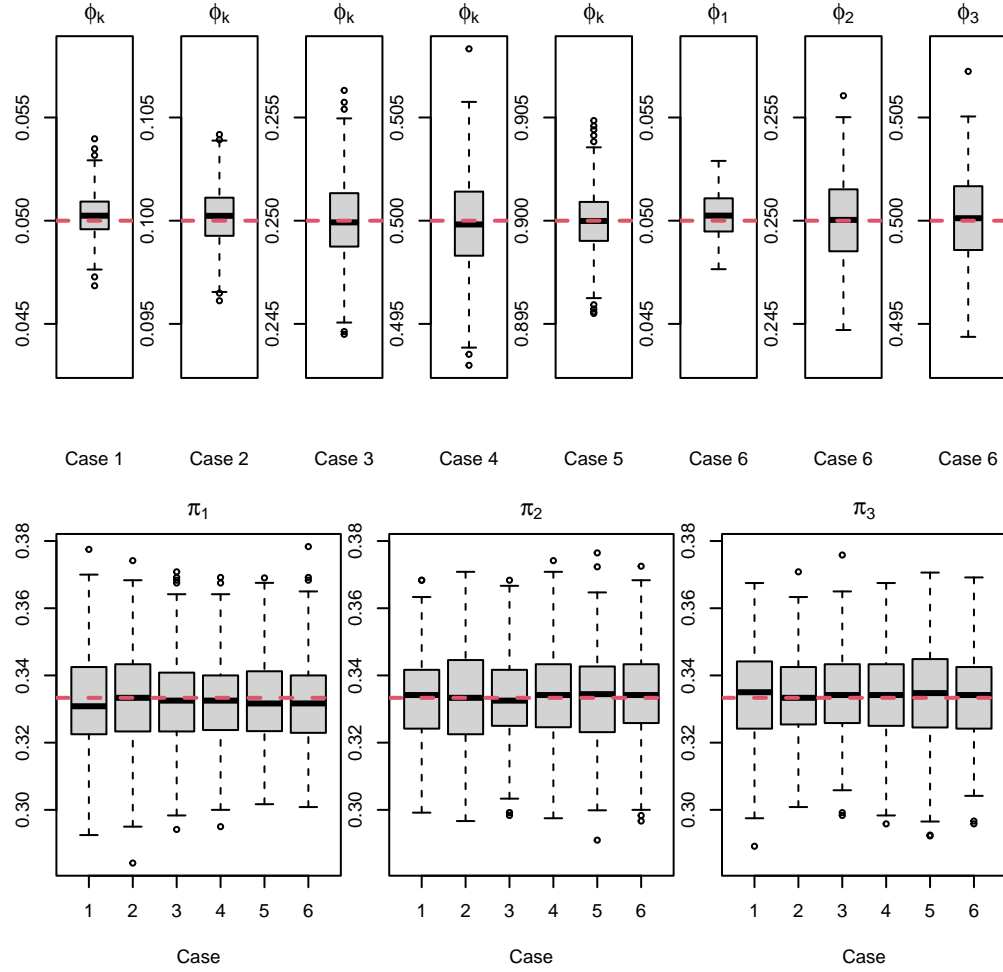

**Figure 38: ZIP mixture model without covariates. Scenario 3:** Boxplots for the estimates of  $\phi_k$  (top row) and  $\pi_k$  (bottom row), for  $k = 1, \dots, 3$  obtained using the proposed EM algorithm across the datasets simulated from the settings described in Table 62. Red lines correspond to true values. See also Tables 63 and 64.

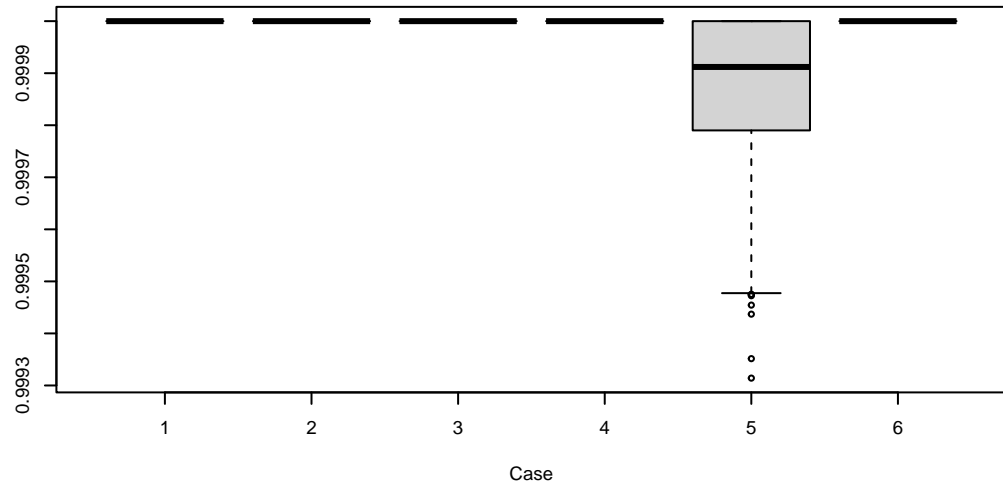

**Figure 39: Scenario 6:** Boxplots for the V-measures of the clustering obtained by the EM algorithm across the datasets simulated from the settings described in Table 62.

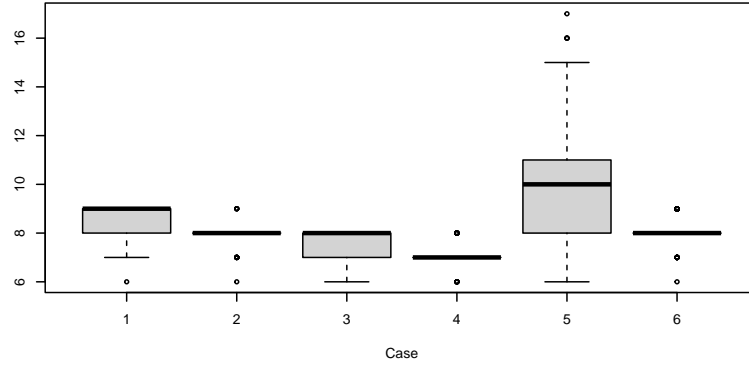

**Figure 40: Scenario 6:** Boxplots for the number of iterations until the EM algorithm converged across the datasets simulated from the settings described in Table 62. See also Table 67.

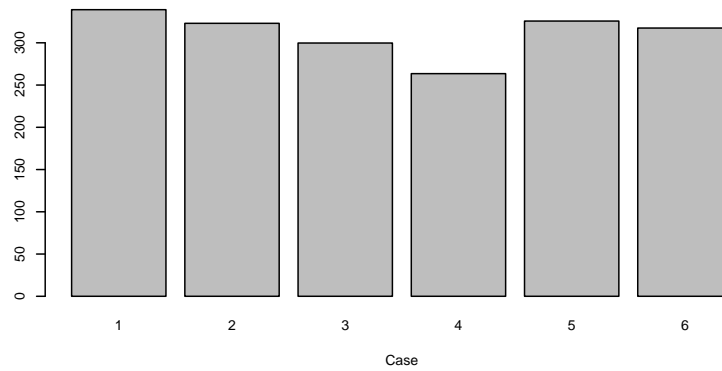

**Figure 41: Scenario 6:** Bar plot for the total computing times, in seconds, taken for the EM algorithm to converge across the datasets simulated from the settings described in Table 62. See also Table 68.

**Table 63: Scenario 6:** Mean and standard deviation (SD) for the estimates of  $\phi_k$  for each  $k$  and each case, obtained using the EM algorithm across the datasets simulated from the settings described in Table 62.

| $\phi_k$ | Case | Mean    | SD      |
|----------|------|---------|---------|
| $\phi_1$ | 1    | 0.05023 | 0.00098 |
|          | 2    | 0.10026 | 0.00140 |
|          | 3    | 0.25009 | 0.00189 |
|          | 4    | 0.49992 | 0.00229 |
|          | 5    | 0.89997 | 0.00148 |
|          | 6    | 0.05027 | 0.00107 |
| $\phi_2$ | 1    | 0.05030 | 0.00100 |
|          | 2    | 0.10006 | 0.00139 |
|          | 3    | 0.25006 | 0.00190 |
|          | 4    | 0.49978 | 0.00225 |
|          | 5    | 0.90002 | 0.00145 |
|          | 6    | 0.25001 | 0.00213 |
| $\phi_3$ | 1    | 0.05024 | 0.00092 |
|          | 2    | 0.10024 | 0.00138 |
|          | 3    | 0.24992 | 0.00189 |
|          | 4    | 0.49989 | 0.00218 |
|          | 5    | 0.89991 | 0.00131 |
|          | 6    | 0.50008 | 0.00220 |

**Table 64: Scenario 6:** Mean and standard deviation (SD) for the estimates of  $\pi_k$  for each  $k$  and each case, obtained using the EM algorithm across the datasets simulated from the settings described in Table 62.

| $\pi_k$ | Case | Mean    | SD      |
|---------|------|---------|---------|
| $\pi_1$ | 1    | 0.33265 | 0.01449 |
|         | 2    | 0.33349 | 0.01426 |
|         | 3    | 0.33261 | 0.01366 |
|         | 4    | 0.33217 | 0.01318 |
|         | 5    | 0.33227 | 0.01349 |
|         | 6    | 0.33193 | 0.01300 |
| $\pi_2$ | 1    | 0.33333 | 0.01331 |
|         | 2    | 0.33320 | 0.01513 |
|         | 3    | 0.33305 | 0.01295 |
|         | 4    | 0.33402 | 0.01395 |
|         | 5    | 0.33364 | 0.01422 |
|         | 6    | 0.33457 | 0.01296 |
| $\pi_3$ | 1    | 0.33401 | 0.01417 |
|         | 2    | 0.33331 | 0.01346 |
|         | 3    | 0.33434 | 0.01354 |
|         | 4    | 0.33381 | 0.01388 |
|         | 5    | 0.33409 | 0.01511 |
|         | 6    | 0.33351 | 0.01314 |

**Table 65: Scenario 6:** Mean squared error for the estimates of  $\rho_{gk}$  for each  $k$  and each case, using the EM algorithm across the datasets simulated from the settings described in Table 62.

| $k$ | Case        |             |             |             |             |             |
|-----|-------------|-------------|-------------|-------------|-------------|-------------|
|     | 1           | 2           | 3           | 4           | 5           | 6           |
| 1   | 0.000226465 | 0.000237206 | 0.000281781 | 0.000417185 | 0.002150195 | 0.000264188 |
| 2   | 0.000228237 | 0.000235153 | 0.000278374 | 0.000419742 | 0.002098454 | 0.000294226 |
| 3   | 0.000221568 | 0.000234383 | 0.000277740 | 0.000411982 | 0.002113181 | 0.000357756 |

**Table 66: Scenario 6:** Mean squared error for the estimates of  $\beta_{0g}$  for each case, using the EM algorithm across the datasets simulated from the settings described in Table 62.

| Case    |         |         |         |         |         |
|---------|---------|---------|---------|---------|---------|
| 1       | 2       | 3       | 4       | 5       | 6       |
| 0.00011 | 0.00011 | 0.00013 | 0.00020 | 0.00106 | 0.00015 |

**Table 67: Scenario 6:** Mean and standard deviation (SD) for the number of iterations until the EM algorithm converged, by case, across the datasets simulated from the settings described in Table 62.

| Case | Mean    | SD      |
|------|---------|---------|
| 1    | 8.51172 | 0.55999 |
| 2    | 7.96875 | 0.27830 |
| 3    | 7.60547 | 0.50547 |
| 4    | 7.01562 | 0.27962 |
| 5    | 9.84375 | 2.05393 |
| 6    | 8.10547 | 0.55361 |

**Table 68: Scenario 6:** Mean and standard deviation (SD) for the EM algorithm computing times, in seconds, by case, across the datasets simulated from the settings described in Table 62.

| Case | Mean    | SD      |
|------|---------|---------|
| 1    | 1.32499 | 0.11500 |
| 2    | 1.26188 | 0.09447 |
| 3    | 1.17087 | 0.10087 |
| 4    | 1.02929 | 0.08939 |
| 5    | 1.27236 | 0.30302 |
| 6    | 1.24007 | 0.12507 |

## 1.5 Simulation results for the ZIP mixture model with a covariate

In this section, we simulate data from the zero-inflated Poisson mixture model (as described in Section 2.1.2) when we have a cell-specific size factor ( $T_n$ ), the cluster effects ( $\rho_{gk}$ ), the baseline expression ( $\beta_{0g}$ ), and include a covariate  $x_{n1}$ , for  $n = 1, \dots, N$ . For this model, we simulate  $x_{n1}$  from a Bernoulli distribution with a 0.5 probability of success. We consider two scenarios. In scenario 1, we vary  $N$  (the number of cells) while fixing  $G$  (the number of genes) and all other parameters and hyperparameters. For scenario 2, we vary  $G$ , while  $N$  and all other parameters and hyperparameters are kept fixed. We simulate  $S = 100$  datasets for all cases in each scenario. The parameters that we use to simulate data include:

- Number of clusters:  $K = 2$ .
- Probability of cluster assignments:  $\pi_1 = \pi_2 = 0.5$ .
- Probability of always zero in each cluster:  $\phi_1 = \phi_2 = 0.1$ .
- Baseline expression:  $\beta_{0g} = 0.85$  for all  $g$ .
- Cluster effects:  $\rho_{g1}$ 's =  $(2, -2)$  and  $\rho_{g2}$ 's =  $(-2, 2)$ , in which, for cluster one, the cluster effects on the first half of the genes are 2 and for the remaining half of the genes they are  $-2$  and vice versa for the second cluster.
- Covariate coefficients:  $\beta_{1g} = 1$  for the first half of the genes, and for the remaining half of the genes,  $\beta_{1g} = 0.5$ .
- Size factors:  $T_n$ 's are simulated from a normal distribution with  $\mu = 10$  and  $\sigma = 0.5$ .

### 1.5.1 Scenario 1

As mentioned in the previous paragraph, for this scenario, we consider different  $N$  values while fixing all other parameters and hyperparameters. Table 69 demonstrates the setting for this scenario.

**Table 69: ZIP mixture model with a covariate. Scenario 1:** Values chosen for the number of observations  $N$  in each case along with the fixed parameters used to simulate the datasets.

| Case | $N$  | $G$ | $K$ | $\phi_k$ | $\pi_k$ |
|------|------|-----|-----|----------|---------|
| 1    | 60   |     |     |          |         |
| 2    | 120  |     |     |          |         |
| 3    | 300  | 120 | 2   | 0.1      | $1/K$   |
| 4    | 600  |     |     |          |         |
| 5    | 1200 |     |     |          |         |

For the probabilities of cluster assignments ( $\pi_k$ ) and the probabilities of always zero ( $\phi_k$ ), respectively, as can be seen from Tables 70 and 71 and Figure 42, the resulting estimates get closer to their true values and as  $N$  increases and the standard deviation of these estimates decreases as  $N$  increases, as expected. We also calculate the MADs of the other parameters, including  $\beta_{0g}$ ,  $\beta_{1g}$ , and  $\rho_{gk}$  across all genes and all the simulated datasets. As shown in Tables 72 and 73, the MADs are small, which shows the closeness of these estimates to their true values. In addition, as  $N$  increases, the MAD values decrease, as expected by the convergence properties of the EM algorithm. The computing time increases when  $N$  increases (Table 74 and Figure 43) and V-measures are all one, which shows a perfect match between inferred and true cluster assignments.

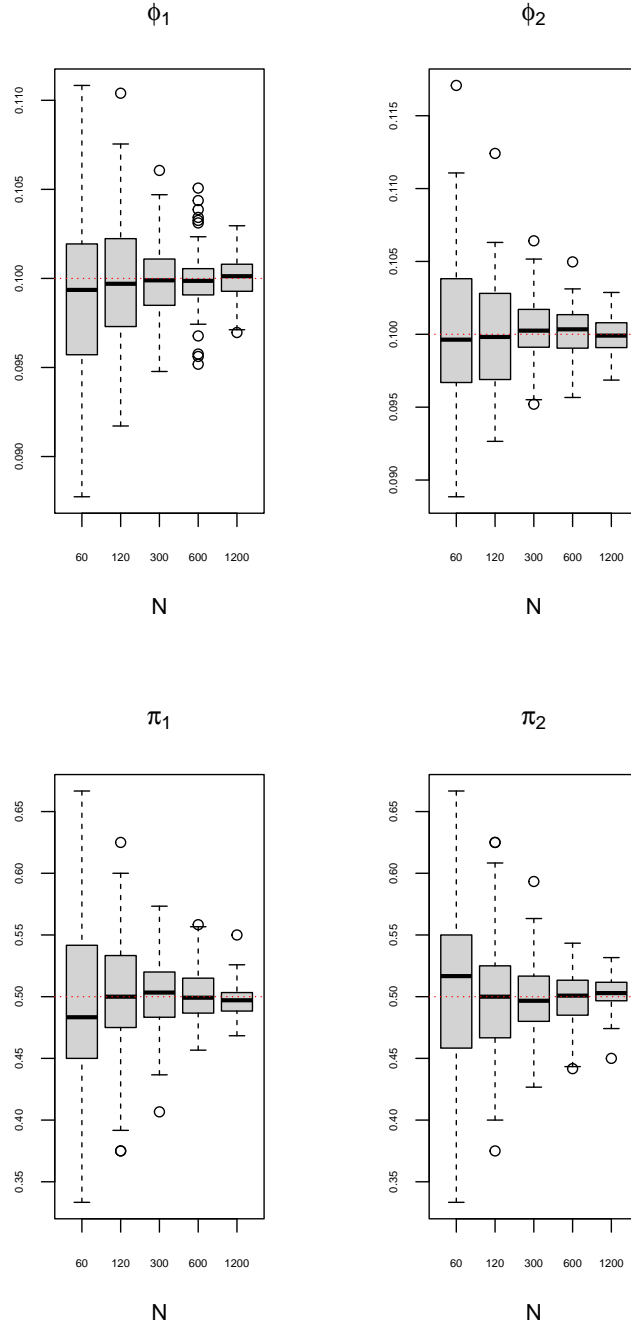

**Figure 42: ZIP mixture model without covariates. Scenario 3:** Boxplots for the estimates of  $\phi_k$  (*top row*) and  $\pi_k$  (*bottom row*), for  $k = 1, 2$  obtained using the proposed EM algorithm across the datasets simulated from the settings described in Table 69. Red lines correspond to true values. See also Tables 70 and 71.

**Table 70: Scenario 1:** Mean and standard deviation (SD) for the estimates of  $\pi_k$  for each  $k$  and each case, obtained using the EM algorithm across the datasets simulated from the settings described in Table 69.

| $k$ | $N$  | Mean        | SD          |
|-----|------|-------------|-------------|
| 1   | 60   | 0.491500000 | 0.065798002 |
|     | 120  | 0.498166667 | 0.049585544 |
|     | 300  | 0.499666667 | 0.029188424 |
|     | 600  | 0.501066667 | 0.019969843 |
|     | 1200 | 0.497058333 | 0.013312513 |
| 2   | 60   | 0.508500000 | 0.065798002 |
|     | 120  | 0.501833333 | 0.049585544 |
|     | 300  | 0.500333333 | 0.029188424 |
|     | 600  | 0.498933333 | 0.019969843 |
|     | 1200 | 0.502941667 | 0.013312513 |

**Table 71: Scenario 1:** Mean and standard deviation (SD) for the estimates of  $\phi_k$  for each  $k$  and each case, obtained using the EM algorithm across the datasets simulated from the settings described in Table 69.

| $k$ | $N$  | Mean        | SD          |
|-----|------|-------------|-------------|
| 1   | 60   | 0.098992456 | 0.005007809 |
|     | 120  | 0.099832251 | 0.003744747 |
|     | 300  | 0.099809984 | 0.002182312 |
|     | 600  | 0.099899911 | 0.001649528 |
|     | 1200 | 0.099991528 | 0.001203047 |
| 2   | 60   | 0.100149594 | 0.005226926 |
|     | 120  | 0.099848961 | 0.003716596 |
|     | 300  | 0.100306134 | 0.002214400 |
|     | 600  | 0.100145810 | 0.001825143 |
|     | 1200 | 0.100001481 | 0.001173997 |

**Table 72: Scenario 1:** MAD for the estimates of  $\rho_{gk}$  for each  $k$  and each  $N$ , using the EM algorithm across the datasets simulated from the settings described in Table 69.

| $k$ | $N$         |             |             |             |             |
|-----|-------------|-------------|-------------|-------------|-------------|
|     | 60          | 120         | 300         | 600         | 1200        |
| 1   | 0.038813812 | 0.026580682 | 0.016910423 | 0.011647520 | 0.008494867 |
| 2   | 0.035358002 | 0.024422462 | 0.015716372 | 0.010928285 | 0.007832469 |

**Table 73: Scenario 1:** MAD for the estimates of  $\beta_{0g}$  and  $\beta_{1g}$  for each  $N$ , using the EM algorithm across the datasets simulated from the settings described in Table 69.

|              | $N$         |             |             |             |             |
|--------------|-------------|-------------|-------------|-------------|-------------|
|              | 60          | 120         | 300         | 600         | 1200        |
| $\beta_{0g}$ | 0.014636945 | 0.010251386 | 0.006453585 | 0.004745225 | 0.003249015 |
| $\beta_{1g}$ | 0.016953099 | 0.011994497 | 0.007652635 | 0.005360614 | 0.003791324 |

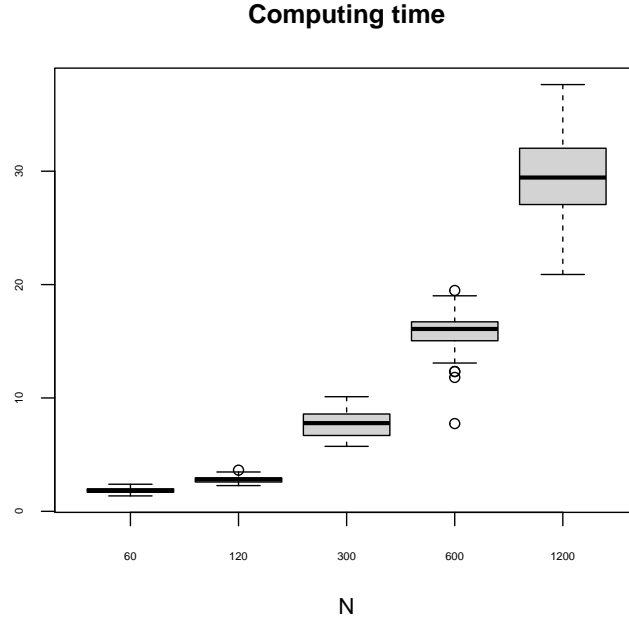

**Figure 43: Scenario 1:** Bar plot for the total computing times, in seconds, taken for the EM algorithm to converge across the datasets simulated from the settings described in Table 69. See also Table 74.

**Table 74: Scenario 1:** Mean and standard deviation (SD) for the EM algorithm computing times, in seconds, by  $K$ , across the datasets simulated from the settings described in Table 69.

| $N$  | Mean  | SD   |
|------|-------|------|
| 60   | 1.84  | 0.21 |
| 120  | 2.80  | 0.27 |
| 300  | 7.72  | 1.15 |
| 600  | 15.80 | 1.64 |
| 1200 | 29.46 | 3.03 |

### 1.5.2 Scenario 2

For this scenario, by fixing  $N = 1200$  and all other parameters and hyperparameters, the number of genes varies according to the settings in Table 75.

**Table 75: ZIP mixture model with a covariate. Scenario 2:** Values chosen for the number of genes  $G$  in each case along with the fixed parameters used to simulate the datasets.

| Case | $N$  | $G$  | $K$ | $\phi_k$ | $\pi_k$ |
|------|------|------|-----|----------|---------|
| 1    | 1200 | 12   | 2   | 0.1      | $1/K$   |
| 2    |      | 60   |     |          |         |
| 3    |      | 120  |     |          |         |
| 4    |      | 600  |     |          |         |
| 5    |      | 1500 |     |          |         |

In this scenario, the estimates of  $\pi_k$ 's (probability of cluster assignments), are close to their true values, but their standard deviations remain somewhat the same while  $G$  increases (Table 76 and Figure 44). For the probability of always zero, we can observe from Table 77 and Figure 44 that the resulting estimates are close to their true values and the standard deviations decrease as  $G$  increases. For other parameter estimates, including  $\beta_{0g}$ ,  $\beta_{1g}$ , and  $\rho_{gk}$  from Tables 78 and 79, the MADs remain almost the same when the number of genes increases as  $N$  remains fixed. The V-measures are equal to one in all cases. As expected, the computing time increases when  $G$  increases, particularly for the largest one when  $G = 1500$  (Table 80 and Figure 45).

**Table 76: Scenario 2:** Mean and standard deviation (SD) for the estimates of  $\pi_k$  for each  $k$  and each  $G$ , obtained using the EM algorithm across the datasets simulated from the settings described in Table 75.

| $k$ | $G$  | Mean        | SD          |
|-----|------|-------------|-------------|
| 1   | 12   | 0.499675000 | 0.014990127 |
|     | 60   | 0.499125000 | 0.012900908 |
|     | 120  | 0.499216667 | 0.014080407 |
|     | 600  | 0.503308333 | 0.014740771 |
|     | 1500 | 0.499600000 | 0.014515405 |
| 2   | 12   | 0.500325000 | 0.014990127 |
|     | 60   | 0.500875000 | 0.012900908 |
|     | 120  | 0.500783333 | 0.014080407 |
|     | 600  | 0.496691667 | 0.014740771 |
|     | 1500 | 0.500400000 | 0.014515405 |

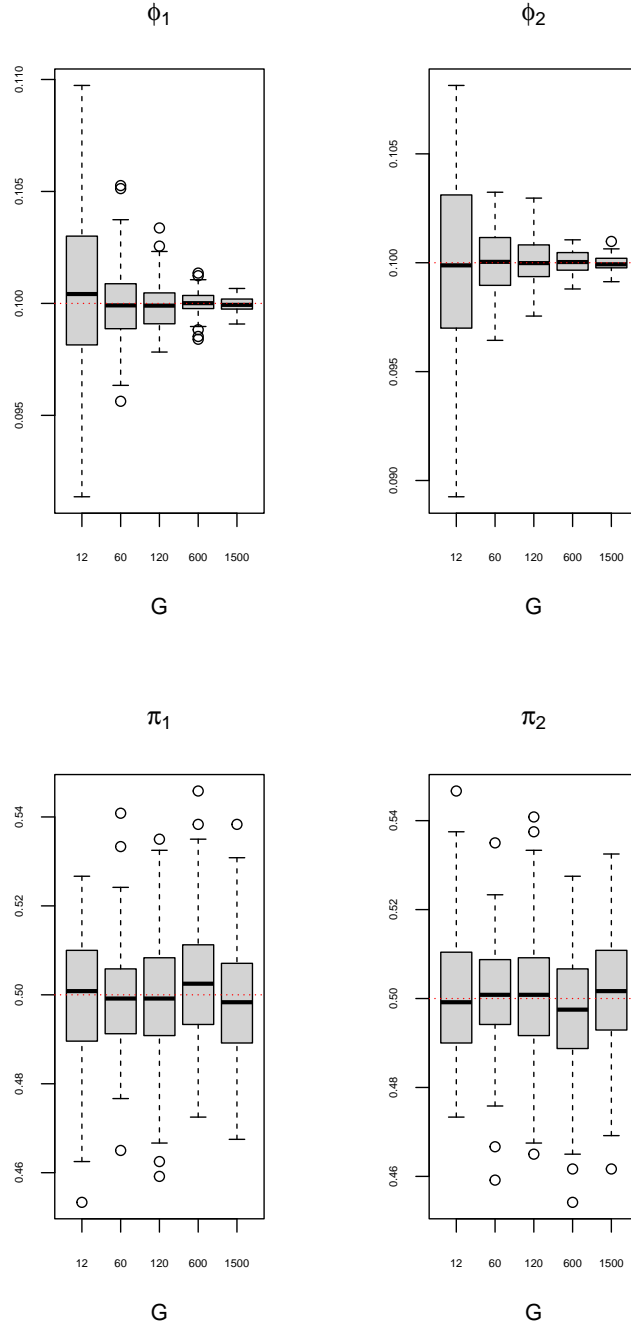

**Figure 44: ZIP mixture model without covariates. Scenario 3:** Boxplots for the estimates of  $\phi_k$  (*top row*) and  $\pi_k$  (*bottom row*), for  $k = 1, 2$  obtained using the proposed EM algorithm across the datasets simulated from the settings described in Table 75. Red lines correspond to true values. See also Tables 76 and 77.

**Table 77: Scenario 2:** Mean and standard deviation (SD) for the estimates of  $\phi_k$  for each  $k$  and each case, obtained using the EM algorithm across the datasets simulated from the settings described in Table 75.

| $k$ | $G$  | Mean        | SD          |
|-----|------|-------------|-------------|
| 1   | 12   | 0.100470497 | 0.003632417 |
|     | 60   | 0.099988024 | 0.001694311 |
|     | 120  | 0.099896435 | 0.001094482 |
|     | 600  | 0.100007377 | 0.000554468 |
|     | 1500 | 0.099973886 | 0.000331099 |
| 2   | 12   | 0.099665322 | 0.004176079 |
|     | 60   | 0.099985994 | 0.001601331 |
|     | 120  | 0.100113810 | 0.001070322 |
|     | 600  | 0.100034844 | 0.000530891 |
|     | 1500 | 0.099958600 | 0.000329253 |

**Table 78: Scenario 2:** MAD for the estimates of  $\rho_{gk}$  for each  $k$  and each case, using the EM algorithm across the datasets simulated from the settings described in Table 75.

| $k$ | $G$         |             |             |             |             |
|-----|-------------|-------------|-------------|-------------|-------------|
|     | 12          | 60          | 120         | 600         | 1500        |
| 1   | 0.008111007 | 0.008324391 | 0.008290203 | 0.008281629 | 0.008424692 |
| 2   | 0.008118105 | 0.007922273 | 0.007625036 | 0.007775817 | 0.007789265 |

**Table 79: Scenario 2:** MAD for the estimates of  $\beta_{0g}$  and  $\beta_{1g}$  for each  $G$ , using the EM algorithm across the datasets simulated from the settings described in Table 75.

|              | $G$         |             |             |             |             |
|--------------|-------------|-------------|-------------|-------------|-------------|
|              | 12          | 60          | 120         | 600         | 1500        |
| $\beta_{0g}$ | 0.003424299 | 0.003184400 | 0.003212991 | 0.003321381 | 0.003312820 |
| $\beta_{1g}$ | 0.003699243 | 0.003602925 | 0.003818405 | 0.003781053 | 0.003764123 |

**Table 80: Scenario 2:** Mean and standard deviation (SD) for the EM algorithm computing times, in seconds, by  $K$ , across the datasets simulated from the settings described in Table 75.

| $G$  | Mean    | SD     |
|------|---------|--------|
| 12   | 2.43    | 0.23   |
| 60   | 12.78   | 1.14   |
| 120  | 26.62   | 2.33   |
| 600  | 198.17  | 16.87  |
| 1500 | 1241.09 | 150.62 |

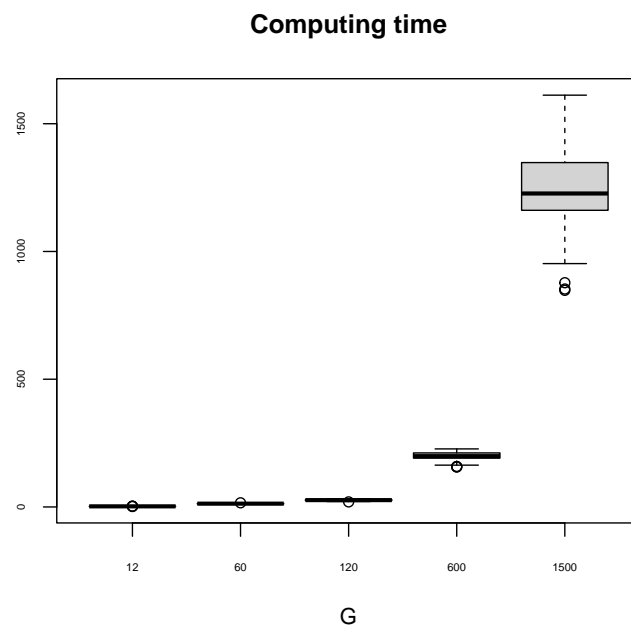

**Figure 45: Scenario 2:** Bar plot for the total computing times, in seconds, taken for the EM algorithm to converge across the simulated datasets. See also Table 80.

## 1.6 Simulation results for the Mixture of ZINB without covariates

### 1.6.1 Scenario 1

**Table 81: Scenario 1:** Mean and standard deviation (SD) for the estimates of  $\pi_k$  for each cluster  $k$  and each  $N$ , obtained using the EM algorithm across the simulated datasets.

| $k$ | $N$  | Mean        | SD          |
|-----|------|-------------|-------------|
| 1   | 60   | 0.502500000 | 0.063712977 |
|     | 120  | 0.499833333 | 0.045643239 |
|     | 300  | 0.499433333 | 0.027784060 |
|     | 600  | 0.499966667 | 0.020996472 |
|     | 1200 | 0.503100000 | 0.014755813 |
| 2   | 60   | 0.497500000 | 0.063712977 |
|     | 120  | 0.500166667 | 0.045643239 |
|     | 300  | 0.500566667 | 0.027784060 |
|     | 600  | 0.500033333 | 0.020996472 |
|     | 1200 | 0.496900000 | 0.014755813 |

**Table 82: Scenario 1:** Mean and standard deviation (SD) for the estimates of  $\phi_k$  for each  $k$  and each case, obtained using the EM algorithm across the simulated datasets.

| $k$ | $N$  | Mean        | SD          |
|-----|------|-------------|-------------|
| 1   | 60   | 0.101422431 | 0.006166323 |
|     | 120  | 0.100564181 | 0.004162313 |
|     | 300  | 0.100183877 | 0.002496634 |
|     | 600  | 0.099694053 | 0.002046551 |
|     | 1200 | 0.100138043 | 0.001312946 |
| 2   | 60   | 0.099817364 | 0.005766071 |
|     | 120  | 0.100215019 | 0.003390551 |
|     | 300  | 0.099439385 | 0.002471910 |
|     | 600  | 0.100079498 | 0.001403623 |
|     | 1200 | 0.099994556 | 0.001015787 |

**Table 83: Scenario 1:** Mean and standard deviation (SD) for the estimates of  $\nu_k$  for each  $k$  and each case, obtained using the EM algorithm across the simulated datasets.

| $k$ | $N$  | Mean  | SD   |
|-----|------|-------|------|
| 1   | 60   | 5.48  | 0.38 |
|     | 120  | 5.26  | 0.23 |
|     | 300  | 5.10  | 0.12 |
|     | 600  | 5.04  | 0.11 |
|     | 1200 | 5.01  | 0.07 |
| 2   | 60   | 23.07 | 2.04 |
|     | 120  | 21.29 | 1.20 |
|     | 300  | 20.36 | 0.74 |
|     | 600  | 20.21 | 0.52 |
|     | 1200 | 20.11 | 0.33 |

**Table 84: Scenario 1:** Mean and standard deviation (SD) for the EM algorithm computing times, in seconds, by  $K$ , across the simulated datasets.

| $N$  | Mean  | SD   |
|------|-------|------|
| 60   | 1.15  | 0.19 |
| 120  | 2.29  | 0.31 |
| 300  | 5.52  | 0.95 |
| 600  | 11.05 | 1.89 |
| 1200 | 22.61 | 3.57 |

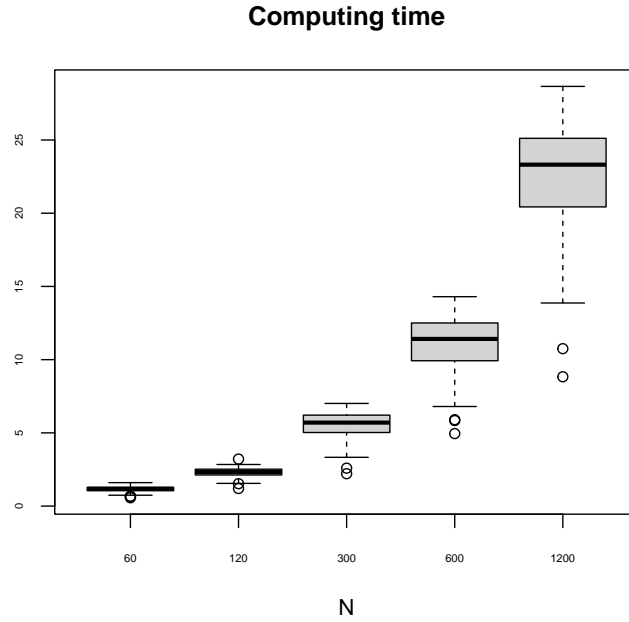

**Figure 46: Scenario 1:** Bar plot for the total computing times, in seconds, taken for the EM algorithm to converge across the simulated datasets. See also Table 84.

### 1.6.2 Scenario 2

**Table 85: Scenario 2:** Mean and standard deviation (SD) for the estimates of  $\pi_k$  for each  $k$  and each case, obtained using the EM algorithm across the simulated datasets.

| $k$ | $G$  | Mean        | SD          |
|-----|------|-------------|-------------|
| 1   | 12   | 0.499719868 | 0.017829928 |
|     | 60   | 0.501075000 | 0.014799110 |
|     | 120  | 0.501675000 | 0.016050257 |
|     | 600  | 0.497741667 | 0.014496940 |
|     | 1500 | 0.500300000 | 0.012287772 |
| 2   | 12   | 0.500280132 | 0.017829928 |
|     | 60   | 0.498925000 | 0.014799110 |
|     | 120  | 0.498325000 | 0.016050257 |
|     | 600  | 0.502258333 | 0.014496940 |
|     | 1500 | 0.499700000 | 0.012287772 |

**Table 86: Scenario 2:** Mean and standard deviation (SD) for the estimates of  $\phi_k$  for each  $k$  and each case, obtained using the EM algorithm across the simulated datasets.

| $k$ | $G$  | Mean        | SD          |
|-----|------|-------------|-------------|
| 1   | 12   | 0.099852809 | 0.004301919 |
|     | 60   | 0.100302132 | 0.002016654 |
|     | 120  | 0.099789100 | 0.001318137 |
|     | 600  | 0.100000309 | 0.000585295 |
|     | 1500 | 0.100004958 | 0.000351525 |
| 2   | 12   | 0.100203671 | 0.003345701 |
|     | 60   | 0.099927764 | 0.001476867 |
|     | 120  | 0.100218634 | 0.001022206 |
|     | 600  | 0.100067091 | 0.000544676 |
|     | 1500 | 0.099958123 | 0.000300695 |

**Table 87: Scenario 2:** Mean and standard deviation (SD) for the estimates of  $\nu_k$  for each  $k$  and each case, obtained using the EM algorithm across the datasets simulated from the settings described in Table ?? across the simulated datasets.

| $k$ | $G$  | Mean    | SD     |
|-----|------|---------|--------|
| 1   | 12   | 4.9981  | 0.1790 |
|     | 60   | 5.0416  | 0.0816 |
|     | 120  | 5.0122  | 0.0732 |
|     | 600  | 5.0186  | 0.0281 |
|     | 1500 | 5.0218  | 0.0222 |
| 2   | 12   | 19.9360 | 1.0668 |
|     | 60   | 20.0507 | 0.4643 |
|     | 120  | 20.1685 | 0.3419 |
|     | 600  | 20.1155 | 0.1467 |
|     | 1500 | 20.1211 | 0.0917 |

**Table 88: Scenario 2:** Mean and standard deviation (SD) for the EM algorithm computing times, in seconds, by  $K$ , across the simulated datasets.

| $G$  | Mean    | SD     |
|------|---------|--------|
| 12   | 6.96    | 1.26   |
| 60   | 33.52   | 6.32   |
| 120  | 54.62   | 9.28   |
| 600  | 256.19  | 46.64  |
| 1500 | 1099.00 | 302.13 |

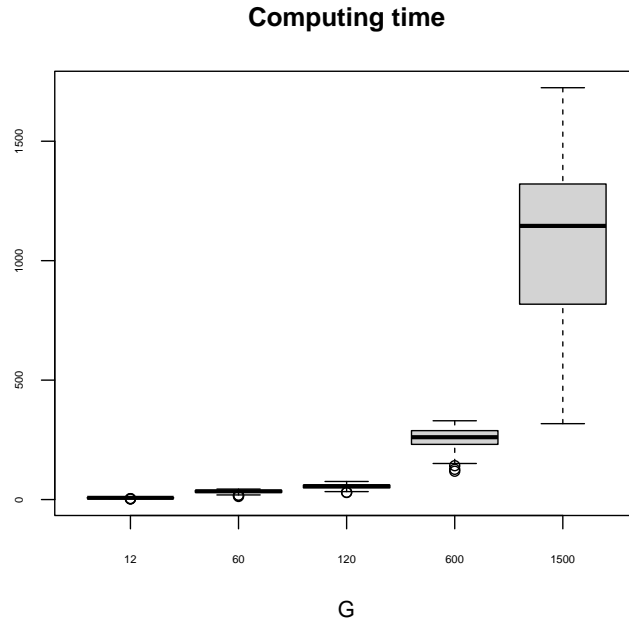

**Figure 47: Scenario 2:** Bar plot for the total computing times, in seconds, taken for the EM algorithm to converge across the simulated datasets. See also Table 88.

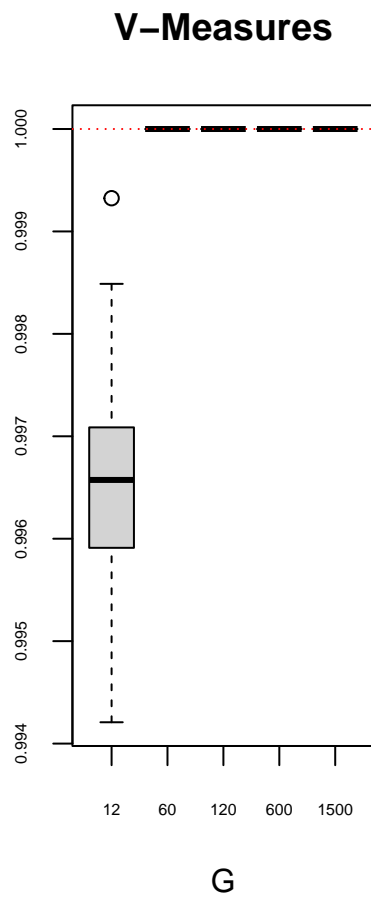

**Figure 48: Scenario 2:** Boxplots for the  $V$ -measures of the clustering obtained by the EM algorithm across the simulated datasets.

## 1.7 Simulation results for the mixture of ZINB with a size factor

### 1.7.1 Scenario 1

**Table 89: Scenario 1:** Mean and standard deviation (SD) for the estimates of  $\pi_k$  for each  $k$  and each  $N$ , obtained using the EM algorithm across the simulated datasets.

| $k$ | $N$  | Mean        | SD          |
|-----|------|-------------|-------------|
| 1   | 60   | 0.499000000 | 0.059403129 |
|     | 120  | 0.499416667 | 0.044274533 |
|     | 300  | 0.499700000 | 0.024989762 |
|     | 600  | 0.496466667 | 0.018173129 |
|     | 1200 | 0.497150000 | 0.012803652 |
| 2   | 60   | 0.501000000 | 0.059403129 |
|     | 120  | 0.500583333 | 0.044274533 |
|     | 300  | 0.500300000 | 0.024989762 |
|     | 600  | 0.503533333 | 0.018173129 |
|     | 1200 | 0.502850000 | 0.012803652 |

**Table 90: Scenario 1:** Mean and standard deviation (SD) for the estimates of  $\phi_k$  for each  $k$  and each  $N$ , obtained using the EM algorithm across the simulated datasets.

| $k$ | $N$  | Mean        | SD          |
|-----|------|-------------|-------------|
| 1   | 60   | 0.098709502 | 0.005962128 |
|     | 120  | 0.099481329 | 0.003898979 |
|     | 300  | 0.099814282 | 0.002657849 |
|     | 600  | 0.099822926 | 0.001770076 |
|     | 1200 | 0.100074985 | 0.001325751 |
| 2   | 60   | 0.198481193 | 0.006203301 |
|     | 120  | 0.199096122 | 0.005127590 |
|     | 300  | 0.200084764 | 0.003133217 |
|     | 600  | 0.200102372 | 0.002030886 |
|     | 1200 | 0.199840261 | 0.001712608 |

**Table 91: Scenario 1:** Mean and standard deviation (SD) for the estimates of  $\nu_k$  for each  $k$  and each  $N$ , obtained using the EM algorithm across the simulated datasets.

| $k$ | $N$  | Mean    | SD     |
|-----|------|---------|--------|
| 1   | 60   | 5.2327  | 0.1597 |
|     | 120  | 5.1426  | 0.1225 |
|     | 300  | 5.0433  | 0.0672 |
|     | 600  | 5.0199  | 0.0461 |
|     | 1200 | 5.0104  | 0.0368 |
| 2   | 60   | 21.1015 | 0.8673 |
|     | 120  | 20.5514 | 0.6456 |
|     | 300  | 20.2056 | 0.3604 |
|     | 600  | 20.0906 | 0.2556 |
|     | 1200 | 20.0455 | 0.1791 |

**Table 92: Scenario 1:** Mean and standard deviation (SD) for the EM algorithm computing times, in seconds, by  $K$ , across the simulated datasets.

| $N$  | Mean  | SD   |
|------|-------|------|
| 60   | 2.58  | 0.29 |
| 120  | 4.72  | 0.52 |
| 300  | 10.95 | 1.37 |
| 600  | 22.14 | 2.38 |
| 1200 | 44.42 | 4.34 |

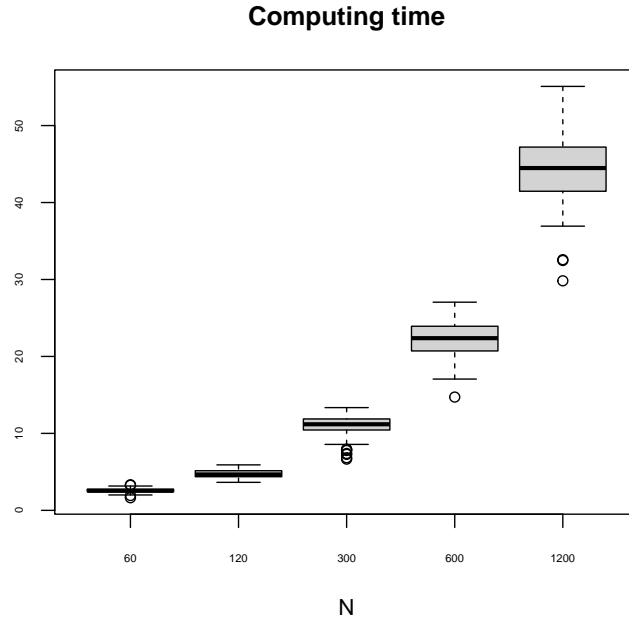

**Figure 49: Scenario 1:** Bar plot for the total computing times, in seconds, taken for the EM algorithm to converge across the simulated datasets. See also Table 92.

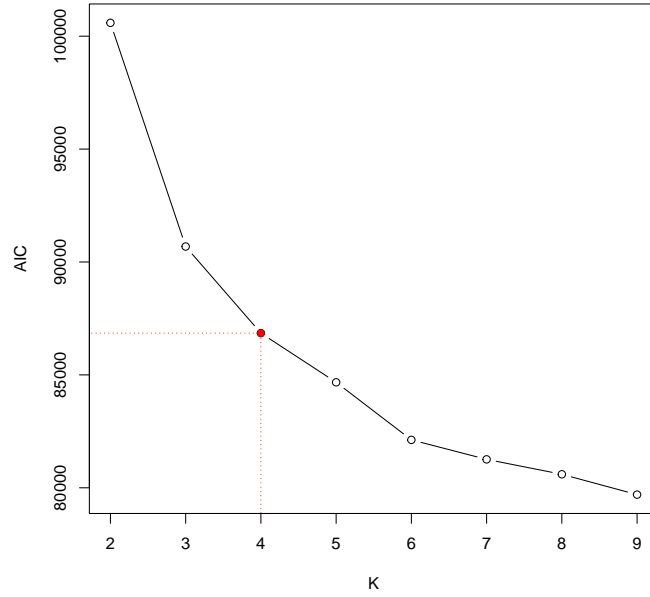

**Figure 50:** Plot of the best AIC for each  $K$  obtained from applying the EM algorithm under the simple ZIP model to the MESC dataset with random clustering initialization. Based on the elbow method, the optimal EM run corresponds to the point in red when  $K = 4$ .

## 2 Data analyses

### 2.1 Mouse Embryonic Stem Cell (MESC) data

**Table 93:** Confusion matrix between the EM clustering result when fitting the simple ZIP model to the MESC data and the experiment day labels. Inferred clusters are from the best EM algorithm run ( $K$ -means initialization and  $K = 4$ ) under the simple ZIP model (see Figure 51).

| Day | Inferred cluster |     |     |     |
|-----|------------------|-----|-----|-----|
|     | 1                | 2   | 3   | 4   |
| 0   | 218              | 64  | 396 | 255 |
| 4   | 0                | 676 | 0   | 7   |

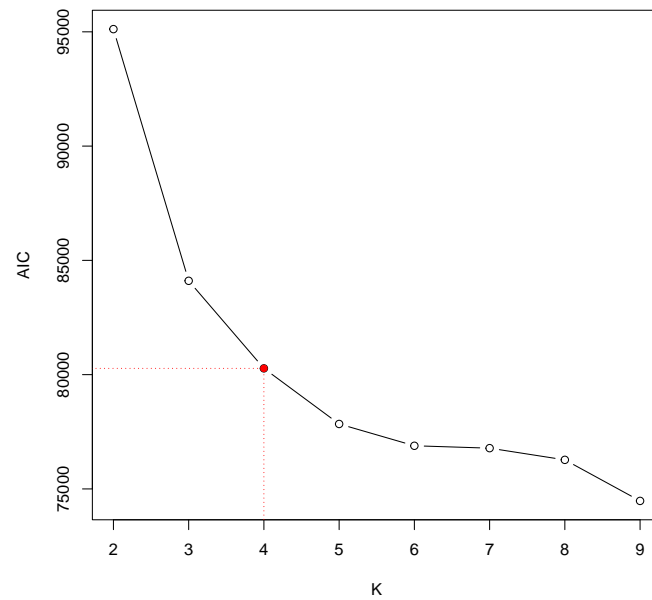

**Figure 51:** Plot of the best AIC for each  $K$  obtained from applying the EM algorithm under the simple ZIP model to the MESC dataset with  $K$ -means clustering initialization. Based on the elbow method, the optimal EM run corresponds to the point in red when  $K = 4$ .

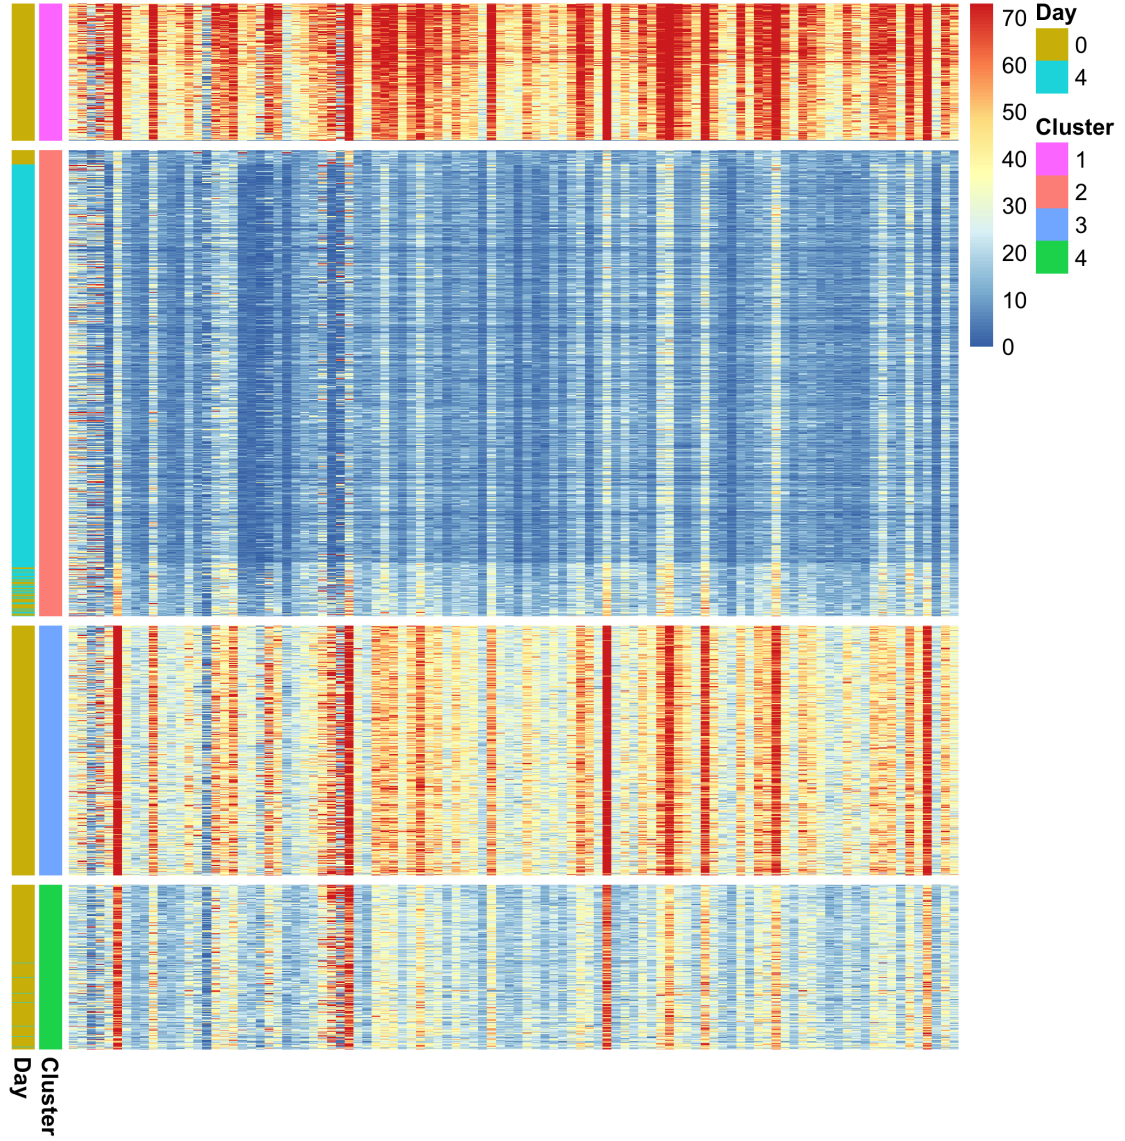

**Figure 52:** Heatmap of MESC data displaying read counts across all 1,616 cells (rows) and all 100 selected genes (columns). Cells (rows) are ordered by their inferred cluster assignments obtained from the best EM algorithm run ( $K$ -means initialization and  $K = 4$ ) under the simple ZIP model. The first column on the left shows the annotation for each cell's experiment day (0 or 4). Dark blue colours represent low read count values, and dark red colours represent high read count values. Note that to facilitate visualization under this colour scheme, read counts with values higher than the 95th percentile were truncated at the value of the 95th percentile.

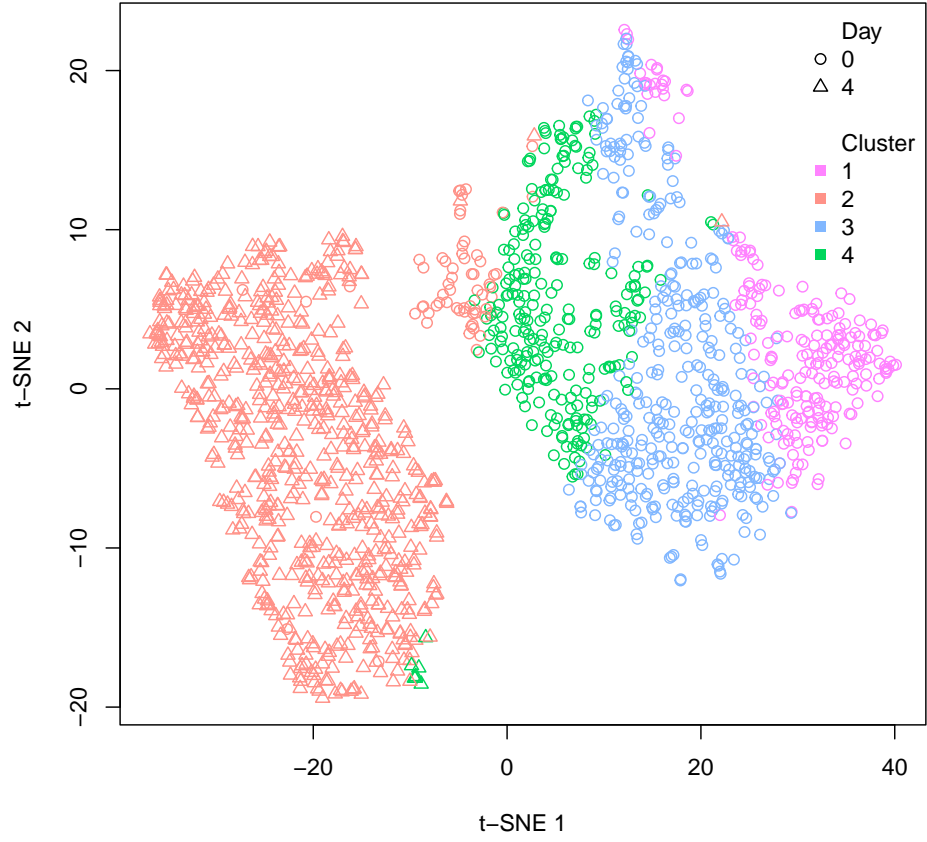

**Figure 53:**  $t$ -SNE plot for the MESC dataset and the clustering obtained from the best EM algorithm run ( $K$ -means initialization and  $K = 4$ ) under the simple ZIP model. Each point represents a cell with the shape symbol indicating the experiment day label (day 0 or day 4), and the colour the corresponding inferred cluster (1, 2, 3, or 4).

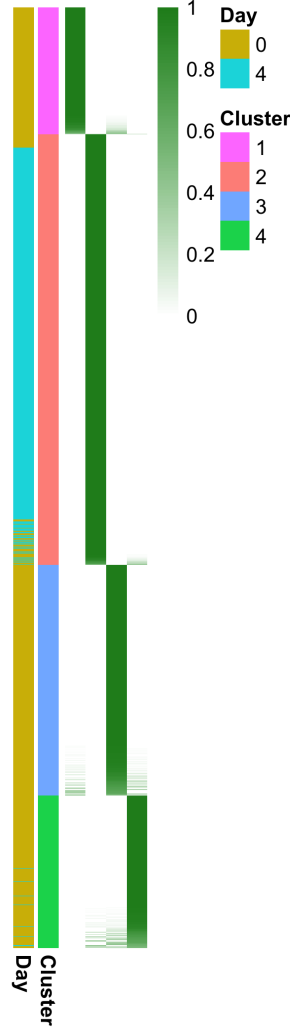

**Figure 54:** Heatmap of the  $\hat{Z}_{nk}$ 's for MESC dataset obtained from the best EM algorithm run ( $K$ -means initialization and  $K = 4$ ) under the simple ZIP model. Each row shows the estimated probability of a cell  $n$  belonging to each cluster  $k$  (columns). Rows are ordered by the final inferred cluster assignments determined by Eq. (??). The labels on the left show the assigned clusters and the day labels. Dark colours represent high probabilities.

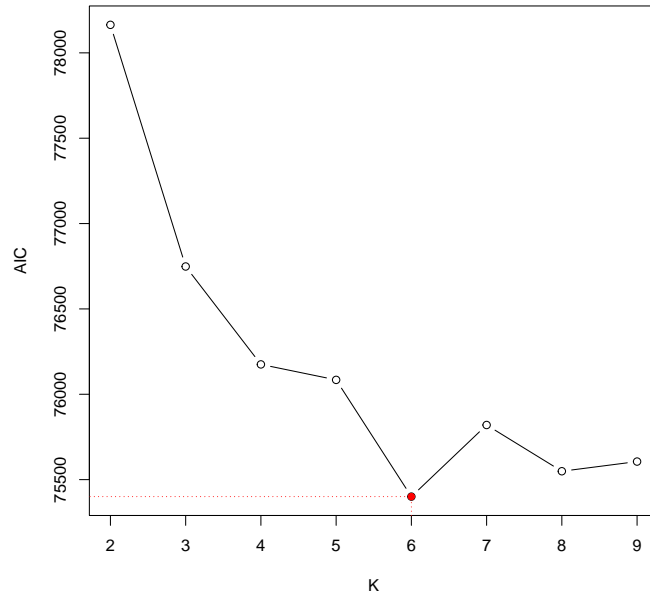

**Figure 55:** Plot of the best AIC for each  $K$  obtained from applying the EM algorithm under the ZIP mixture model with size factor to the MESC dataset with random clustering initialization. Based on the elbow method, the optimal EM run corresponds to the point in red when  $K = 6$ .

**Table 94:** Confusion matrix between the EM clustering result when fitting the ZIP mixture model with size factor to the MESC data and the experiment day labels. Inferred clusters are from the best EM algorithm run ( $K$ -means initialization and  $K = 4$ ) under the ZIP mixture model with size factor (see Figure 56).

| Day | Inferred cluster |   |    |     |
|-----|------------------|---|----|-----|
|     | 1                | 2 | 3  | 4   |
| 0   | 2                | 1 | 11 | 919 |
| 4   | 683              | 0 | 0  | 0   |

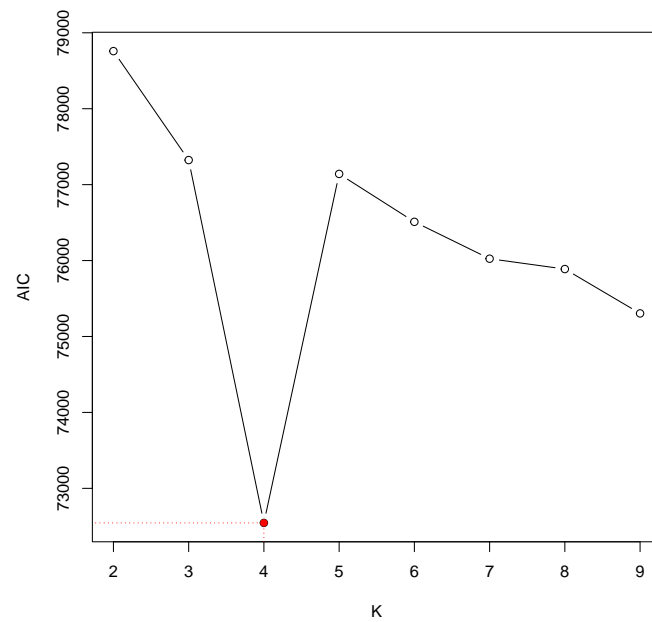

**Figure 56:** Plot of the best AIC for each  $K$  obtained from applying the EM algorithm under the ZIP mixture model with size factor to the MESC dataset with  $K$ -means clustering initialization. Based on the elbow method, the optimal EM run corresponds to the point in red when  $K = 4$ .

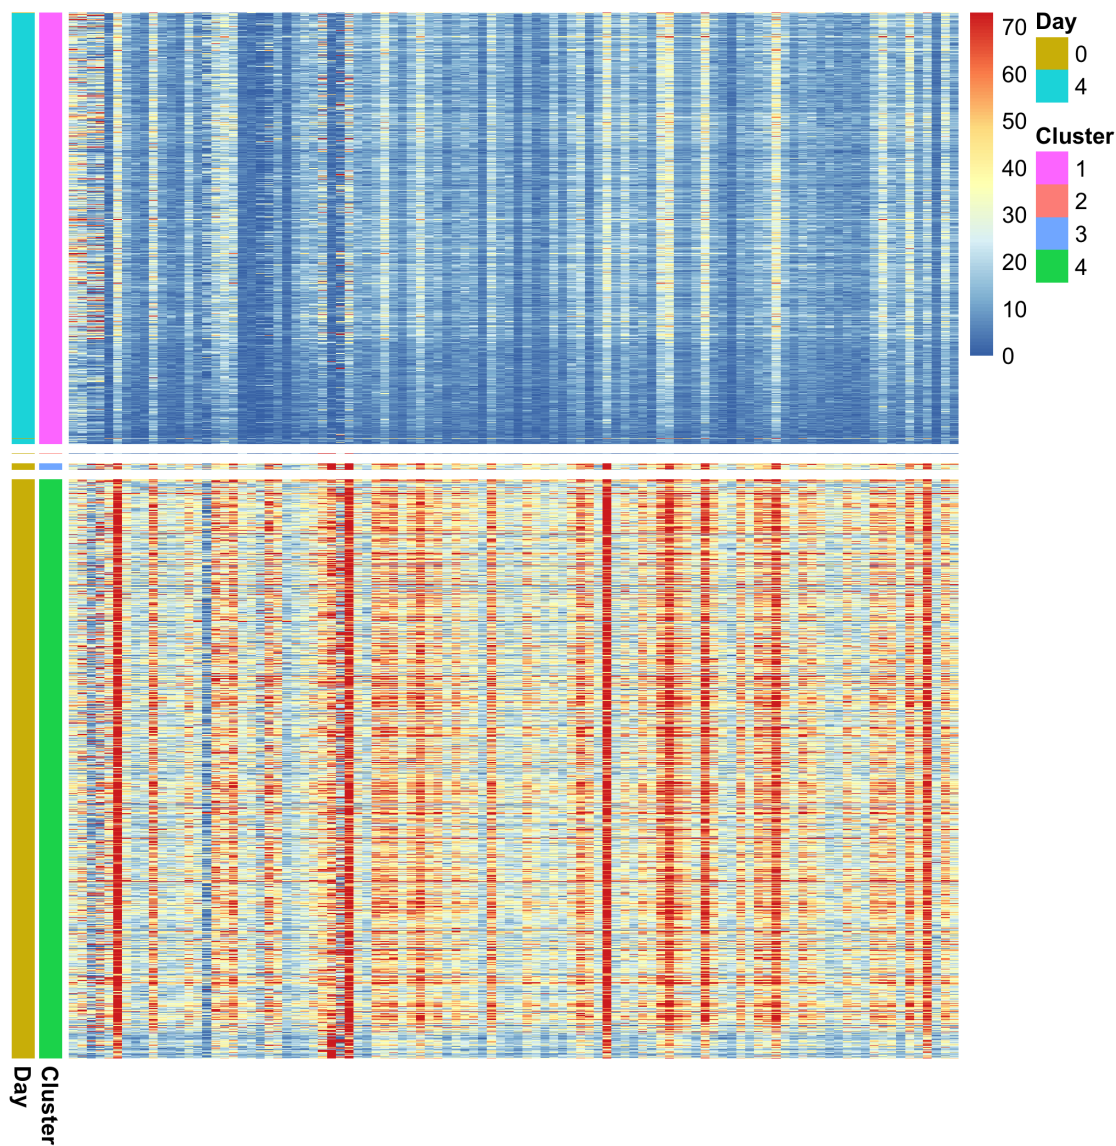

**Figure 57:** Heatmap of MESC data displaying read counts across all 1,616 cells (rows) and all 100 selected genes (columns). Cells (rows) are ordered by their inferred cluster assignments obtained from the best EM algorithm run ( $K$ -means initialization and  $K = 4$ ) under the ZIP mixture model with size factor. The first column on the left shows the annotation for each cell's experiment day (0 or 4). Dark blue colours represent low read count values, and dark red colours represent high read count values. Note that to facilitate visualization under this colour scheme, read counts with values higher than the 95th percentile were truncated at the value of the 95th percentile.

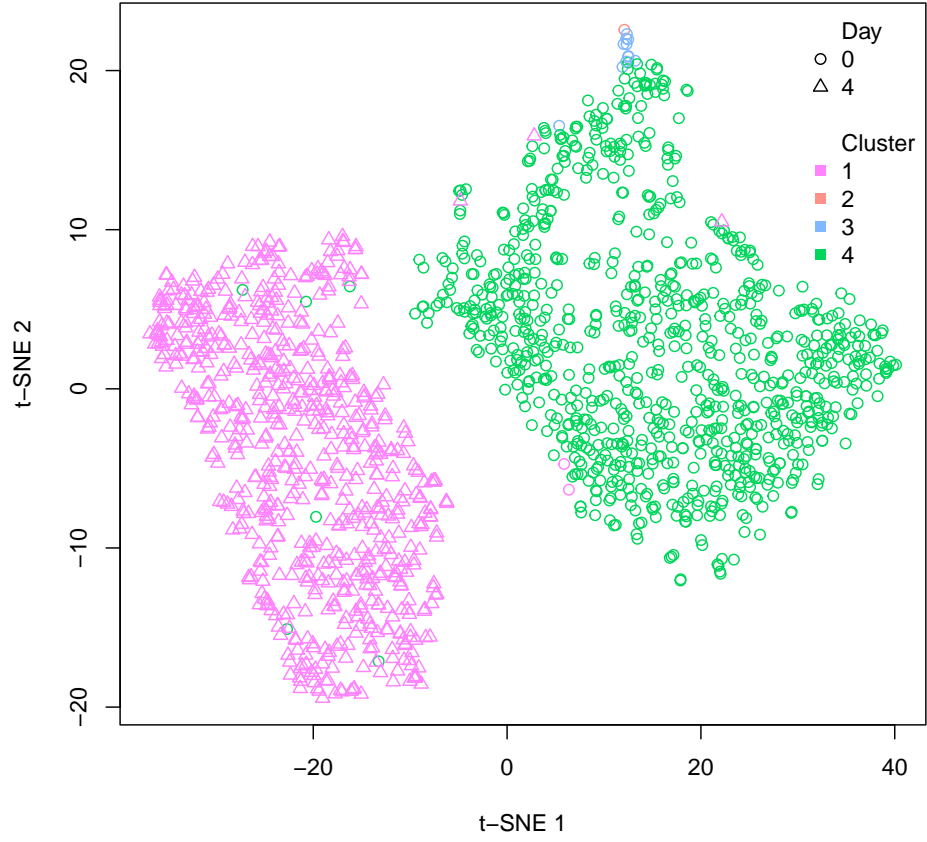

**Figure 58:**  $t$ -SNE plot for the MESC dataset and the clustering obtained from the best EM algorithm run ( $K$ -means initialization and  $K = 4$ ) under the ZIP mixture model with size factor. Each point represents a cell with the shape symbol indicating the experiment day label (day 0 or day 4), and the colour the corresponding inferred cluster (1, 2, 3, or 4).

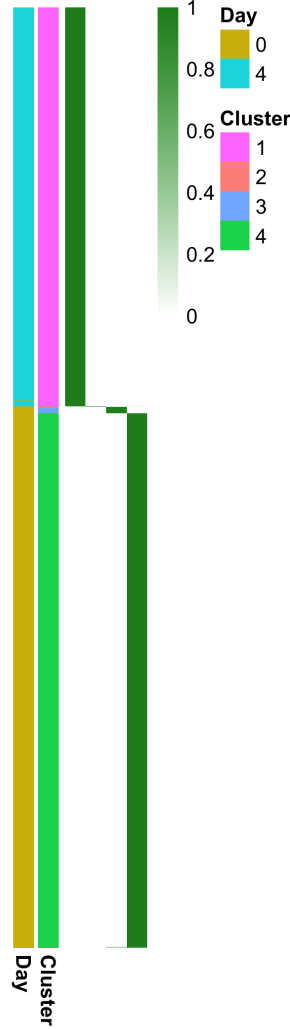

**Figure 59:** Heatmap of the  $\hat{Z}_{nk}$ 's for MESC dataset obtained from the best EM algorithm run ( $K$ -means initialization and  $K = 4$ ) under the ZIP mixture model with size factor. Each row shows the estimated probability of a cell  $n$  belonging to each cluster  $k$  (columns). Rows are ordered by the final inferred cluster assignments determined by Eq. (??). The labels on the left show the assigned clusters and the day labels. Dark colours represent high probabilities.

## 2.2 Liver Data

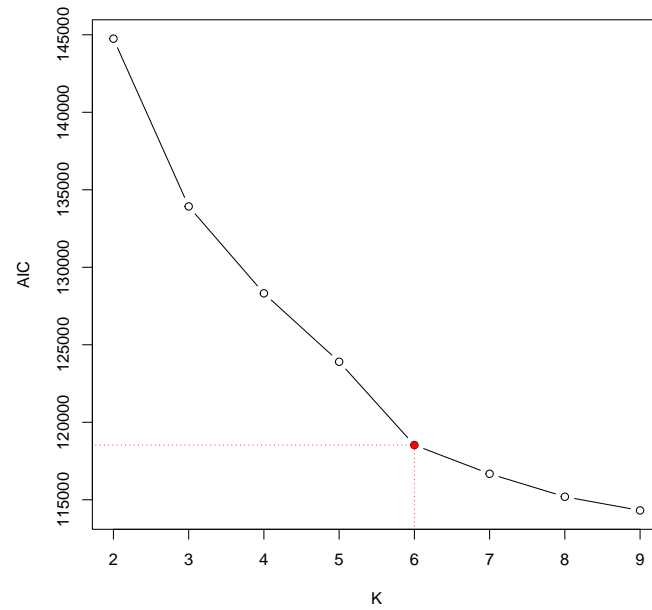

**Figure 60:** Plot of the best AIC for each  $K$  obtained from applying the EM algorithm under the simple ZIP model to the liver dataset with random clustering initialization. Based on the elbow method, the optimal EM run corresponds to the point in red when  $K = 6$ .

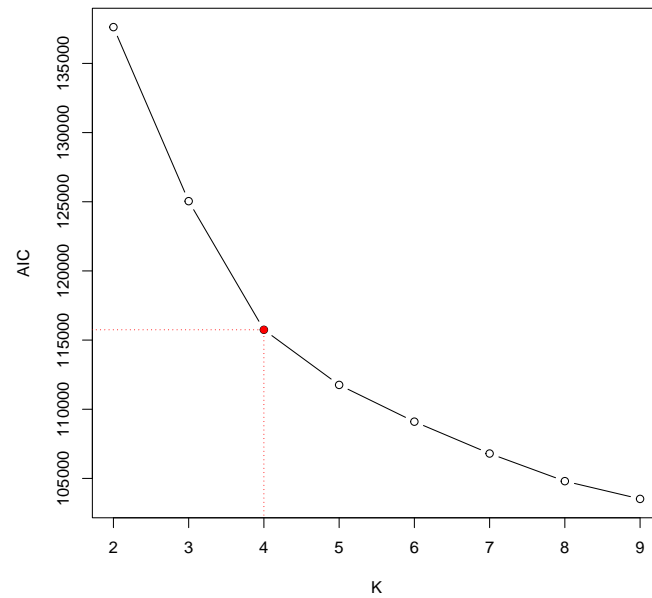

**Figure 61:** Plot of the best AIC for each  $K$  obtained from applying the EM algorithm under the simple ZIP model to the liver dataset with  $K$ -means clustering initialization. Based on the elbow method, the optimal EM run corresponds to the point in red when  $K = 4$ .

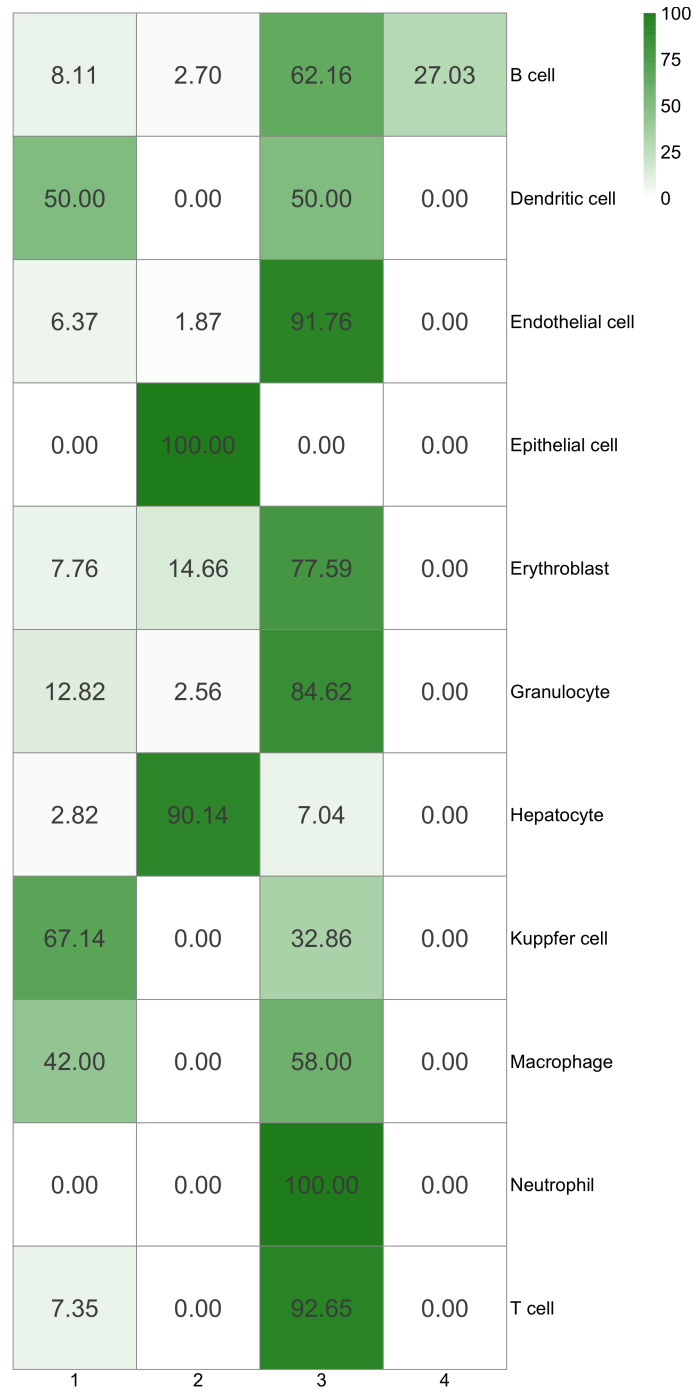

**Figure 62:** Liver dataset. Co-clustering between cell types (rows) and inferred clusters by the proposed EM algorithm (columns). Each entry  $a_{ij}$  represents the % of cells from type  $i$  that are present in the inferred cluster  $j$ . Rows sum up to 100%. Inferred clusters are from the best EM algorithm run ( $K$ -means initialization and  $K = 4$ ) under the simple ZIP model.

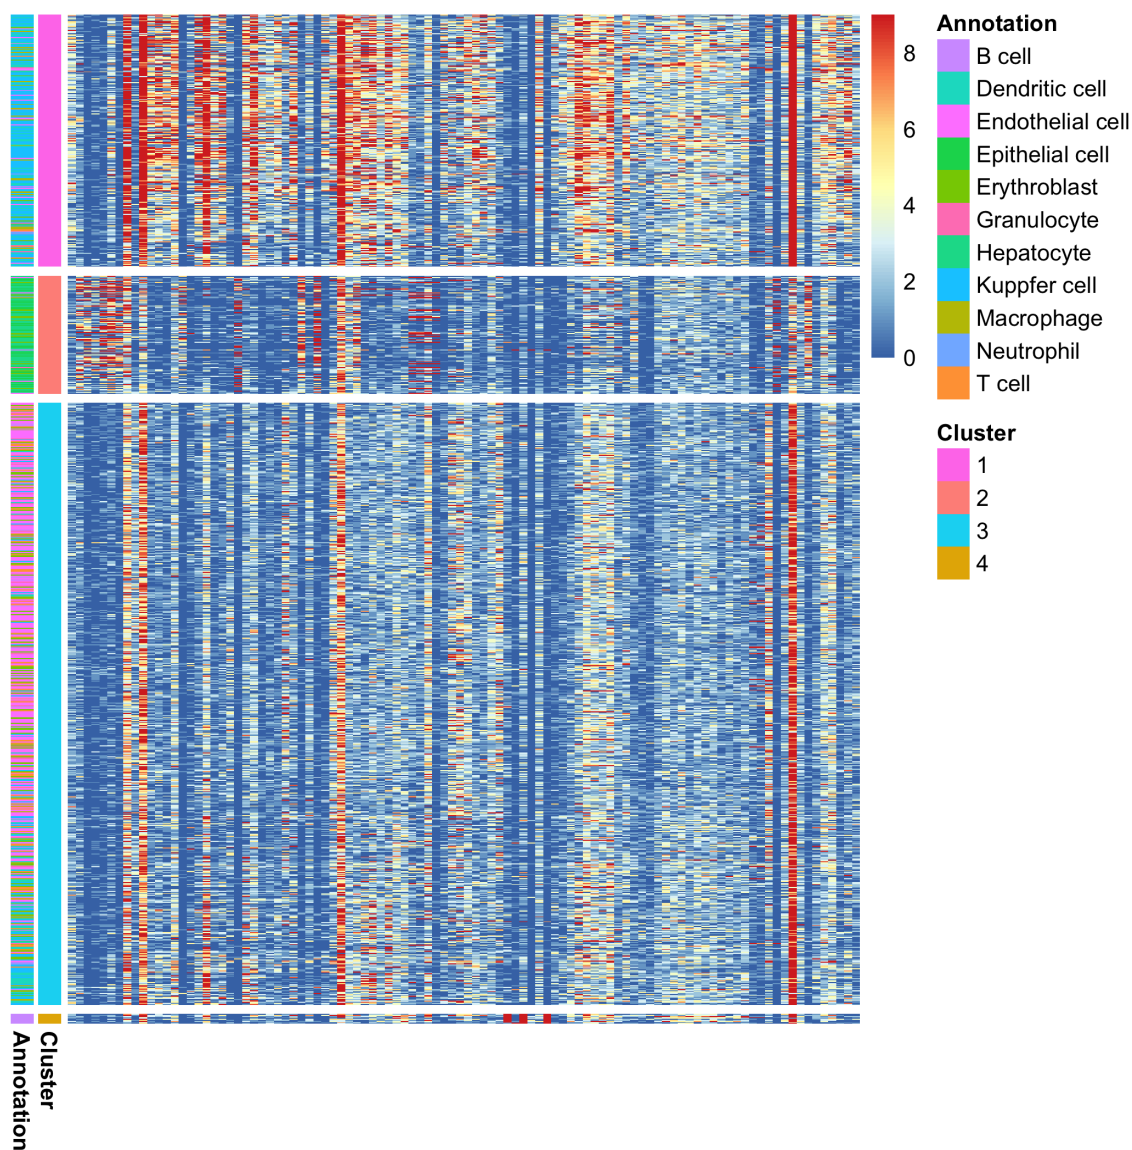

**Figure 63:** Heatmap of the liver data displaying read counts across all 1,000 randomly selected cells (rows) and all 100 selected genes (columns). Cells (rows) are ordered by their inferred cluster assignments obtained from the best EM algorithm run ( $K$ -means initialization and  $K = 4$ ) under the simple ZIP model. The first column on the left shows the annotation for each cell type. Dark blue colours represent low read count values, and dark red colours represent high read count values. Note that to facilitate visualization under this colour scheme, read counts with values higher than the 95th percentile were truncated at the value of the 95th percentile.

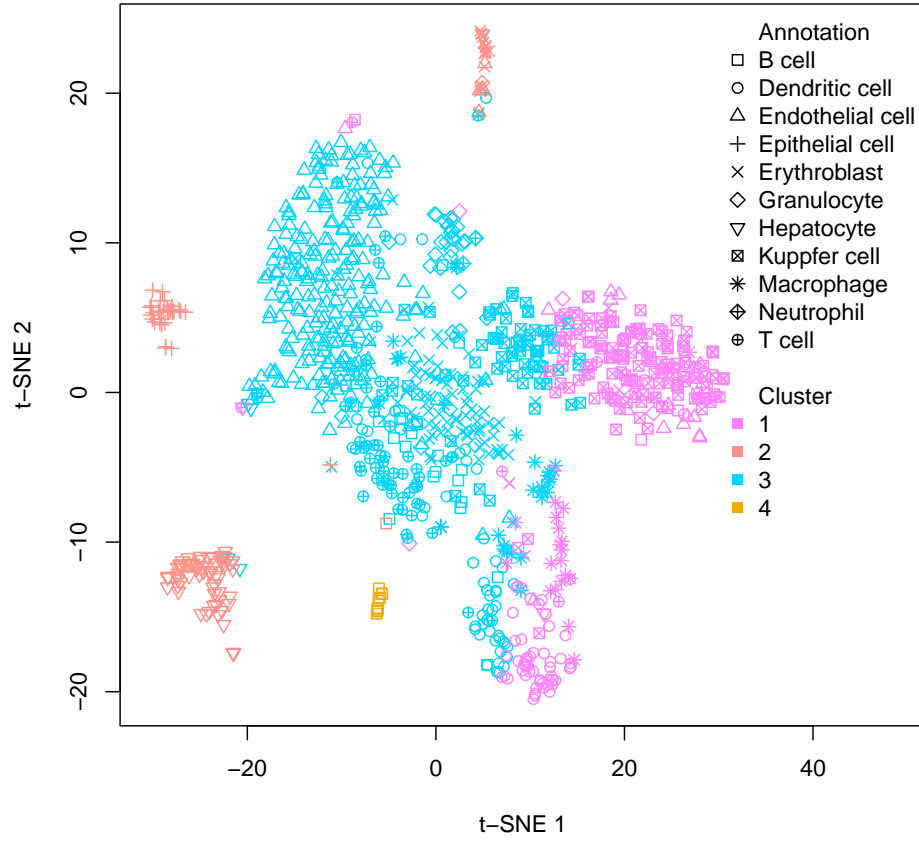

**Figure 64:**  $t$ -SNE plot for the liver dataset and the clustering obtained from the best EM algorithm run ( $K$ -means initialization and  $K = 4$ ) under the simple ZIP model. Each point represents a cell with the shape symbol indicating the cell type label, and the colour the corresponding inferred cluster (1, 2, 3, or 4).

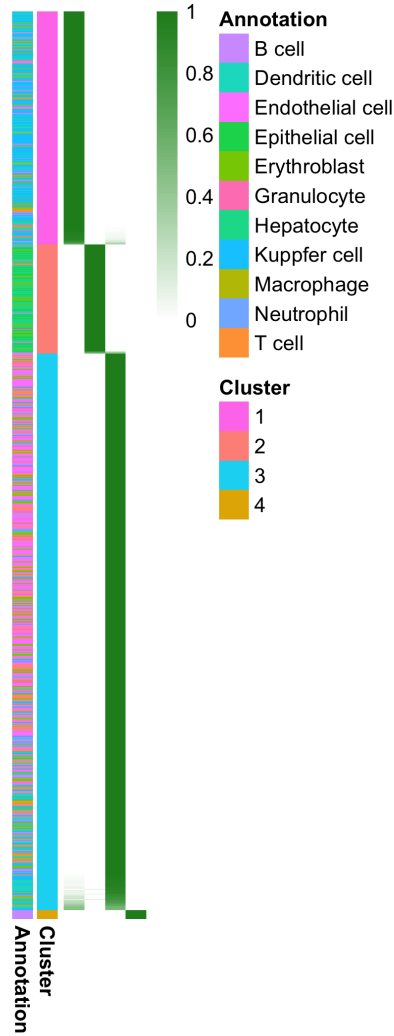

**Figure 65:** Heatmap of the  $\hat{Z}_{nk}$ 's for the liver dataset obtained from the best EM algorithm run ( $K$ -means initialization and  $K = 4$ ) under the simple ZIP model. Each row shows the estimated probability of a cell  $n$  belonging to each cluster  $k$  (columns). Rows are ordered by the final inferred cluster assignments. The labels on the left show the assigned clusters and the cell type labels. Dark colours represent high probabilities.

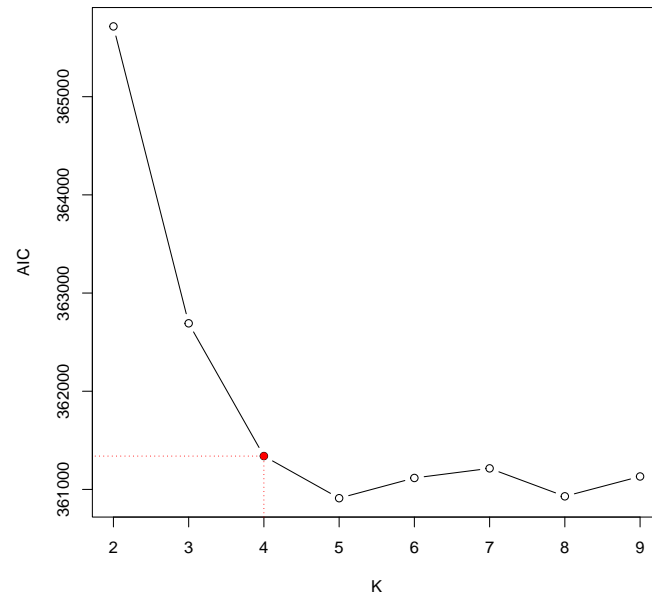

**Figure 66:** Plot of the best AIC for each  $K$  obtained from applying the EM algorithm under the simple ZINB model to the liver dataset with random clustering initialization. Based on the elbow method, the optimal EM run corresponds to the point in red when  $K = 4$ .

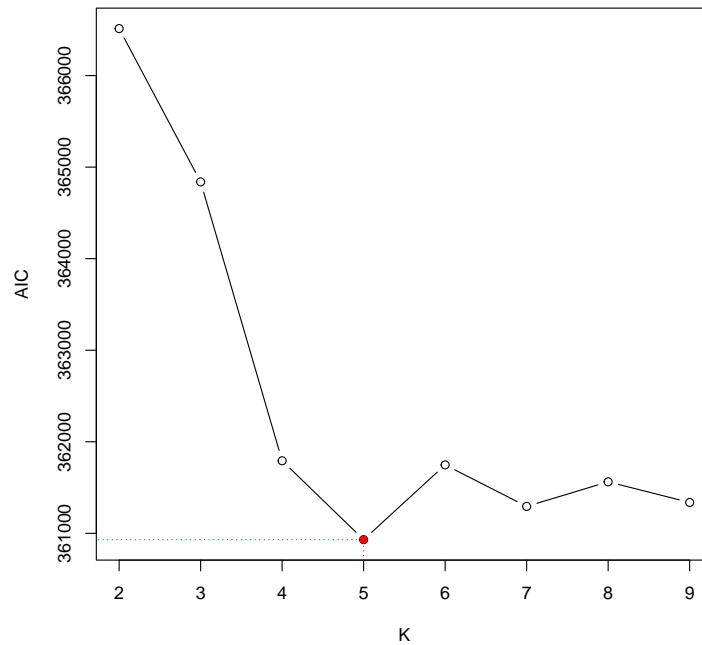

**Figure 67:** Plot of the best AIC for each  $K$  obtained from applying the EM algorithm under the simple ZINB model to the liver dataset with  $K$ -means clustering initialization. Based on the elbow method, the optimal EM run corresponds to the point in red when  $K = 5$ .

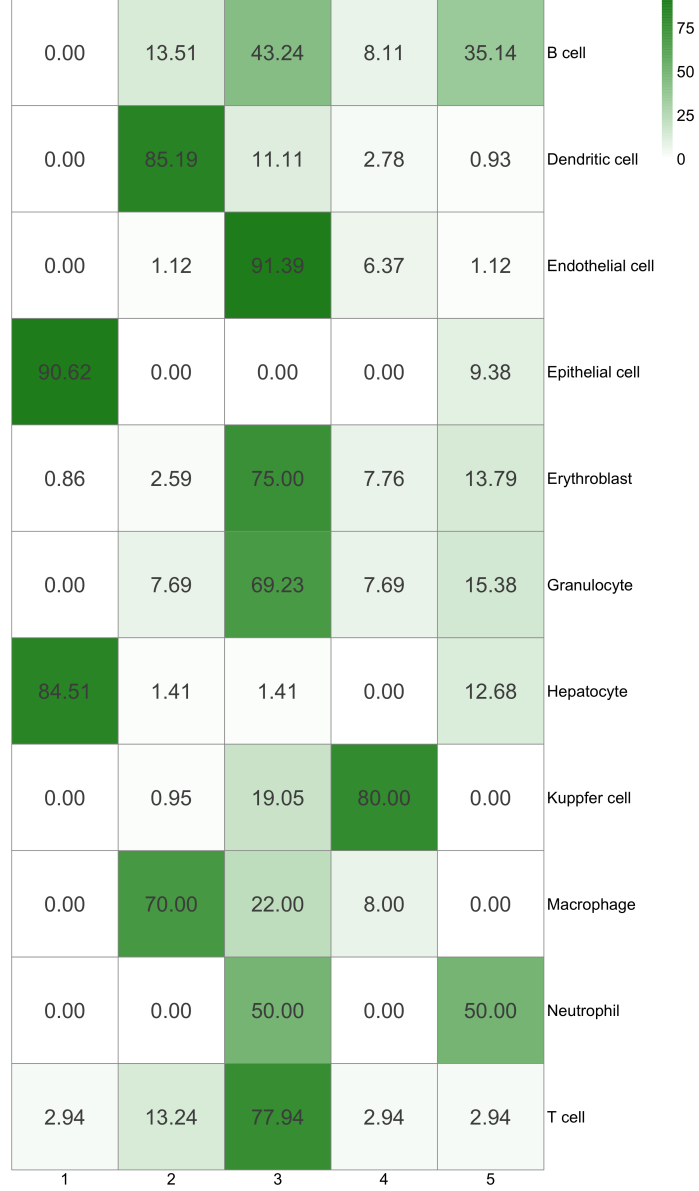

**Figure 68:** Liver dataset. Co-clustering between cell types (rows) and inferred clusters by the proposed EM algorithm (1, 2, 3, 4, and 5; columns). Each entry  $a_{ij}$  represents the % of cells from type  $i$  that are present in the inferred cluster  $j$ . Rows sum up to 100%. Inferred clusters are from the best EM algorithm run ( $K$ -means initialization and  $K = 5$ ) under the simple ZINB model.

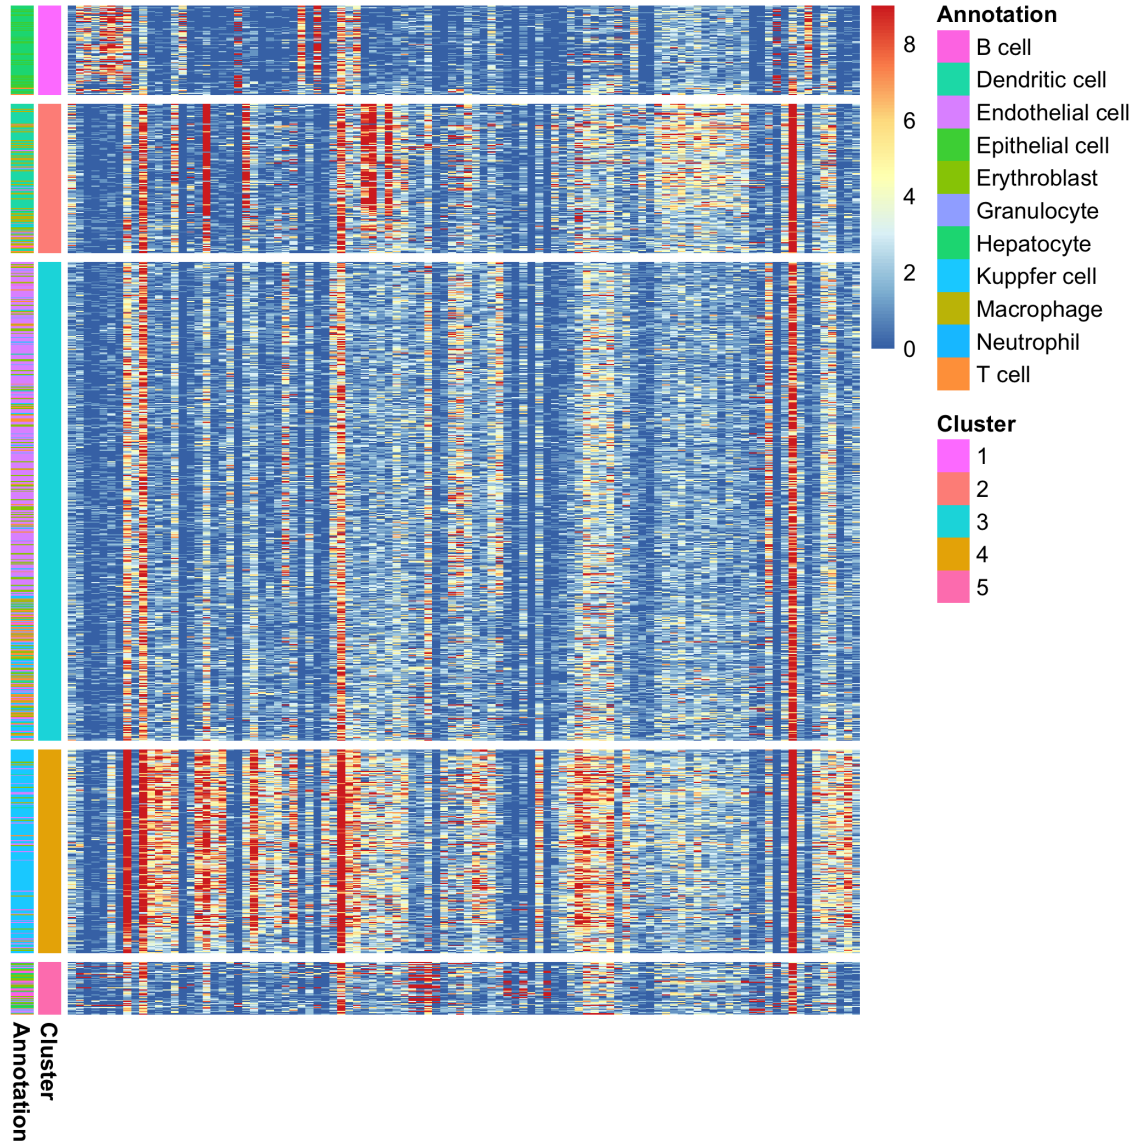

**Figure 69:** Heatmap of the liver data displaying read counts across all 1,000 randomly selected cells (rows) and all 100 selected genes (columns). Cells (rows) are ordered by their inferred cluster assignments obtained from the best EM algorithm run ( $K$ -means initialization and  $K = 5$ ) under the simple ZINB model. The first column on the left shows the annotation for each cell type. Dark blue colours represent low read count values, and dark red colours represent high read count values. Note that to facilitate visualization under this colour scheme, read counts with values higher than the 95th percentile were truncated at the value of the 95th percentile.

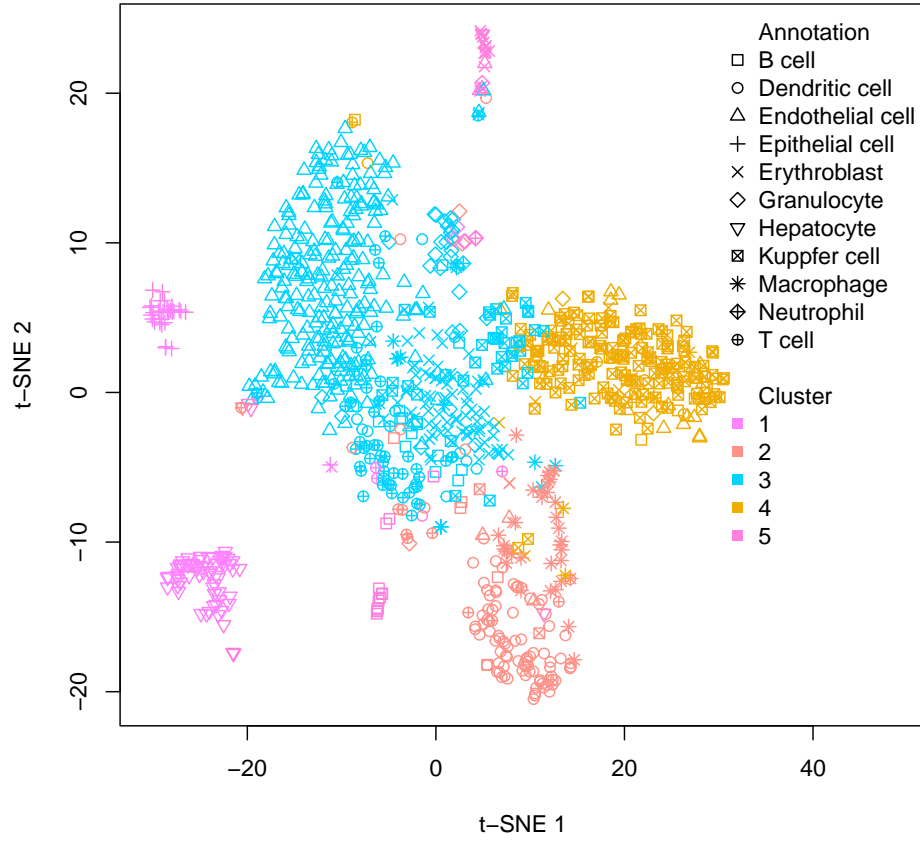

**Figure 70:**  $t$ -SNE plot for the liver dataset and the clustering obtained from the best EM algorithm run ( $K$ -means initialization and  $K = 5$ ) under the simple ZINB model. Each point represents a cell with the shape symbol indicating the cell type label, and the colour the corresponding inferred cluster (1, 2, 3, 4, or 5).

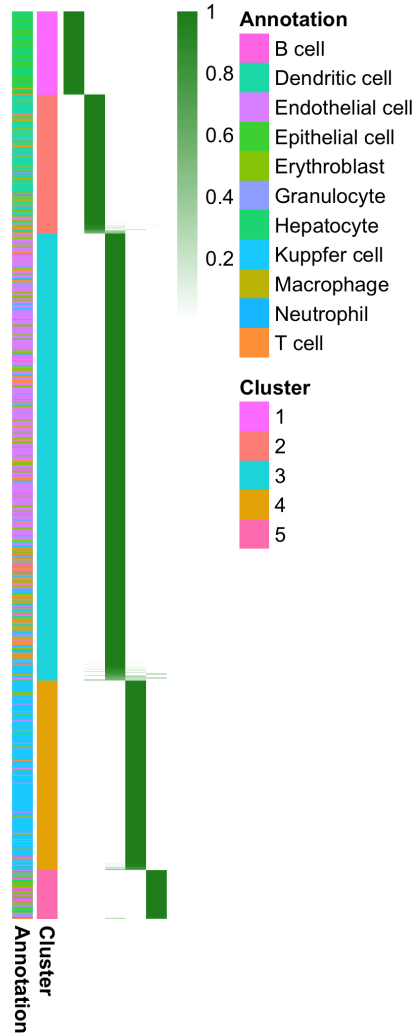

**Figure 71:** Heatmap of the  $\hat{Z}_{nk}$ 's for the liver dataset obtained from the best EM algorithm run ( $K$ -means initialization and  $K = 5$ ) under the simple ZINB model. Each row shows the estimated probability of a cell  $n$  belonging to each cluster  $k$  (columns). Rows are ordered by the final inferred cluster assignments. The labels on the left show the assigned clusters and the cell type labels. Dark colours represent high probabilities.

## Bibliography

- L. Hi, H. Sieling, and T. Aspelmeier. FDRSeg: FDR-control in multiscale change-point segmentation. *R package version 1.0-3*, 2017. → pages 3
- A. Rosenberg and J. Hirschberg. V-measure: A conditional entropy-based external cluster evaluation measure. *Proceedings of the 2007 Joint Conference on Empirical Methods in Natural Language Processing and Computational Natural Language Learning*, pages 410–420, 2007. → pages 3
